# Supplementary material for: Inference for Heterogeneous Graphical Models using Doubly High-Dimensional Linear-Mixed Models
Source: arXiv:2403.10034 source file (2026-10-09)
Supplement: Supplementary file 1 [file supp.tex]

\documentclass{article}
\usepackage[utf8]{inputenc}

\title{Supplement: Inference for Heterogeneous Graphical Models using Doubly High-Dimensional Linear-Mixed Models}
\author{}
\date{}
\setlength\parindent{8pt}
\usepackage{natbib}
\usepackage{graphicx}
\usepackage{amsmath, amssymb, color}
\usepackage{amsthm, bm}
\usepackage{setspace}
\usepackage{url}
\usepackage{float}
\usepackage{fullpage}
\usepackage{booktabs, multirow,ltablex}
\usepackage{lscape}

\doublespacing

\newtheorem{theorem}{Theorem}[section]
\newtheorem*{theorem*}{Theorem}

\newtheorem*{corollary*}{Corollary}
\newtheorem{lemma}[theorem]{Lemma}
\newtheorem*{lemma*}{Lemma}
\newtheorem{assumption}{Assumption}
\newtheorem*{assumption*}{Assumption}
\theoremstyle{definition}

\theoremstyle{remark}
\newtheorem{remark}{Remark}[section]

\def\diag{\mathop{\mathrm{diag}}}
\def\Tr{\mathop{\mathrm{tr}}}
\def\tr{\mathop{\mathrm{tr}}}
\def\SE{\mathop{\mathrm{SE}}}
\def\SG{\mathop{\mathrm{SG}}}
\def\N{\mathop{\mathrm{N}}}
\def\E{\mathop{\mathbb{E}}}
\def\R{\mathop{\mathbb{R}}}
\def\P{\mathop{\mathbb{P}}}
\def\qm{\mathop{\mathbf{1}\{q>c_0m\}}}
\def\SGV{\mathop{\mathrm{SGV}}}
\def\vec{\mathop{\mathrm{vec}}}
\def\Var{\mathop{\mathrm{Var}}}

\renewcommand{\theenumi}{\arabic{enumi}}
\renewcommand{\theenumii}{\arabic{enumii}}

\makeatletter
\renewcommand{\p@enumii}{\theenumi.}
\renewcommand{\p@enumiii}{\theenumi.\theenumii.}
\makeatother

%%% HELPER CODE FOR DEALING WITH EXTERNAL REFERENCES
\usepackage{xr}
\makeatletter
\newcommand*{\addFileDependency}[1]{
  \typeout{(#1)}
  \@addtofilelist{#1}
  \IfFileExists{#1}{}{\typeout{No file #1.}}
}
\makeatother

%%% END HELPER CODE

% \myexternaldocument{main}

\makeatletter
\renewcommand \thesection{S\@arabic\c@section}
\renewcommand\thetable{S\@arabic\c@table}
\renewcommand \thefigure{S\@arabic\c@figure}
\renewcommand \theequation{S\@arabic\c@equation}
\makeatother

\begin{document}
\maketitle

This document collects the proofs for Lemmas and Theorems in the main paper.

\section{Fixed Effect Estimator $\hat\beta$}
\label{S:A}

\begin{assumption}
\label{as.A}
\begin{enumerate}
    \item \label{as.A.1} Let $q>c_0m$ or $m>c_0q$ for some constant $c_0>1$ and let $m \vee q > c_1$ for some suitably large constant $c_1>0$. Moreover, let $\log(q) \left(q/m\right)^{\qm}/n = o(1)$.
    \item \label{as.A.2} $\forall \ i$, $\sigma(\Sigma_X) \asymp \sigma(R^i) \asymp \|\Psi \|_2 \asymp 1$, $\|\Sigma_X^i - \Sigma_X\|_2 \leq  \sigma_{\min}(\Sigma_X) - c_2$, for some constant $c_2 >0$. 
    % \item \label{as.A.4} 
    % \begin{align*}
    %     \begin{cases}
    %     \frac{s^2q\log(p)}{mn} =o(1) &, \text{ when } q>c_0m\\
    %     \frac{s^2 \log^2(n)\log(p)}{n} =o(1) &, \text{ when } q>c_0m \text{ and Assumption \ref{as.A.add}.\ref{as.A.3} holds}\\
    %     \frac{s^2\log(p)}{n} =o(1) &, \text{ when } m>c_0q \text{ and } p=q\\
    %     \frac{s^2m\log(p)}{n} =o(1) &, \text{ when } m>c_0q \text{ and } p>q
    %     \end{cases}
    % \end{align*}
\end{enumerate}
\end{assumption}

\begin{assumption}
\label{as.A.add}
\begin{enumerate}
    \item \label{as.A.3} $\Psi = \diag(\psi)$ for a vector $\psi \in \R^q$. The support of $\psi$ is $S_\psi$ with cardinality $s_\psi < c_2m \wedge n$ for some constant $c_2>0$, and $\min(\psi_{S_\psi}) \asymp \max(\psi_{S_\psi}) \asymp 1$.
    \item \label{as.A.3.2} $\sigma_{\min}(\Psi) \asymp 1$.
\end{enumerate}

\end{assumption}

\begin{theorem}[Fixed effect estimator consistency]
\label{thm:S1}
Under Assumption \ref{as.A}.\ref{as.A.1} and Assumption \ref{as.A}.\ref{as.A.2}, with probability at least $1-4\exp\{-cn\} -12\exp\{-c\log(n)\} - 2\exp\{-cmnq^{-\qm}\} - \exp\{-cn(m/q)^{\qm}\}$, we have the following results:
\begin{enumerate}
    \item When $q>c_0m$: Taking $\lambda_a = c_1\sqrt{q\log(p)/(nm)}$ for a suitably large $c_1>0$, we have that:
     \begin{align*}
         &\|\hat \beta -\beta^*\|_2 = O_p\left(\sqrt{\frac{sq\log(p)}{mn}}\right),\\
         &\|\hat \beta -\beta^*\|_1 = O_p\left(s\sqrt{\frac{q\log(p)}{mn}}\right),\\
         & \left\|\Sigma_a^{-1/2} X (\hat \beta -\beta^*)\right\|_2^2 = O_p\left(s\log(p)\right).
     \end{align*}
     
     \item  When $q>c_0m$ and Assumption~\ref{as.A.add}.\ref{as.A.3} also holds:
    Taking $\lambda_a = c_2\sqrt{\log(p)\log^2(n)/n}$ for suitably large $c_2>0$, we have that:
     \begin{align*}
         &\|\hat \beta -\beta^*\|_2 = O_p\left(\sqrt{\frac{s\log^2(n)\log(p)}{n}}\right),\\
         &\|\hat \beta -\beta^*\|_1 = O_p\left(s\sqrt{\frac{\log^2(n)\log(p)}{n}}\right),\\
         &\|\Sigma_a^{-1/2} X (\hat \beta -\beta^*)\|_2^2 = O_p\left(\frac{sm\log^2(n)\log(p)}{q}\right).
     \end{align*}
     
     \item When $m>c_0q$ and $p=q$:
    Taking $\lambda_a = c_3\sqrt{\log(p)/(nm^2)}$ for suitably large $c_3>0$, we have that:
     \begin{align*}
         &\|\hat \beta -\beta^*\|_2 = O_p\left(\sqrt{\frac{s\log(p)}{n}}\right),\\
         &\|\hat \beta -\beta^*\|_1 = O_p\left(s\sqrt{\frac{\log(p)}{n}}\right),\\
         &\|\Sigma_a^{-1/2} X (\hat \beta -\beta^*)\|_2^2 = O_p\left(s\log(p)\right).
     \end{align*}
     
    \item When $m>c_0q$ and $p>q$:
    Taking $\lambda_a = c_4\sqrt{{\log(p)}/{(nm)}}$ for suitably large $c_4>0$, we have that:
     \begin{align*}
         &\|\hat \beta -\beta^*\|_2 = O_p\left(\sqrt{\frac{sm\log(p)}{n}}\right),\\
         &\|\hat \beta -\beta^*\|_1 = O_p\left(s\sqrt{\frac{m\log(p)}{n}}\right),\\
         &\|\Sigma_a^{-1/2} X (\hat \beta -\beta^*)\|_2^2 = O_p\left(sm\log(p)\right).
     \end{align*}
    
\end{enumerate}
% Under Assumption \ref{as.A}.\ref{as.A.4}, $\hat\beta_j$ consistently estimates $\beta_j^*$ under $\ell_1$-norm and $\ell_2$-norm.
\end{theorem}

\subsection{Related lemmas for Theorem \ref{thm:S1}}

%lemmaA.1
\begin{lemma}[Core Lemma]
\label{lemma:A.1}
Assume $q>c_0m$ or $m > c_0q$ for some constant $c_0>1$. $Z$ is a $m \times q$ matrix with entries independently following the $N(0, 1)$ distribution, and $Z^i$, $i=1, \dots, n$ are identical copies of $Z$. Then the following properties hold for the non-zero singular values $\sigma(Z)$ of $Z$ and $\sigma(Z^i)$ of $Z^i$'s:
\begin{enumerate}
    \item \label{lemma:A.1(1)}
    $|\sqrt{q} - \sqrt{m}| \leq \E(\sigma(Z)) \leq \sqrt{m} + \sqrt{q}$, $\E(\sigma(Z)) \asymp \sqrt{m} \vee \sqrt{q}$.
    \item \label{lemma:A.1(2)}
    $\sigma(Z) - \E(\sigma(Z)) \in \SG(1)$. 
    \item \label{lemma:A.1(3)}
    $\E(\sigma^2(Z)) \in [\E(\sigma(Z))^2, \E(\sigma(Z))^2+1]$, $\E(\sigma^2(Z)) \asymp m \vee q$.
    \item \label{lemma:A.1(4)}
    $\sigma^2(Z) - \E(\sigma^2(Z)) \in \SE(32, 4)$. $\sum_{i=1}^n \sigma^2(Z^i) \asymp n(m \vee q)$ with probability at least $1-2\exp\{-c_1n(m\vee q)\}$, for some $c_1>0$.
    \end{enumerate}
    Further assume $m \vee q > c_2 >0$ for some suitably large constant $c_2$. Denote $\Sigma_a^i = aZ^i(Z^i)^\top + I_m$, where $a$ is a positive constant. Then we have the following properties hold for any constant $c>0$, for positive constants $c_3, c_4, \dots$:
    \begin{enumerate}
    \setcounter{enumi}{4}
    \item \label{lemma:A.1(5)}
        $\frac{1}{\E(\sigma^2(Z)) + c} \leq \E\left( \frac{1}{\sigma^2(Z) +c}\right) \leq \frac{4}{\E(\sigma^2(Z))+c}$.
    \item  \label{lemma:A.1(6.1)}
    $ \frac{1}{\sigma^2(Z) +c} - \E\left( \frac{1}{\sigma^2(Z) +c}\right) \in \SE\left(c_3 \E\left( \frac{1}{\sigma^2(Z) +c}\right)^2, c_3 \E\left( \frac{1}{\sigma^2(Z) +c}\right)\right)$.
    \item \label{lemma:A.1(6.2)}\label{lemma:A.1(6.3)} \label{lemma:A.1(6.4)}
    $\sum_{i=1}^n  \frac{1}{\sigma^2(Z^i) +c} \asymp \frac{n}{m\vee q}$ with probability at least $1-2\exp\{-c_4n\}$. $\max_{1 \leq i \leq n} \frac{1}{\sigma^2(Z^i) +c} \leq \frac{1}{c} \wedge \frac{c_5\log(n)}{m \vee q}$ with probability at least $1-2\exp\{-c_6\log(n)\}$, $\min_{1 \leq i \leq n} \frac{1}{\sigma^2(Z^i) +c} \geq \frac{c_7}{\log(n) + m \vee q}$ with probability at least $1-2\exp\{-c_6\log(n)\}$.
    \item \label{lemma:A.1(6.5)}
    $\sum_{i=1}^n \Tr\left((\Sigma_a^i)^{-1}\right) \asymp mnq^{-\qm}$ with probability at least $1-4\exp\{-c_8n\}$.\\
    When $q>c_0m$: $ \frac{c_9m}{\log(n) + q} \leq \min_i\Tr\left((\Sigma_a^i)^{-1}\right) \leq \max_i\Tr\left((\Sigma_a^i)^{-1}\right) \leq c_{10} m \left(1 \wedge \frac{\log(n)}{q}\right)$ with probability at least $1-4\exp\{-c_{11}\log(n)\}$.\\
    When $m>c_0q$: $c_{12} \left(m + \frac{q}{m + \log(n)}\right)\leq \min_i\Tr\left((\Sigma_a^i)^{-1}\right) \leq \max_i\Tr\left((\Sigma_a^i)^{-1}\right) \leq c_{13} \left(m + q\left(1 \wedge \frac{\log(n)}{m}\right) \right)$ with probability at least $1-4\exp\{-c_{14}\log(n)\}$.
    % \item \label{lemma:A.1(7)} \textcolor{blue}{maybe not need}
    %     $ \frac{1}{(\E(\sigma^2(Z))+c)^2+c_{15}} \leq \E\left(\frac{1}{(\sigma^2(Z) +c)^2}\right) \leq \frac{k}{(\E(\sigma^2(Z)) +c)^2}$, for constant $k>4$.
    \item \label{lemma:A.1(8)}
         $\E\left(Z^\top (aZZ^\top +I_m)^{-1}Z\right) = k I_q$, $k \asymp \left({m}/{q}\right)^{\qm}$.
$\sigma\left(\sum_{i=1}^n (Z^i)^\top (\Sigma_a^i)^{-1} Z^i\right) \asymp n \left({m}/{q} \right)^{\qm}$ with probability at least $1-\exp\left\{\log(q) - c_{16}n\left({m}/{q}\right)^{\qm}\right\}$.
    \item \label{lemma:A.1(9)} Assume ${\log(q)}\left(q/m\right)^{\qm}/n = o(1)$. %Based on Lemma \ref{lemma:A.1(8)}, Lemma \ref{lemma:A.1(6.3)}
    Then with probability at least $1-2\exp\{-c_{18}n\} - 2\exp\{-c_{18}\log(n)\} - \exp\left\{-c_{18}n\left(m/q\right)^{\qm}\right\}$: 
    \begin{align*}
        & \sigma\left( \sum_{i=1}^n (Z^i)^\top (\Sigma_a^i)^{-2} Z^i \right) \leq
        \begin{cases}
            c_{17} \frac{n}{q}\left( 1 \wedge \frac{m\log(n)}{q}\right)& , q>c_0m, \\
            c_{17} \frac{n}{m}& , m>c_0q.
        \end{cases}
    \end{align*}
\end{enumerate}
\end{lemma}

%lemmaA.3
\begin{lemma}
\label{lemma:A.3}
\begin{enumerate}
    \item \label{lemma:A.3.1} Under Assumption \ref{as.A}.\ref{as.A.1} and Assumption \ref{as.A}.\ref{as.A.2}, with probability at least $1-4\exp\{-cn\} -2\exp\{-c\log(n)\} - 2\exp\{-cmnq^{-\qm}\} -\exp\left\{-cn\left(m/q\right)^{\qm} \right\}$, we have:
    \begin{align*}
        \begin{cases}
            \sigma(X^\top \Sigma_a^{-1} X) \asymp \frac{mn}{q} &, q>c_0m,\\
            \sigma(X^\top \Sigma_a^{-1} X) \asymp n &, m>c_0q \text{ and } p=q,\\
            c_1n \leq \sigma(X^\top \Sigma_a^{-1} X) \leq  c_2mn &, m>c_0q \text{ and } q<p.
        \end{cases}
    \end{align*}
    \item \label{lemma:A.3.2}  Under Assumption \ref{as.A}.\ref{as.A.1} and Assumption \ref{as.A}.\ref{as.A.2}, $\max_i\sigma((X^i)^\top (\Sigma^i_a)^{-1} X^i) \leq c_1$ when $p=q$; when $p>q$, with probability at least $1-8\exp\{-c_2\log(n)\}$ we have:
    \begin{align*}
        \max_i\sigma((X^i)^\top (\Sigma^i_a)^{-1} X^i) \leq \begin{cases}
            c_3 \left(1 \vee \frac{m\log^2(n)}{q}\right) &, q>c_0m,\\
            c_3 m \log^2(n) &, m>c_0q.
        \end{cases}
    \end{align*}
\end{enumerate}
\end{lemma}

%lemmaA.2
\begin{lemma}
\label{lemma:A.2}
\begin{enumerate}
    % lemmaA.2.1
    \item \label{lemma:A.2.1} 
    Under Assumption \ref{as.A}.\ref{as.A.1} and Assumption \ref{as.A}.\ref{as.A.2}, we have 
    \begin{align*}
        \max_{1\leq j\leq p} \sum_{i=1}^n \left\|(Z^i)^\top \left(\Sigma_a^i\right)^{-1} X_j^i \right\|_2^2 \left\|\Psi\right\|_2 + \left\|\left(\Sigma_a^i\right)^{-1} X_j^i\right\|_2^2 \|R^i\|_2
        \leq \begin{cases}
            c_1\frac{nm}{q} &, q>c_0m,\\
            c_1n &, m>c_0q \text{ and } q=p,\\
            c_1mn &, m>c_0q \text{ and } q<p,
        \end{cases}
    \end{align*}
    with probability at least $1-4\exp\{-cn\} - 12\exp\{-c\log(n)\} - 2\exp\{-cmnq^{-\qm}\} - \exp\{-cn(m/q)^{\qm}\}$.
    
    If we additionally assume Assumption \ref{as.A.add}.\ref{as.A.3}, we have 
    \begin{align*}
    \max_{1\leq j\leq p} \sum_{i=1}^n \left\|(Z^i_{S_\psi})^\top \left(\Sigma_a^i\right)^{-1} X_j^i \right\|_2^2 \left\|\Psi\right\|_2 + \left\|\left(\Sigma_a^i\right)^{-1} X_j^i\right\|_2^2 \|R^i\|_2 \leq \begin{cases}
            \frac{c_1mn}{q}\left(1 \wedge \frac{m\log^2(n)}{q}\right) &, q>c_0m,\\
            c_1n &, m>c_0q \text{ and } p=q,\\
            c_1mn &, m>c_0q \text{ and } q<p,
        \end{cases}
\end{align*}
with probability at least $1-4\exp\{-cn\} -6\exp\{-c\log(n)\} - 2\exp\{-cmnq^{-\qm}\} -\exp\left\{-cn\left(m/q\right)^{\qm} \right\}$.
    
    \item \label{lemma:A.2.0} Define 
    \begin{align*}
        z_0^* = \max_{1\leq j \leq p} \left|\frac{1}{\tr(\Sigma_a^{-1})} X^\top_j \Sigma_a^{-1} (y-X\beta^*) \right|.
    \end{align*}
    Under Assumption \ref{as.A}.\ref{as.A.1} and Assumption \ref{as.A}.\ref{as.A.2}, we have
    \begin{align*}
        z_0^* \leq \begin{cases}
        c_1 \sqrt{\frac{q\log(p)}{nm}} &, q>c_0m ,\\
        c_1 \sqrt{\frac{\log(p)\log^2(n)}{n}} &, q>c_0m \text{ and Assumption~\ref{as.A.add}.\ref{as.A.3}} also holds,\\
        c_1 \sqrt{\frac{\log(p)}{nm^2}} &, m>c_0q \text{ and } p=q ,\\
        c_1 \sqrt{\frac{\log(p)}{nm}} &, m>c_0q \text{ and } p>q .\\
        \end{cases}
    \end{align*}
    with probability at least $1-4\exp\{-cn\} -12\exp\{-c\log(n)\} - 2\exp\{-cmnq^{-\qm}\} -\exp\left\{-cn\left(m/q\right)^{\qm} \right\}$.
\end{enumerate}
\end{lemma}

\newpage

\subsection{Proof of Theorem \ref{thm:S1}}

\begin{proof}
$\left.\right.$

Based on the definition of $\hat\beta$, we can get: 
\begin{align*}
    \frac{1}{2 \tr(\Sigma_a^{-1})} \left\|\Sigma_a^{-1/2}(y-X\hat\beta) \right\|^2_2 + \lambda_a\|\hat\beta\|_1 \leq \frac{1}{2 \tr(\Sigma_a^{-1})} \left\|\Sigma_a^{-1/2}(y-X\beta^*) \right\|^2_2 + \lambda_a\|\beta^*\|_1.
\end{align*}
Denoting $\hat u =\hat\beta -\beta^*$ and rearranging the terms, we get
\begin{align}
    0 \leq \frac{1}{2 \tr(\Sigma_a^{-1})}\left\|\Sigma_a^{-1/2}X\hat u \right\|^2_2 \leq (z_0^* + \lambda_a) \|\hat u_S\|_1 + (z_0^* - \lambda_a) \|\hat u_{S^c}\|_1, \label{e.t.1.1}
\end{align}
where 
\begin{align*}
    z_0^* := \max_{1\leq j \leq p} \left|\frac{1}{ \tr(\Sigma_a^{-1})} X^\top_j \Sigma_a^{-1}(y-X\beta^*)\right|.
\end{align*}
Based on Lemma \ref{lemma:A.3}.\ref{lemma:A.3.1} and Lemma \ref{lemma:A.1}.\ref{lemma:A.1(6.5)}, we have that:
 \begin{align*}
     \frac{1}{2 \tr(\Sigma_a^{-1})}\left\|\Sigma_a^{-1/2}X\hat u \right\|^2_2 \geq \frac{\|\hat u\|^2_2 }{2 \tr(\Sigma_a^{-1})} \sigma_{\min}(X^\top \Sigma_a^{-1}X) \geq 
     \begin{cases}
     c_1    \|\hat u\|^2_2 &, q>c_0m,\\
     c_1 \frac{1}{m}\|\hat u\|^2_2 &, m>c_0q.
     \end{cases}
 \end{align*}
Based on Lemma \ref{lemma:A.2}.\ref{lemma:A.2.0}:
\begin{align*}
    z_0^* \leq \begin{cases}
        c_1 \sqrt{\frac{q\log(p)}{nm}} &, q>c_0m ,\\
        c_1 \sqrt{\frac{\log(p)\log^2(n)}{n}} &, q>c_0m \text{ and assume Assumption \ref{as.A.add}.\ref{as.A.3}},\\
        c_1 \sqrt{\frac{\log(p)}{nm^2}} &, m>c_0q \text{ and } p=q ,\\
        c_1 \sqrt{\frac{\log(p)}{nm}} &, m>c_0q \text{ and } p>q .\\
        \end{cases}
\end{align*}
Thus with probability at least $1-4\exp\{-cn\} -12\exp\{-c\log(n)\} - 2\exp\{-cmnq^{-\qm}\} -\exp\left\{-cn\left(m/q\right)^{\qm} \right\}$, we can get the following results:
\begin{enumerate}
    \item When $q>c_0m$:
     With $\lambda_a = c_2\sqrt{\frac{q\log(p)}{nm}}$ for suitably large $c_2$, we have $z_0^* \leq \lambda_a/2$ with high probability. Then based on \eqref{e.t.1.1} we have 
     \begin{align*}
         c_1\|\hat u\|_2^2 \leq 3\lambda_a\|\hat u_S\|_1 - \lambda_a\|\hat u_{S^c}\|_1 \leq 3\lambda_a \|\hat u_S\|_2^2 \leq 3\lambda_a \sqrt{s}\|\hat u\|_2^2.
     \end{align*}
     Thus we can obtain
     \begin{align*}
         &\|\hat u\|_2 \leq O_p\left(\sqrt{\frac{sq\log(p)}{mn}}\right),\\
         &\|\hat u\|_1 \leq O_p\left(s\sqrt{\frac{q\log(p)}{mn}}\right),\\
         &\|\Sigma_a^{-1/2} X \hat u\|_2^2 \leq O_p\left(s\log(p)\right).
     \end{align*}

    \item When $q>c_0m$ and additionally assume Assumption \ref{as.A.add}.\ref{as.A.3}:
    With $\lambda_a = c_2\sqrt{\frac{\log(p)\log^2(n)}{n}}$ for suitably large $c_2$, we have $z_0^* \leq \lambda_a/2$ with high probability. Then following similar arguments as before, we can obtain
     \begin{align*}
         &\|\hat u\|_2 \leq O_p\left(\sqrt{\frac{s\log^2(n)\log(p)}{n}}\right),\\
         &\|\hat u\|_1 \leq O_p\left(s\sqrt{\frac{\log^2(n)\log(p)}{n}}\right),\\
         &\|\Sigma_a^{-1/2} X \hat u\|_2^2 \leq O_p\left(\frac{sm\log^2(n)\log(p)}{q}\right).
     \end{align*}

    \item When $m>c_0q$ and $p=q$:
    With $\lambda_a = c_2\sqrt{\frac{\log(p)}{nm^2}}$ for suitably large $c_2$, we have $z_0^* \leq \lambda_a/2$ with high probability. Then following similar arguments as before, we can obtain
     \begin{align*}
         &\|\hat u\|_2 \leq O_p\left(\sqrt{\frac{s\log(p)}{n}}\right),\\
         &\|\hat u\|_1 \leq O_p\left(s\sqrt{\frac{\log(p)}{n}}\right),\\
         &\|\Sigma_a^{-1/2} X \hat u\|_2^2 \leq O_p\left(s\log(p)\right).
     \end{align*}
     
    \item When $m>c_0q$ and $p>q$:
    With $\lambda_a = c_2\sqrt{\frac{\log(p)}{nm}}$ for suitably large $c_2$, we have $z_0^* \leq \lambda_a/2$ with high probability. Then following similar arguments as before, we can obtain
     \begin{align*}
         &\|\hat u\|_2 \leq O_p\left(\sqrt{\frac{sm\log(p)}{n}}\right),\\
         &\|\hat u\|_1 \leq O_p\left(s\sqrt{\frac{m\log(p)}{n}}\right),\\
         &\|\Sigma_a^{-1/2} X \hat u\|_2^2 \leq O_p\left(sm\log(p)\right).
     \end{align*}
\end{enumerate}
\end{proof}

\subsection{Proof of related lemmas for Theorem \ref{thm:S1}}

\begin{proof}[Proof of Lemma \ref{lemma:A.1}]
$\left.\right.$

\textit{Lemma~\ref{lemma:A.1}.\ref{lemma:A.1(1)})}
{
$\left.\right.$

By Theorem 5.32 in \cite{vershynin2010introduction}, we have $|\sqrt{q} -\sqrt{m}| \leq \E(\sigma(Z)) \leq \sqrt{q} + \sqrt{m}$. With $q>c_0m$ or $m > c_0 q$, we have $(\sqrt{q} \vee \sqrt{m})\left(1-\frac{1}{\sqrt{c_0}}\right) \leq \E(\sigma(Z)) \leq (\sqrt{q} \vee \sqrt{m})\left(1+\frac{1}{\sqrt{c_0}}\right)$, and thus $\E(\sigma(Z)) \asymp \sqrt{q} \vee \sqrt{m}$.
}
\\

\textit{Lemma \ref{lemma:A.1}.\ref{lemma:A.1(2)})}
{
$\left.\right.$

By Proposition 5.34 in \cite{vershynin2010introduction}, we have 
\begin{align*}
    \P\left(|\sigma(Z) - \E(\sigma(Z))|>t \right) \leq 2\exp\{-t^2/2\}.
\end{align*}
Thus $\sigma(Z) - \E(\sigma(Z)) \in \SG(1)$. 
}
\\

\textit{Lemma \ref{lemma:A.1}.\ref{lemma:A.1(3)})}
{
$\left.\right.$

By Lemma \ref{lemma:A.1}.\ref{lemma:A.1(2)}, we have $\mathrm{Var}(\sigma(Z)) \leq 1$. Then 
\begin{align*}    
\E(\sigma^2(Z)) & = \mathrm{Var}(\sigma(Z)) + \E(\sigma(Z))^2 \leq 1 + \E(\sigma(Z))^2
\asymp m\vee q;\\
    \E(\sigma^2(Z)) & \geq \E(\sigma(Z))^2 \asymp m \vee q.
\end{align*}
}

\textit{Lemma \ref{lemma:A.1}.\ref{lemma:A.1(4)})}
{
$\left.\right.$

By Lemma \ref{lemma:A.1}.\ref{lemma:A.1(2)} and the results in the Appendix B of \cite{honorio2014tight}, we have $\sigma^2(Z) - \E(\sigma^2(Z)) \in \SE(32, 4)$. Then for independent copies $Z^i$'s, we have
\begin{align*}
    \P\left(\left|\sum_{i=1}^n \sigma^2(Z^i) - n\E(\sigma^2(Z))\right|\right) \geq 2\exp\left\{-\frac{1}{2}\min\left(\frac{t^2}{32n}, \frac{t}{4}\right)\right\}.
\end{align*}
Thus by Lemma \ref{lemma:A.1}.\ref{lemma:A.1(3)}, we have $\sum_{i=1}^n \sigma^2(Z^i) \asymp n(m\vee q)$ with probability at least $1-2\exp\{-c_1n(m\vee q)\}$.
}
\\

\textit{Lemma \ref{lemma:A.1}.\ref{lemma:A.1(5)})}
{
$\left.\right.$

By Jensen's inequality, 
\begin{align*}
    \E\left(\frac{1}{\sigma^2(Z) +c}\right) \geq \frac{1}{\E(\sigma^2(Z)) +c}.
\end{align*}

For simpler notation, denote $\sigma^2 = \sigma^2(Z)$ and $\mu = \E(\sigma^2(Z))$ in the following proof. For some $0 < k < 1$, with $f(\sigma^2)$ being the probability density function of $\sigma^2$, we have
\begin{align*}
    \E\left(\frac{1}{\sigma^2+c}\right) &  = \int_0^{k\mu} \frac{1}{\sigma^2+c} f(\sigma^2) \mathrm{d}\sigma^2+ \int_{k\mu} ^ \infty \frac{1}{\sigma^2+c} f(\sigma^2) \mathrm{d}\sigma^2 \\
    & \leq \int_0^{k\mu} \frac{1}{c} f(\sigma^2) \mathrm{d}\sigma^2+ \int_{k\mu} ^ \infty \frac{1}{k\mu+c} f(\sigma^2) \mathrm{d}\sigma^2 \\
    & = \frac{1}{c} \P(\sigma^2 < k\mu) + \frac{1}{k\mu + c} \P(\sigma^2 \geq k\mu) \\
    & \leq \frac{1}{c} 2\exp\left\{-\frac{1}{2}\min\left(\frac{(1-k)^2 \mu^2}{32}, \frac{(1-k)\mu}{4}\right)\right\} + \frac{1}{k\mu + c},
\end{align*}
using the fact that $\sigma^2 - \E(\sigma^2) \in \SE(32, 4)$ (Lemma \ref{lemma:A.1}.\ref{lemma:A.1(4)}). Then take $k=1/2$, we have 
\begin{align*}
    \E\left(\frac{1}{\sigma^2+c}\right) & \leq \frac{2}{\mu + 2c} + \frac{2}{c}\exp\left\{-\frac{1}{2}\min\left(\frac{\mu^2}{128}, \frac{\mu}{8}\right)\right\} \\
    & \leq  \frac{4}{\mu + c}
\end{align*}
for all $\mu > c_1 >0$ for some suitably large constant $c_1$. By Lemma \ref{lemma:A.1}.\ref{lemma:A.1(3)}, it suffices to assume $m\vee q > c_2 >0$ for some suitably large constant $c_2$.
}
\\

\textit{Lemma \ref{lemma:A.1}.\ref{lemma:A.1(6.1)})}
{
$\left.\right.$

For simpler notation, we denote $\sigma^2 = \sigma^2(Z)$, $\mu = \E(\sigma^2)$ and $E = \E\left(\frac{1}{\sigma^2+c}\right)$ in the following proof. We would like to show that $\forall\ t \in \R$,
\begin{align*}
    \P\left( \left|\frac{1}{\sigma^2 + c} - E \right| < t\right) \geq 1 - 2\exp\left\{-\frac{1}{2}\min \left(\frac{t^2}{c_1 E^2}, \frac{t}{c_1E}\right)\right\}.
\end{align*}
We consider three cases based on the value of $t$:
\begin{itemize}
    \item Case 1: \textit{$t \leq E$}:
    \begin{align}
        \P\left( \left|\frac{1}{\sigma^2 + c} - E \right| < t\right) & = \P\left(\frac{1}{E+t} -\mu -c \leq \sigma^2 -\mu \leq \frac{1}{E-t} -\mu -c \right). \label{a.1.6.1.1}
    \end{align}
    Denote $t_1 = \mu +c -\frac{1}{E+t}$, $t_2 = \frac{1}{E-t} -\mu -c$. Note that we can show $t_1 \geq 0, t_2\geq 0$ because of $\frac{1}{\mu+c} \leq E \leq \frac{4}{\mu+c}$ (Lemma \ref{lemma:A.1}.\ref{lemma:A.1(5)}). Then based on the sub-gaussian property of $\sigma^2$ (Lemma~\ref{lemma:A.1}.\ref{lemma:A.1(4)}) and the equation \eqref{a.1.6.1.1}, we have
    \begin{align*}
         \P\left( \left|\frac{1}{\sigma^2 + c} - E \right| < t\right) & \geq 1-\exp\left\{-\frac{1}{2}\min\left(\frac{t_1^2}{32}, \frac{t_1}{4}\right)\right\}-\exp\left\{-\frac{1}{2}\min\left(\frac{t_2^2}{32}, \frac{t_2}{4}\right)\right\}.
    \end{align*}
    We next show that $\forall\ 0 \leq t \leq E$,
    \begin{align}
        \exp\left\{-\frac{1}{2}\min\left(\frac{t_1^2}{32}, \frac{t_1}{4}\right)\right\} + \exp\left\{-\frac{1}{2}\min\left(\frac{t_2^2}{32}, \frac{t_2}{4}\right)\right\} \leq 2\exp\left\{-\frac{1}{2}\min\left(\frac{t^2}{32E^2}, \frac{t}{32E}\right)\right\}. \label{E.A.1.6}
    \end{align}
    Note that $\frac{t_1^2}{32} \leq \frac{t_1}{4}$ for $0 \leq t \leq t_1^* := \frac{1}{\mu+c-8}-E$, and $\frac{t_2^2}{32} \leq \frac{t_2}{4}$ for $0 \leq t \leq t_2^* := E-\frac{1}{\mu+c+8}$. Then:
    \begin{enumerate}
        \item On $t\in [0, t_1^* \wedge t_2^*]$:
        \begin{align*}
            \text{LHS of }\eqref{E.A.1.6}& = \exp\left\{-\frac{1}{2}\frac{t_1^2}{32}\right\} + \exp\left\{-\frac{1}{2}\frac{t_2^2}{32}\right\} \\
            & \leq 2 \exp\left\{-\frac{1}{4}\left(\frac{t_1}{8} + \frac{t_2}{8}\right)^2\right\} \quad \quad \text{(By Jensen's inequality)} \\
            & \leq 2 \exp\left\{ -\frac{1}{256}\left(\frac{2t}{E^2-t^2}\right)^2\right\} \\
            & \leq 2\exp\left\{-\frac{t^2}{64E^2}\right\} \quad \quad \text{(For $m\vee q > c_1$ for suitably large $c_1 >0$, we have $E^2 <1$)} \\
            & \leq \text{RHS of }\eqref{E.A.1.6}
        \end{align*}
        \item On $t \geq t_1^* \vee t_2^*$:
        \begin{align*}
            \text{LHS of }\eqref{E.A.1.6}& = \exp\left\{-\frac{1}{2}\frac{t_1}{4}\right\} + \exp\left\{-\frac{1}{2}\frac{t_2}{4}\right\} \\
            & \leq 2 \exp\left\{-\frac{1}{2}\left(\frac{t_1}{8} + \frac{t_2}{8}\right)\right\} \quad \quad \text{(By Jensen's inequality)} \\
            & = 2 \exp\left\{- \frac{1}{16} \left(\frac{2t}{E^2-t^2}\right)\right\} \\
            & \leq 2 \exp\left\{-\frac{t^2}{64E^2}\right\}  \quad \quad \text{(For $m\vee q > c_1$ for suitably large $c_1 >0$, we have $E <1$)} \\
            & \leq \text{RHS of }\eqref{E.A.1.6}.
        \end{align*}
        \item On $t \in [t_1^*\wedge  t_2^*, t_1^*\vee  t_2^*]$:
        \begin{enumerate}
            \item When $t_1^* \leq t_2^*$: 
            \begin{align*}
                 \text{LHS of }\eqref{E.A.1.6}& = \exp\left\{-\frac{1}{2}\frac{t_1}{4}\right\} + \exp\left\{-\frac{1}{2}\frac{t_2^2}{32}\right\} \\
                & = \exp\left\{-\frac{1}{8}\left(\mu + c -\frac{1}{E+t}\right)\right\} + \exp\left\{-\frac{1}{64}\left(\frac{1}{E-t}-\mu-c\right)^2\right\},
            \end{align*}
            where the last expression takes maximum value at $t=t_1^*$. Thus, denoting $\Delta_1 = \frac{1}{E-t_1^*}-\mu-c$, we have $\Delta_1\geq 0$, and
            \begin{align*}
                 \text{LHS of }\eqref{E.A.1.6}& \leq \exp\{-1\} + \exp\left\{-\frac{\Delta_1^2}{64}\right\} \\
                & \leq 2 \exp\left\{-\frac{1}{4}\left(1 + \frac{\Delta_1}{8}\right)^2\right\}\\
                & \leq 2 \exp\left\{ -\frac{1}{64}\left(1-\frac{1}{E(\mu +c+8)}\right)^2\right\} \quad \quad \text{(since $E \geq \frac{1}{\mu+c}$ by Lemma \ref{lemma:A.1}.\ref{lemma:A.1(5)})}\\
               & = 2 \exp\left\{-\frac{(t_2^*)^2}{64E^2}\right\}\\
               & \leq 2 \exp\left\{-\frac{t^2}{64E^2}\right\} \\
               & \leq \text{RHS of}\eqref{E.A.1.6}.
            \end{align*}
            
            \item When $t_1^* > t_2^*$: similarly, the LHS of \eqref{E.A.1.6} reaches maximum value at $t=t_2^*$. Then denoting $\Delta_2 = \mu + c - \frac{1}{E+t_2^*}$, we have
            \begin{align*}
                 \text{LHS of }\eqref{E.A.1.6}& = \exp\left\{-\frac{1}{2}\frac{t_2}{4}\right\} + \exp\left\{-\frac{1}{2}\frac{t_1^2}{32}\right\}\\
                 & \leq \exp\{-1\} + \exp\left\{-\frac{\Delta_2^2}{64}\right\} \\
                 & \leq 2 \exp\left\{-\frac{1}{4}\left(1 + \frac{\Delta_2}{8}\right)^2\right\};\\
                 \text{RHS of }\eqref{E.A.1.6} & \geq 2 \exp\left\{-\frac{(t_1^*)^2}{64E^2}\right\};
            \end{align*}
            and
            \begin{align*}
                \frac{t_1^*}{8E} &  = \frac{1}{8} \left(\frac{1}{E(\mu + c-8)}-1\right) \\
                & \leq \frac{1}{8} \left(\frac{\mu + c}{\mu + c -8}-1\right) \quad \quad \text{(since $E \geq \frac{1}{\mu+c}$ by Lemma \ref{lemma:A.1}.\ref{lemma:A.1(5)})}\\
                & \leq \frac{1}{2} + \frac{\Delta_2}{16},
            \end{align*}
            where the last inequality hold for $m\vee q >c_2$ for suitably large $c_2>0$, based on Lemma \ref{lemma:A.1}.\ref{lemma:A.1(3)}.
        \end{enumerate}
        Thus we have shown \eqref{E.A.1.6} holds for $t\leq E$.
        \end{enumerate}

        \item Case 2: \textit{$E < t < \frac{1}{c}$}: Denoting $t_1 = \frac{1}{E+t}-\mu-c$, using Lemma~\ref{lemma:A.1}.\ref{lemma:A.1(4)}, we have that:
        \begin{align*}
            \P\left(\left|\frac{1}{\sigma^2+c}-E\right|\leq t\right) & = \P\left(\sigma^2-\mu \geq \frac{1}{E+t}-c-\mu\right) \\
            & \geq 1-\exp\left\{-\frac{1}{2}\min\left(\frac{t_1^2}{32}, \frac{t_1}{4}\right)\right\}.
        \end{align*}
        Then we want to show
        \begin{align}
            1-\exp\left\{-\frac{1}{2}\min\left(\frac{t_1^2}{32}, \frac{t_1}{4}\right)\right\} \geq 1-2\exp\left\{-\frac{1}{2}\min\left(\frac{c_1^2t^2}{128E^2}, \frac{ct}{8E}\right)\right\} \label{E.A.1.6.2}.
        \end{align}
        To show \eqref{E.A.1.6.2}, note that
        \begin{align*}
            \frac{t_1^2}{32} \geq \frac{c^2 t^2}{128E^2} & \Leftrightarrow t_1 \geq \frac{ct}{2E} 
            \Leftrightarrow \mu + c \geq \frac{ct}{2E} + \frac{1}{E+t};
        \end{align*}
        and we can show
        \begin{align*}
            \frac{ct}{2E} + \frac{1}{E+t} &\leq \max\left(\frac{c}{2} + \frac{1}{2E}, \frac{1}{2E} + \frac{1}{E+ \frac{1}{c}}\right) \\
            & \leq \max\left(\frac{c}{2} + \frac{\mu + c}{2}, \frac{\mu + c}{2} + c\right) \\
            & \leq \mu + c
        \end{align*}
        using that fact that $E \geq \frac{1}{\mu + c}$ (Lemma \ref{lemma:A.1}.\ref{lemma:A.1(5)}) for $m \vee q > c_2$ for suitably large $c_2>0$. Thus, \eqref{E.A.1.6.2} holds.

    \item Case 3: \textit{$t \geq \frac{1}{c}$:} We have $\P\left(\left|\frac{1}{\sigma^2+c}-E\right|\leq t\right) =1$ since $\frac{1}{\sigma^2+c} \leq \frac{1}{c}$.
\end{itemize}

Thus, we have shown $\P\left(\left|\frac{1}{\sigma^2+c}-E\right|\leq t\right) \geq 1-2\exp\left\{-c_2\min\left(\frac{t^2}{E^2}, \frac{t}{E}\right)\right\}$, which implies $\frac{1}{\sigma^2+c}-E \in \SE(c_2E^2, c_2E)$.
}
\\

\textit{Lemma \ref{lemma:A.1}.\ref{lemma:A.1(6.2)})} % and 6.3, 6.4
{
$\left.\right.$

By Lemma \ref{lemma:A.1}.\ref{lemma:A.1(6.1)}, it is straightforward that
\begin{align*}
    \P&\left( \left|\sum_{i=1}^n\frac{1}{\sigma^2(Z^i)+c}-\sum_{i=1}^n\E\left(\frac{1}{\sigma^2(Z^i)+c}\right)\right|\leq t\right) \\
    & \geq 1-2\exp\left\{-c_1\min\left(\frac{t^2}{\sum_{i=1}^n\E\left(\frac{1}{\sigma^2(Z^i)+c}\right)^2}, \frac{t}{\max_i\E\left(\frac{1}{\sigma^2(Z^i)+c}\right)}\right)\right\}.
\end{align*}
Based on Lemma \ref{lemma:A.1}.\ref{lemma:A.1(5)}, we have $\sum_{i=1}^n\frac{1}{\sigma^2(Z^i)+c} \asymp \frac{n}{m \vee q}$ with probability at least $1-2\exp\{-c_2n\}$.

By Lemma \ref{lemma:A.1}.\ref{lemma:A.1(6.1)}, we have 
\begin{align*}
    \P&\left(\forall\ i, \left|\frac{1}{\sigma^2(Z^i)+c}-\E\left(\frac{1}{\sigma^2(Z^i)+c}\right)\right|\geq t\right) \\
    & \leq 2\exp\left\{\log(n)-c_1\min\left(\frac{t^2}{\max_i\E\left(\frac{1}{\sigma^2(Z^i)+c}\right)^2}, \frac{t}{\max_i\E\left(\frac{1}{\sigma^2(Z^i)+c}\right)}\right)\right\}.
\end{align*}
Thus based on Lemma \ref{lemma:A.1}.\ref{lemma:A.1(5)}, and the trivial bound $\max_i\frac{1}{\sigma^2(Z^i)+c} \leq \frac{1}{c}$, we have $\max_i\frac{1}{\sigma^2(Z^i)+c} \leq \frac{1}{c} \wedge \frac{c_2\log(n)}{m \vee q}$ with probability at least $1-2\exp\{-c_3n\}$.

By Lemma \ref{lemma:A.1}.\ref{lemma:A.1(4)}, we have 
\begin{align*}
    \P\left(\forall\ i, \left|\sigma^2(Z^i) - \E(\sigma^2(Z^i)) \right| \geq t\right) \leq 2\exp\left\{\log(n)-c_1\min\left(\frac{t^2}{32}, \frac{t}{4}\right)\right\}.
\end{align*}
Thus $\max_i\sigma^2(Z^i) \leq c_2(\log(n) + m\vee q)$ and $\min_i \frac{1}{\sigma^2(Z^i)+c} \geq \frac{c_3}{\log(n) + m \vee q}$ with probability at least $1-2\exp\{-c_4n\}$.
}
\\

\textit{Lemma \ref{lemma:A.1}.\ref{lemma:A.1(6.5)})}
{
$\left.\right.$

Note that $\Tr\left((\Sigma_a^i)^{-1}\right) = \sum_{l=1}^m \frac{1}{a\sigma_l^2(Z^i) + 1}$, where $\sigma_l^2(Z^i)$'s are the singular values of $Z^i$.

For $q>c_0m$: $\sigma_l^2(Z^i)$'s are positive. We then have
\begin{align*}
    \frac{m}{a\sigma_{\max}^2(Z^i) +1} \leq \Tr\left((\Sigma_a^i)^{-1}\right) \leq \frac{m}{a\sigma_{\min}^2(Z^i) +1};
\end{align*}
and based on Lemma \ref{lemma:A.1}.\ref{lemma:A.1(6.2)}:
\begin{align*}
    & \P\left(\max_i\Tr\left((\Sigma_a^i)^{-1}\right) \leq c_1 m\left(1\wedge \frac{\log(n)}{q}\right)\right) \geq 1-2\exp\{-c_2\log(n)\},\\
    & \P\left(\min_i\Tr\left((\Sigma_a^i)^{-1}\right) \geq \frac{c_1 m }{\log(n)+q}\right) \geq 1-2\exp\{-c_2\log(n)\},\\
    & \P\left(\sum_{i=1}^n\Tr\left((\Sigma_a^i)^{-1}\right) \asymp \frac{nm}{q}\right) \geq 1-4\exp\{-c_3n\}.
\end{align*}

For $m > c_0q$: $\sigma_l^2(Z^i)$'s are zero for $l>q$, and $\sigma_l^2(Z^i)$'s are positive for $1 \leq l \leq q$. Then $\Tr\left((\Sigma_a^i)^{-1}\right) = m-q + \sum_{l=1}^q \frac{1}{a\sigma_l^2(Z^i) +1}$. We thus have:
\begin{align*}
    & \P\left(\max_i\Tr\left((\Sigma_a^i)^{-1}\right) \leq m-q + c_1 q\left(1\wedge \frac{\log(n)}{m}\right) \leq c_1 \left(m + q\left(1\wedge \frac{\log(n)}{m}\right)\right) \right) \geq 1-2\exp\{-c_2\log(n)\},\\
    & \P\left(\min_i\Tr\left((\Sigma_a^i)^{-1}\right) \geq m-q+ \frac{c_1 q }{\log(n)+m} \geq c_1\left(m + \frac{q }{\log(n)+m}\right)\right) \geq 1-2\exp\{-c_2\log(n)\},\\
    & \P\left(\sum_{i=1}^n\Tr\left((\Sigma_a^i)^{-1}\right) \asymp n(m-q) + \frac{nq}{m} \asymp nm\right) \geq 1-4\exp\{-c_3n\}.
\end{align*}
}
\\

\textit{Lemma \ref{lemma:A.1}.\ref{lemma:A.1(8)})}
{
$\left.\right.$

For any $q\times q $ orthogonal matrix $P$, $Z$ and $ZP$ follow the same distribution. Thus
\begin{align*}
    \E\left(Z^\top (a ZZ^\top + I_m)^{-1} Z\right) & = \E\left((ZP)^\top (a ZPP^\top Z^\top + I_m)^{-1} ZP\right) \\
    & = P^\top\E\left(Z^\top (a ZZ^\top + I_m)^{-1} Z\right)P.
\end{align*}
Then by Proposition 2.14 in \cite{EatonMorrisL2007Ms}, we have $\E\left(Z^\top (a ZZ^\top + I_m)^{-1} Z\right) = kI_q$ for some $k\in \R$.

We then have
\begin{align*}
    kq & = \tr(kI_q) = \tr\left(\E\left(Z^\top (a ZZ^\top + I_m)^{-1} Z\right)\right) \\
    & = \E\left(\tr \left(I_m - (a ZZ^\top + I_m)^{-1}\right)\right) \\
    & = m - \E\left(\sum_{l=1}^m\frac{1}{a \sigma^2_l(Z) +1} \right).
\end{align*}

When $q>c_0m$, $\sigma^2_l(Z)$'s are positive. By Lemma \ref{lemma:A.1}.\ref{lemma:A.1(3)} and Lemma \ref{lemma:A.1}.\ref{lemma:A.1(5)} we have
\begin{align}
    m-\frac{c_1m}{q} \leq m - m\E\left(\frac{1}{a \sigma^2_{\min}(Z) +1} \right)\leq kq \leq m - m\E\left(\frac{1}{a \sigma^2_{\max}(Z) +1} \right) \leq m-\frac{c_2m}{q}. \label{a.1.8.1}
\end{align}
Thus $k \asymp \frac{m}{q}$ when $q>c_0m$.

When $m>c_0q$, $\sigma^2_l(Z)$'s are positive and $\sigma^2_l(Z)=0$ for $l>q$. Then similar to the proof of \eqref{a.1.8.1}, by Lemma \ref{lemma:A.1}.\ref{lemma:A.1(3)} and Lemma \ref{lemma:A.1}.\ref{lemma:A.1(5)}, we have
\begin{align*}
    q-\frac{c_1q}{m} \leq q-q \E\left( \frac{1}{a\sigma_{\min}^2(Z) +1}\right)\leq kq = q - \E\left(\sum_{l=1}^q \frac{1}{a\sigma_l^2(Z) +1}\right) \leq  q-q \E\left( \frac{1}{a\sigma_{\max}^2(Z) +1}\right) \leq q-\frac{c_2q}{m}.
\end{align*}
Thus $k \asymp 1$ when $m>c_0q$.

Then since $\|(Z^i)^\top (\Sigma_a^i)^{-1} Z^i\|_2 \leq \max_l \frac{\sigma^2_l(Z^i)}{a\sigma^2_l(Z^i) +1} \leq \frac{1}{a}$, by Matrix Chernoff bound \cite{tropp2015introduction} we have:
\begin{align*}
    & \P\left(\sigma_{\min}\left(\sum_{i=1}^n(Z^i)^\top (\Sigma_a^i)^{-1} Z^i\right) \geq \frac{1}{2} n \sigma_{\min} \left(\E\left((Z^i)^\top (\Sigma_a^i)^{-1} Z^i\right)\right)\right) \\
    & \quad \geq 1-\exp\left\{\log(q) - \left(\frac{1}{2}-\log{\sqrt{2}}\right)an\sigma_{\min} \left(\E\left((Z^i)^\top (\Sigma_a^i)^{-1} Z^i\right)\right) \right\};\\
    & \P\left(\sigma_{\max}\left(\sum_{i=1}^n(Z^i)^\top (\Sigma_a^i)^{-1} Z^i\right) \leq \frac{3}{2} n \sigma_{\max} \left(\E\left((Z^i)^\top (\Sigma_a^i)^{-1} Z^i\right)\right)\right) \\
    & \quad \geq 1-\exp\left\{\log(q) - \left(\frac{3}{2}\log{\frac{3}{2}} - \frac{1}{2}\right) an\sigma_{\min} \left(\E\left((Z^i)^\top (\Sigma_a^i)^{-1} Z^i\right)\right) \right\}.
\end{align*}
Plugging in $\E\left(Z^\top (a ZZ^\top + I_m)^{-1} Z\right) = kI_q$ with $k \asymp \left(\frac{m}{q}\right)^{\qm}$, we obtain the stated results in the lemma.
}
\\

\textit{Lemma \ref{lemma:A.1}.\ref{lemma:A.1(9)})}
{
$\left.\right.$

By Lemma \ref{lemma:A.1}.\ref{lemma:A.1(6.3)} and Lemma \ref{lemma:A.1}.\ref{lemma:A.1(8)},
\begin{align*}
    \sigma_{\max}\left(\sum_{i=1}^n(Z^i)^\top (\Sigma_a^i)^{-2} Z^i\right) & \leq \sigma_{\max}\left(\sum_{i=1}^n(Z^i)^\top (\Sigma_a^i)^{-1} Z^i\right) \sigma_{\max}\left((\Sigma_a^i)^{-1}\right) \\
    & \leq c_1 n \left(\frac{m}{q}\right)^{\qm} \left(1 \wedge \frac{\log(n)}{m \vee q}\right)
\end{align*}
with probability at least $1-\exp\left\{-c_2n\left(\frac{m}{q}\right)^{\qm}\right\} - 2\exp\{-c_2\log(n)\}$. At the same time, based on Lemma \ref{lemma:A.1}.\ref{lemma:A.1(6.2)} we have
\begin{align*}
    \sigma_{\max}\left(\sum_{i=1}^n(Z^i)^\top (\Sigma_a^i)^{-2} Z^i\right) &\leq \sigma_{\max}\left(\sum_{i=1}^n (\Sigma_a^i)^{-1}\right) \max_i \sigma_{\max}\left((Z^i)^\top (\Sigma_a^i)^{-1} Z^i\right) \\
    & \leq \frac{c_1n}{m \vee q}
\end{align*}
with probability at least $1-2\exp\{-c_2n\}$. Thus with probability at least $1-2\exp\{-c_2n\}-\exp\left\{-c_2n\left(\frac{m}{q}\right)^{\qm}\right\} - 2\exp\{-c_2\log(n)\}$ we have
\begin{align*}
    \sigma_{\max}\left(\sum_{i=1}^n(Z^i)^\top (\Sigma_a^i)^{-2} Z^i\right) \leq \begin{cases}
        c_1\frac{n}{q}\left(1 \wedge \frac{m\log(n)}{q}\right) &,  q>c_0m \\
        c_1 \frac{n}{m} &, m>c_0q
    \end{cases}
\end{align*}
}
\end{proof}

\begin{proof}[Proof of Lemma \ref{lemma:A.3}]
$\left.\right.$

\textit{Lemma \ref{lemma:A.3}.\ref{lemma:A.3.1})}
{
$\left.\right.$

Define $\check X^i = X^i (\Sigma_X^i)^{-1/2}$ and $\check Z^i = Z^i (\Sigma_Z^i)^{-1/2}$. Conditional on $\{\Sigma_X^i\}_{i=1}^n$ and $\{\Sigma_Z^i\}_{i=1}^n$, the entries of $\check X^i$'s and $\check Z^i$'s independently follow $N(0,1)$ distribution. Then we have
\begin{align*}
    X^\top \Sigma_a X  & = \sum_{i=1}^n (\Sigma_X^i)^{1/2}(\check X^i)^\top (a \check Z^i \Sigma^i_Z (\check Z^i)^\top + I_m)^{-1} \check X^i (\Sigma_X^i)^{1/2} \\
    & \preceq \max_i \sigma_{\max}(\Sigma^i_X) \sum_{i=1}^n (\check X^i)^\top (a \sigma_{\min}(\Sigma^i_Z) \check Z^i(\check Z^i)^\top + I_m)^{-1} \check X^i,
\end{align*}
and similarly, 
\begin{align*}
    X^\top \Sigma_a X & \succeq \min_i \sigma_{\min}(\Sigma^i_X) \sum_{i=1}^n (\check X^i)^\top (a \sigma_{\max}(\Sigma^i_Z) \check Z^i(\check Z^i)^\top + I_m)^{-1} \check X^i.
\end{align*}
Under Assumption \ref{as.A}.\ref{as.A.2}, we have $\sigma(\Sigma_X^i) \asymp \sigma(\Sigma_Z^i) \asymp 1$ based on \cite{johnson1981eigenvalue}, and thus $\sigma(X^\top \Sigma_a X)$ has the same rate as $\sigma\left(\sum_{i=1}^n (\check X^i)^\top ( c \check Z^i(\check Z^i)^\top + I_m)^{-1} \check X^i\right)$. Therefore, without loss of generality, we work with $\Sigma^i_X=I_p$, $\Sigma^i_Z=I_q$ for the rest of the proof.

When $p=q$: $X^i = Z^i$ for $i=1, \dots, n$. Then by Lemma \ref{lemma:A.1}.\ref{lemma:A.1(8)}, we have $\sigma(X^\top \Sigma_a X) \asymp n\left(m/q\right)^{\qm}$ with probability at least $1-\exp\left\{-cn\left(m/q\right)^{\qm} \right\}$.

When $p>q$: Recall that $Z^i = X^i_{1:q}$ and denote $Q^i = X^i_{-\{1:q\}}$. Suppose $u$ is a non-random length $q$ vector, and denote $u_Z = u_{1:q}$, $u_Q = u_{-\{1:q\}}$. We have $Q^i u_Q | Z^i \sim N(0, \|u_Q\|^2_2 I_m)$. Then we have
\begin{align}
    u^\top X^\top \Sigma_a^{-1} X u & = \sum_{i=1}^n \left(Z^i u_Z + Q^i u_Q\right)^\top \left(a Z^i (Z^i)^\top +I_m\right)^{-1} \left(Z^i u_Z + Q^i u_Q\right) \nonumber\\
    & = \sum_{i=1}^n u_Z^\top (Z^i)^\top (\Sigma_a^i)^{-1} Z^i u_Z  \label{e.a.3.1.1}\\
    & \quad + \sum_{i=1}^n u_Q^\top (Q^i)^\top (\Sigma_a^i)^{-1} Q^i u_Q \label{e.a.3.1.2}\\
    & \quad + 2\sum_{i=1}^n u_Z^\top (Z^i)^\top (\Sigma_a^i)^{-1} Q^i u_Q \label{e.a.3.1.3}.
\end{align}
\begin{enumerate}
    \item For \eqref{e.a.3.1.1}: By Lemma \ref{lemma:A.1}.\ref{lemma:A.1(8)}, $\eqref{e.a.3.1.1} \asymp \|u_Z\|_2^2 n \left(m/q\right)^{\qm}$ with probability at least $1-\exp\left\{-c_1 n \left(m/q\right)^{\qm}\right\}$. 
    
    \item For \eqref{e.a.3.1.3}: Note that entries of $Q^i$ are i.i.d. realizations of a standard normal distribution. Thus given $Z^i$, $u_Z^\top (Z^i)^\top (\Sigma_a^i)^{-1} Q^i u_Q$ is a Gaussian random variable. Then by the tail bound of Gaussian random variables and Lemma \ref{lemma:A.1}.\ref{lemma:A.1(9)}, we have 
    \begin{align*}
        \P\left( \left|2\sum_{i=1}^n u_Z^\top (Z^i)^\top (\Sigma_a^i)^{-1} Q^i u_Q\right| > 2t \bigm| \{ Z^i\}_{i=1}^n \right) & \leq 2\exp\left\{-\frac{t^2}{\sum_{i=1}^n u_Z^\top (Z^i)^\top (\Sigma_z^i)^{-2} Z^i u_Z \|u_Q\|_2^2}\right\} \\
        & \leq \begin{cases}
            2\exp\left\{-\frac{t^2}{\frac{c_1n}{q} \left(1\wedge \frac{m\log(n)}{q}\right) \|u_Z\|_2^2 \|u_Q\|_2^2}\right\} &, q>c_0m\\
            2\exp\left\{-\frac{t^2}{\frac{c_1n}{m} \|u_Z\|_2^2 \|u_Q\|_2^2}\right\} &, m>c_0q.
        \end{cases}
    \end{align*}
    Thus with probability at least $1-2\exp\{-c_{2}n\} - 4\exp\{-c_{2}\log(n)\} - \exp\left\{-c_{2}n\left(m/q\right)^{\qm}\right\}$, we have:
    \begin{align*}
        \text{\eqref{e.a.3.1.3}} \leq \begin{cases}
            c_3 \sqrt{\frac{n\log(n) \left(1 \wedge \frac{m\log(n)}{q}\right)}{q}}\|u_Z\|_2 \|u_Q\|_2 &, q>c_0m \\
            c_3 \sqrt{\frac{n\log(n)}{m}}\|u_Z\|_2 \|u_Q\|_2 &, m>c_0q. \\
        \end{cases}
    \end{align*}
 \item For \eqref{e.a.3.1.2}: With $\E\left(\sum_{i=1}^n u_Q^\top (Z^i)^\top (\Sigma_a^i)^{-1} Q^i u_Q |\{Z^i\}_{i=1}^n\right) = \tr(\Sigma_a^{-1})\|u_Q\|^2_2$, Hanson-Wright inequality gives:
 \begin{align*}
     & \P\left( \left| \sum_{i=1}^n u_Q^\top (Z^i)^\top (\Sigma_a^i)^{-1} Q^i u_Q - \tr(\Sigma_a^{-1})\|u_Q\|^2_2 \right| > t \bigm| \{Z^i\}_{i=1}^n \right) \\
     & \quad  \leq 2\exp\left\{-c_1 \min\left(\frac{t^2}{\|u_Q\|_2^4 \|\Sigma_a^{-1}\|_F^2}, \frac{t}{\|u_Q\|_2^2 \|\Sigma_a^{-1}\|_2}\right)\right\},
 \end{align*}
where based on Lemma \ref{lemma:A.1}.\ref{lemma:A.1(6.5)}:
\begin{align*}
    & \tr\left(\Sigma_a^{-1}\right) \asymp mn q^{-\qm} \\
    & \|\Sigma_a^{-1}\|_F^2 = \tr(\Sigma_a^{-2}) \leq  a^{-1}\tr(\Sigma_a^{-1}) \asymp mn q^{-\qm} \\
    & \|\Sigma_a^{-1}\|_2 \leq a^{-1}.
\end{align*}
Then \eqref{e.a.3.1.2}$\asymp \|u_Q\|^2_2 mn q^{-\qm}$ with probability at least $1-2\exp\{-c_1mnq^{-\qm}\} - 4\exp\{-c_1n\}$.
\end{enumerate}

Thus with probability at least $1-4\exp\{-cn\} -2\exp\{-c\log(n)\} - 2\exp\{-cmnq^{-\qm}\} -\exp\left\{-cn\left(m/q\right)^{\qm} \right\}$:

For $m>c_0q$: Since $\frac{\log(n)}{nm} = o(1)$, we have
\begin{align*}
& c_1n \|u\|_2^2 \leq c_2 \left( n \|u_Z\|^2_2 + mn \|u_Q\|_2^2 - \sqrt{\frac{n\log(n)}{m}}\|u_Z\|_2 \|u_Q\|_2 \right) \\
& \leq u^\top X^\top \Sigma_a^{-1} X u \\
    & \leq c_2 \left( n \|u_Z\|^2_2 + mn \|u_Q\|_2^2 + \sqrt{\frac{n\log(n)}{m}}\|u_Z\|_2 \|u_Q\|_2 \right) \leq c_3mn \|u\|_2^2,
\end{align*}
which implies $c_1n \leq \sigma(X^\top \Sigma_a^{-1} X) \leq c_2mn$. 

For $q>c_0m$: Since $\frac{\log^2(n)}{mn} = o(1)$, we have 
\begin{align*}
& c_1\frac{nm}{q} \|u\|_2^2 \leq c_2 \left( \frac{nm}{q} \|u_Z\|^2_2 + \frac{nm}{q}\|u_Q\|_2^2 - \sqrt{\frac{n\log(n)\left(1 \wedge \frac{m\log(n)}{q}\right)}{q}}\|u_Z\|_2 \|u_Q\|_2 \right) \\
& \leq u^\top X^\top \Sigma_a^{-1} X u \\
    & \leq c_2 \left( \frac{nm}{q} \|u_Z\|^2_2 + \frac{nm}{q} \|u_Q\|_2^2 + \sqrt{\frac{n\log(n)\left(1 \wedge \frac{m\log(n)}{q}\right)}{q}}\|u_Z\|_2 \|u_Q\|_2 \right) \leq c_3\frac{nm}{q} \|u\|_2^2,
\end{align*}
which implies $\sigma(X^\top \Sigma_a^{-1} X) \asymp nm/q$.
}
\\

\textit{Lemma \ref{lemma:A.3}.\ref{lemma:A.3.2})}
{
$\left.\right.$

As discussed in the proof of Lemma \ref{lemma:A.3}.\ref{lemma:A.3.1}, without loss of generality, we can let $\Sigma^i_X = I_p$, $\Sigma^i_Z = I_q$. 

When $p=q$: $X^i=Z^i$ for $i=1, \dots, n$. Then based on the singular value decomposition $Z^i = U^i D^i V^i$ with $D^i=\diag\left(\{\sigma_l(Z^i)\}_{l=1}^m\right)$, we have:
\begin{align}
    & \max_i \sigma\left((X^i)^\top (\Sigma_a^i)^{-1} X^i \right)  = \max_i \sigma\left( \left(aZ^i(Z^i)^\top +1 \right)^{-1}Z^i (Z^i)^\top \right) \nonumber \\
    & = \max_i \sigma\left( U^i (a(D^i)^2+I_m)^{-1} (U^i)^\top U^i (D^i)^2 (U^i)^\top \right) \nonumber \\
    & \leq \max_{i,l} \frac{\sigma_l^2(Z^i)}{a\sigma_l^2(Z^i) +1} \leq \frac{1}{a}. \label{a.3.2.1}
\end{align}

When $p>q$: Following the proof of Lemma \ref{lemma:A.3}.\ref{lemma:A.3.1} (the case when $p>q$), denoting $X^i = (Z^i, Q^i)$ and $u = (u_Z^\top, u_Q^\top)^\top$, we have
\begin{align}
    u^\top (X^i)^\top (\Sigma_a^i)^{-1} X^i u & = u_Z^\top (Z^i)^\top (\Sigma_a^i)^{-1} Z^i u_Z \label{e.a.3.2.1} \\
    & \quad + u_Q^\top (Z^i)^\top (\Sigma_a^i)^{-1} Q^i u_Q \label{e.a.3.2.2} \\
    & \quad + 2u_Z^\top (Z^i)^\top (\Sigma_a^i)^{-1} Q^i u_Q \label{e.a.3.2.3}.
\end{align}

\begin{enumerate}
    \item For \eqref{e.a.3.2.1}: $u_Z^\top (Z^i)^\top (\Sigma_a^i)^{-1} Z^i u_Z \leq \|u_Z\|^2_2 \sigma_{\max}\left((Z^i)^\top (\Sigma_a^i)^{-1} Z^i\right) \leq c_1 \|u_Z\|^2_2 $, where we have used the inequality $\sigma_{\max}\left((Z^i)^\top (\Sigma_a^i)^{-1} Z^i\right) \leq c_1$ based on \eqref{a.3.2.1}.
    \item For \eqref{e.a.3.2.2}: Hanson-Wright inequality gives 
    \begin{align*}
        & \P\left(\forall \ i, \left| u_Q^\top (Z^i)^\top (\Sigma_a^i)^{-1} Q^i u_Q - \tr\left((\Sigma_a^i)^{-1}\right) \|u_Q\|^2_2\right| \bigm| Z^i \right) \\
        & \leq 2\exp\left\{\log(n) - c_1\min\left(\frac{t^2}{\max_i\|u_Q\|^4_2 \|(\Sigma_a^i)^{-1}\|_F^2}, \frac{t}{\max_i \|u_Q\|^2_2 \|(\Sigma_a^i)^{-1}\|_2}\right)\right\}
    \end{align*}
    where by Lemma \ref{lemma:A.1}.\ref{lemma:A.1(6.3)} and Lemma \ref{lemma:A.1}.\ref{lemma:A.1(6.5)}:
    \begin{align*}
       & \|(\Sigma_a^i)^{-1}\|_2 \leq c_1\left(1 \wedge \frac{\log(n)}{m \vee q}\right),\\
       & \|(\Sigma_a^i)^{-1}\|_F^2 \leq \max_i \tr\left((\Sigma_a^i)^{-1}\right) \sigma_{\max}\left((\Sigma_a^i)^{-1}\right) \leq \begin{cases}
            c_1m\left(1 \wedge \frac{\log(n)}{q}\right)^2 &, q>c_0m,\\
            c_1\left(m+q\left(1 \wedge \frac{\log(n)}{m}\right)\right)\left(1 \wedge \frac{\log(n)}{m}\right) &, m>c_0q,
        \end{cases} \\
        & \tr\left((\Sigma_a^i)^{-1}\right) \leq \begin{cases}
            c_1m\left(1 \wedge \frac{\log(n)}{q}\right) &, q>c_0m,\\
            c_1\left(m+q\left(1 \wedge \frac{\log(n)}{m}\right)\right) &, m>c_0q.
        \end{cases}
    \end{align*}
    Then with probability at least $1-6\exp\{-c\log(n)\}$, 
    \begin{align*}
        u_Q^\top (Z^i)^\top (\Sigma_a^i)^{-1} Q^i u_Q \leq \begin{cases}
            c_1 \|u_Q\|_2^2m\log(n)\left(1 \wedge \frac{\log(n)}{q}\right) &, q>c_0m,\\
            c_1 \|u_Q\|_2^2 \log(n)\left(m+q\left(1 \wedge \frac{\log(n)}{m}\right)\right) &, m>c_0q.
        \end{cases}
    \end{align*}
    \item For \eqref{e.a.3.2.3}: Since entries of $Q^i$ are i.i.d. realizations of a standard normal distribution, we have $u_Z^\top (Z^i)^\top (\Sigma_a^i)^{-1} Q^i u_Q$ following a normal distribution conditional on $Z^i$. Thus based on the tail bound of a Gaussian random variable, we have that:
    \begin{align*}
        & \P\left(\max_i\left|u_Z^\top (Z^i)^\top (\Sigma_a^i)^{-1} Q^i u_Q\right| > t \bigm|  Z^i\right) \leq 2\exp\left\{\log(n) - c_1 \frac{t^2}{\|u_Q\|^2_2 \max_i \left\|(\Sigma_a^i)^{-1} (Z^i)^\top u_Z\right\|_2^2} \right\} \\
        & \leq 2\exp\left\{\log(n) - c_1 \frac{t^2}{\|u_Q\|^2_2\|u_Z\|^2_2 \max_i \sigma_{\max}\left((Z^i)^\top(\Sigma_a^i)^{-1} Z^i\right) \sigma_{\max}\left((\Sigma_a^i)^{-1}\right)} \right\} \\
        & \leq 2\exp\left\{\log(n) - c_1 \frac{t^2}{\|u_Q\|^2_2\|u_Z\|^2_2 \max_i \left(1 \wedge \frac{\log(n)}{m\vee q}\right)} \right\} \quad \quad \text{(based on Lemma \ref{lemma:A.1}.\ref{lemma:A.1(6.3)})}.
    \end{align*}
    Then $\max_i\left|u_Z^\top (Z^i)^\top (\Sigma_a^i)^{-1} Q^i u_Q\right| \leq c_1 \|u_Q\|_2\|u_Z\|_2\sqrt{\log(n)\left(1 \wedge \frac{\log(n)}{m\vee q}\right)}$ with probability at least $1-4\exp\{-c\log(n)\}$.
\end{enumerate}
Based on the bounds of \eqref{e.a.3.2.1}, \eqref{e.a.3.2.2} and \eqref{e.a.3.2.3}, with probability at least $1-8\exp\{-c\log(n)\}$, we have that:
\begin{align*}
    u^\top (X^i)^\top (\Sigma_a^i)^{-1} X^i u & \leq c_1 \|u_Z\|^2_2  + c_1 \|u_Q\|_2\|u_Z\|_2\sqrt{\log(n)\left(1 \wedge \frac{\log(n)}{m\vee q}\right)} \\
    & \quad \quad + \begin{cases}
            c_1 \|u_Q\|_2^2m\log(n)\left(1 \wedge \frac{\log(n)}{q}\right) &, q>c_0m,\\
            c_1 \|u_Q\|_2^2 \log(n)\left(m+q\left(1 \wedge \frac{\log(n)}{m}\right)\right) &, m>c_0q.
        \end{cases} \\
    & \leq \begin{cases}
            c_1 \|u\|_2^2 \left(1 \vee \frac{m\log^2(n)}{q}\right) &, q>c_0m,\\
            c_1 \|u\|_2^2 m\log^2(n) &, m>c_0q.
        \end{cases}
\end{align*}
}
\end{proof}

\begin{proof}[Proof of Lemma \ref{lemma:A.2}]
$\left.\right.$

\textit{Lemma \ref{lemma:A.2}.\ref{lemma:A.2.1})}
{
$\left.\right.$

We can show that:
\begin{align*}
& \max_{1\leq j\leq p} \sum_{i=1}^n \left\|(Z^i)^\top \left(\Sigma_a^i\right)^{-1} X_j^i \right\|_2^2 \left\|\Psi\right\|_2 + \left\|\left(\Sigma_a^i\right)^{-1} X_j^i\right\|_2^2 \|R^i\|_2 \\
& = \max_{1\leq j\leq p} \sum_{i=1}^n e_j^\top (X^i)^\top \left(\Sigma_a^i\right)^{-1} Z^i (Z^i)^\top \left(\Sigma_a^i\right)^{-1} X^i e_j \left\|\Psi\right\|_2 + e_j^\top (X^i)^\top \left(\Sigma_a^i\right)^{-1}\left(\Sigma_a^i\right)^{-1} X^i e_j \|R^i\|_2\\
& \leq \max_j \max_i \|e_j\|^2_2 \sigma_{\max}\left(X^\top \Sigma_a^{-1}X \right) \left(\sigma_{\max}\left(\Sigma_a^{-1}\right) \|R^i\|_2 + \sigma_{\max}\left((Z^i)^\top \left(\Sigma_a^i\right)^{-1}Z^i\right) \|\Psi\|_2 \right) .
\end{align*}
We can bound $\sigma_{\max}(X^\top \Sigma_a^{-1}X)$ based on Lemma \ref{lemma:A.3}.\ref{lemma:A.3.1}. The remaining terms can be bound under Assumption \ref{as.A}.\ref{as.A.2} and using the results from Lemma \ref{lemma:A.1}.\ref{lemma:A.1(6.3)} and Lemma \ref{lemma:A.3}.\ref{lemma:A.3.2}:
\begin{align*}
    &\max_i \ \sigma_{\max}(\Sigma_a^{-1}) \|R^i\|_2 + \sigma_{\max}\left((Z^i)^\top \left(\Sigma_a^i\right)^{-1}Z^i\right) \|\Psi\|_2\\
    & \leq c_1 + c_2 \left(1 \wedge \frac{\log(n)}{m \vee q}\right)\\
    & \leq c_3,
\end{align*}
with probability at least $1-10\exp\{-c_4\log(n)\}$. Thus we have
\begin{align*}
    \max_{1\leq j\leq p} \sum_{i=1}^n \left\|(Z^i)^\top \left(\Sigma_a^i\right)^{-1} X_j^i \right\|_2^2 \left\|\Psi\right\|_2 + \left\|\left(\Sigma_a^i\right)^{-1} X_j^i\right\|_2^2 \|R^i\|_2 \leq \begin{cases}
            \frac{c_5mn}{q} &, q>c_0m,\\
            c_5n &, m>c_0q \text{ and } p=q,\\
            c_5mn &, m>c_0q \text{ and } q<p,
        \end{cases}
\end{align*}
with probability at least $1-4\exp\{-cn\} -12\exp\{-c\log(n)\} - 2\exp\{-cmnq^{-\qm}\} -\exp\left\{-cn\left(m/q\right)^{\qm} \right\}$.

When $q>c_0m$ and we additionally assume Assumption \ref{as.A.add}.\ref{as.A.3}: We have
\begin{align*}
    & \max_{1\leq j\leq p} \sum_{i=1}^n \left\|(Z^i_{S_\psi})^\top \left(\Sigma_a^i\right)^{-1} X_j^i \right\|_2^2 \left\|\Psi\right\|_2 + \left\|\left(\Sigma_a^i\right)^{-1} X_j^i\right\|_2^2 \|R^i\|_2 \\
    & = \max_{1\leq j\leq p} \sum_{i=1}^n e_j^\top (X^i)^\top \left(\Sigma_a^i\right)^{-1} Z^i_{S_\psi} (Z^i_{S_\psi})^\top \left(\Sigma_a^i\right)^{-1} X^i e_j \left\|\Psi\right\|_2 + e_j^\top (X^i)^\top \left(\Sigma_a^i\right)^{-1}\left(\Sigma_a^i\right)^{-1} X^i e_j \|R^i\|_2 \\
    &  \leq  \max_j \max_i \sum_{i=1}^n \|e_j\|_2^2 \sigma_{\max}\left(X^\top \Sigma_a^{-1} X \right) \sigma_{\max}\left(\Sigma_a^{-1}\right) \left( \sigma_{\max} \left( Z^i_{S_\psi} \left(Z^i_{S_\psi}\right)^\top \right)  \left\|\Psi\right\|_2 + \|R^i\|_2\right).
\end{align*}
Here, based on Lemma \ref{lemma:A.1}.\ref{lemma:A.1(4)}, $\max_i\sigma_{\max}\left( Z^i_{S_\psi} (Z^i_{S_\psi})^\top \right) \leq c_1m\log(n)$ with probability at least $1-2\exp\{-c\log(n)\}$ assuming $s_\psi \leq c_2m$ for some constant $c_2>0$ (Assumption \ref{as.A.add}.\ref{as.A.3}). Then plugging in the upper bound for $\sigma_{\max}\left(X^\top \Sigma_a^{-1} X\right)$ from Lemma \ref{lemma:A.3}.\ref{lemma:A.3.1}, and the upper bound for $\sigma_{\max}\left(\Sigma_a^{-1}\right)$ from Lemma \ref{lemma:A.1}.\ref{lemma:A.1(6.3)}, we obtain:
\begin{align*}
    \max_{1\leq j\leq p} \sum_{i=1}^n \left\|(Z^i_{S_\psi})^\top \left(\Sigma_a^i\right)^{-1} X_j^i \right\|_2^2 \left\|\Psi\right\|_2 + \left\|\left(\Sigma_a^i\right)^{-1} X_j^i\right\|_2^2 \|R^i\|_2 \leq \begin{cases}
            \frac{c_1m^2n\log^2(n)}{q^2} &, q>c_0m,\\
            c_1n\log^2(n) &, m>c_0q \text{ and } p=q,\\
            c_1mn\log^2(n) &, m>c_0q \text{ and } q<p.
        \end{cases}
\end{align*}
Since we also have
\begin{align*}
    & \max_{1\leq j\leq p} \sum_{i=1}^n \left\|(Z^i_{S_\psi})^\top \left(\Sigma_a^i\right)^{-1} X_j^i \right\|_2^2 \left\|\Psi\right\|_2 + \left\|\left(\Sigma_a^i\right)^{-1} X_j^i\right\|_2^2 \|R^i\|_2 \\
    & \leq   \max_{1\leq j\leq p} \sum_{i=1}^n \left\|(Z^i)^\top \left(\Sigma_a^i\right)^{-1} X_j^i \right\|_2^2 \left\|\Psi\right\|_2 + \left\|\left(\Sigma_a^i\right)^{-1} X_j^i\right\|_2^2 \|R^i\|_2,
\end{align*}
we take the smaller upper bounds and obtain:
\begin{align*}
    \max_{1\leq j\leq p} \sum_{i=1}^n \left\|(Z^i_{S_\psi})^\top \left(\Sigma_a^i\right)^{-1} X_j^i \right\|_2^2 \left\|\Psi\right\|_2 + \left\|\left(\Sigma_a^i\right)^{-1} X_j^i\right\|_2^2 \|R^i\|_2 \leq \begin{cases}
            \frac{c_1mn}{q}\left(1 \wedge \frac{m\log^2(n)}{q}\right) &, q>c_0m,\\
            c_1n &, m>c_0q \text{ and } p=q,\\
            c_1mn &, m>c_0q \text{ and } q<p,
        \end{cases}
\end{align*}
with probability at least $1-4\exp\{-cn\} -6\exp\{-c\log(n)\} - 2\exp\{-cmnq^{-\qm}\} -\exp\left\{-cn\left(m/q\right)^{\qm} \right\}$.
}
\\

\textit{Lemma \ref{lemma:A.2}.\ref{lemma:A.2.0})}
{
$\left.\right.$ 

Conditional on $X$, the random effect $\gamma_i$'s and the noise $\epsilon_i$'s are independent sub-Gaussian random vectors with parameters $c_1\|\Psi\|_2$ and $c_2\|R^i\|_2$. Thus for fixed vectors $u_i$, $i=1, \dots, n$, we have $\sum_{i=1}^n u_i^\top Z^i\gamma_i + u_i^\top \epsilon_i \mid X \in \SG \left(c_3\sum_{i=1}^n  \| (Z^i)^\top u_i\|_2^2 \|\Psi\|_2 + \|u_i\|_2^2\|R^i\|_2 \right)$. Then conditional on $X$, letting $u_i = \left(\Sigma_a^i\right)^{-1} X^i_j$, we have $z_0^* = \max_j (\tr(\Sigma_a^{-1}))^{-1}\sum_{i=1}^n u_i^\top Z^i\gamma_i + u_i^\top \epsilon_i$. We thus have the following inequality based on the tail bound for sub-Gaussian random variables:
\begin{align*}
    \P\left( z_0^* > t \mid X\right) \leq 2\exp\left\{ \log(p) - c\frac{t^2 \tr^2(\Sigma_a^{-1})}{\max_j \sum_{i=1}^n \|(Z^i)^\top (\Sigma_a^i)^{-1} X^i_j \|_2^2\|\Psi \|_2 + \|(X^i_j)^\top (\Sigma_a^i)^{-1} \|_2^2 \|R^i\|_2 }\right\}.
\end{align*}
Let $t = c_1 (\tr(\Sigma_a^{-1}))^{-1}\sqrt{\log(p) \max_j \sum_{i=1}^n \|(Z^i)^\top (\Sigma_a^i)^{-1} X^i_j \|_2^2\|\Psi \|_2 + \|(X^i_j)^\top (\Sigma_a^i)^{-1} \|_2^2 \|R^i\|_2 }$. Then using Lemma \ref{lemma:A.2}.\ref{lemma:A.2.1} and the bound for $\tr(\Sigma_a^{-1})$ from Lemma \ref{lemma:A.1}.\ref{lemma:A.1(6.5)}, we obtain the following bounds for $z_0^*$ with probability at least $1-4\exp\{-cn\} -12\exp\{-c\log(n)\} - 2\exp\{-cmnq^{-\qm}\} -\exp\left\{-cn\left(m/q\right)^{\qm} \right\}$:
\begin{align*}
    z_0^* \leq \begin{cases}
        c_1 \sqrt{\frac{q\log(p)}{nm}} &, q>c_0m ,\\
        c_1 \sqrt{\frac{\log(p)}{nm^2}} &, m>c_0q \text{ and } p=q ,\\
        c_1 \sqrt{\frac{\log(p)}{nm}} &, m>c_0q \text{ and } p>q .
    \end{cases}
\end{align*}

When we additionally assume Assumption \ref{as.A.add}.\ref{as.A.3}, the structure of $\Psi$ implies $\gamma_{i, S_\psi} = 0$. Thus $y-X\beta^* = \sum_{i=1}^n Z^i_{S_\psi} \gamma_{i, S_\psi} + \epsilon_i$, where $\gamma_{i, S_\psi} \in \SGV(c_1\|\Psi\|_2)$. Then following the same arguments as above, using the tail bound for sub-Gaussian random variables, and using the results in Lemma \ref{lemma:A.2}.\ref{lemma:A.2.1}, we have $t = O_p\left(\sqrt{\frac{q\log(p)}{mn}\left(1 \wedge \frac{m\log^2(n)}{q}\right)}\right)$, with probability at least
\[1-4\exp\{-cn\} -6\exp\{-c\log(n)\} - 2\exp\{-cmnq^{-\qm}\} -\exp\left\{-cn\left(m/q\right)^{\qm} \right\}. \]
Thus under Assumption \ref{as.A.add}.\ref{as.A.3}, we obtain:
    \begin{align*}
        z_0^* \leq \begin{cases}
        c_1 \sqrt{\frac{\log(p)\log^2(n)}{n}} &, q>c_0m,\\
        c_1 \sqrt{\frac{\log(p)}{nm^2}} &, m>c_0q \text{ and } p=q ,\\
        c_1 \sqrt{\frac{\log(p)}{nm}} &, m>c_0q \text{ and } p>q .\\
        \end{cases}
    \end{align*}
}
\end{proof}

\section{Inference Framework for $\beta$}
\label{S:B}

\begin{assumption}
\label{as.B}
\begin{enumerate}
    \item \label{as.B.1} $\log(p) = o(mn)$. $\forall \ j =1, \dots, p$, conditional on $X^i_{-j}$, the random vector $X^i_j$ has mean $X^i_{-j} \kappa_j^*$ for $\kappa_j^* \in \R^{p-1}$ and variance $G_j$, and $X^i_j - X^i_{-j} \kappa_j^* \mid X^i_{-j} \in \SGV( c_1\|G_j\|_2)$. The support for $\kappa_j^*$ is $H_j$ and its cardinality is $|H_j|$. Assume $\|\kappa_j^*\|_1 \leq c_1|H_j|$. 
    \item \label{as.B.2}  $ \frac{\|G_j\|_2}{\sigma_{\min}(G_j)} \log(n) \sqrt{1\wedge \frac{\log(n)}{m \vee q}} \leq c_1  \sqrt{mnq^{-\qm}}$ %% this assumption ensures $\|w_j\|_2^2$ has a meaningful lower bound
    
    \item \label{as.B.3}
    \begin{enumerate}
        \item When $q>c_0m$, $p=q$:
        \begin{align}
        &\frac{|H_j|q^2\log(p)}{m^3n} \ll \|G_j\|_2 \leq c_1 \frac{mn}{\log(n)\log(p)} \label{as.b.3.e1} \\
        &\frac{\|G_j\|_2}{\sigma_{\min}^2(G_j)} \ll \frac{mn}{|H_j|^3\log(n)\log(p)} \wedge \frac{m^2n^2}{s^2|H_j|q\log(n)\log^2(p)} \label{as.b.3.e2} \\
        &\frac{\|G_j\|_2}{\sigma_{\min}(G_j)} \ll \frac{mn}{|H_j|\log(n)\log(p)} \label{as.b.3.e3}
        \end{align}

        \item when $q>c_0m$, $p>q$: assume the conditions \eqref{as.b.3.e1}--\eqref{as.b.3.e3}, and additionally assume $\|G_j\|_2 \gg \frac{|H_j|\log(p)\log^3(n)}{mn}$    
        \item When $m>c_0q$:
        \begin{align*}
        &\frac{|H_j|\log(p)}{m^3n} \left({ m^3\log^5(n) }\right)^{\mathbf{1}\{p>q\}} \ll \|G_j\|_2 \leq c_1 \frac{mn}{\log(p)} \left(\frac{1}{m\log(n)}\right)^{\mathbf{1}\{p>q\}}\\
        &\frac{\|G_j\|_2}{\sigma_{\min}^2(G_j)} \ll \left(\frac{m^3n}{|H_j|^3\log(p)} \left(\frac{1}{m\log^2(n)}\right)^{\mathbf{1}\{p>q\}} \right) \wedge \left(\frac{m^3n^2}{s^2|H_j|\log^2(p)} \left(\frac{1}{m^2\log^2(n) }\right)^{\mathbf{1}\{p>q\}} \right)\\
        &\frac{\|G_j\|_2}{\sigma_{\min}(G_j)} \ll \frac{m^2n}{|H_j|\log(p)} \left(\frac{1}{m\log(n)}\right)^{\mathbf{1}\{p>q\}}
        \end{align*}
        
        % \item When $m>c_0q$, $p=q$:
        %         \begin{align*}
        %     &\frac{|H_j|\log(p)}{m^3n} \ll \|G_j\|_2 \leq c_1 \frac{mn}{\log(p)}\\
        %     &\frac{\|G_j\|_2}{\sigma_{\min}^2(G_j)} \ll \frac{m^3n}{|H_j|^3\log(p)} \wedge \frac{m^3n^2}{s^2|H_j|\log(p)}\\
        %     &\frac{\|G_j\|_2}{\sigma_{\min}(G_j)} \ll \frac{m^2n}{|H_j|\log(p)}
        % \end{align*}
        % \item When $m>c_0q$, $p>q$:
        %         \begin{align*}
        %     &\frac{|H_j|\log(p)\log^5(n)}{n} \ll \|G_j\|_2 \leq c_1 \frac{n}{\log(n)\log(p)}\\
        %     &\frac{\|G_j\|_2}{\sigma_{\min}^2(G_j)} \ll \frac{m^2n}{|H_j|^3\log^2(n)\log(p)} \wedge \frac{mn^2}{s^2|H_j|\log^2(n)\log^2(p)}\\
        %     &\frac{\|G_j\|_2}{\sigma_{\min}(G_j)} \ll \frac{mn}{|H_j|\log(n)\log(p)}
        % \end{align*}
    \end{enumerate}
\end{enumerate}
\end{assumption}

\begin{assumption}
    \label{as.B.4}
    \begin{enumerate}
        \item \label{cond1} Condition 1: When Assumption \ref{as.A.add}.\ref{as.A.3.2} holds:
    \begin{align*}
        \begin{cases}
          \frac{\|G_j\|_2}{\sigma_{\min}(G_j)}  \ll \frac{n}{\log^6(n)}  &,\ q>c_0m\\
          \frac{\|G_j\|_2}{\sigma_{\min}(G_j)} \ll \frac{n}{\log^5(n)}  &,\ m>c_0q
        \end{cases}
    \end{align*}
        \item \label{cond2} Condition 2: When Assumption \ref{as.A.add}.\ref{as.A.3} holds and $j \in S_\psi$:
        \begin{align*}
        \begin{cases}
          \frac{\|G_j\|_2}{\sigma^2_{\min}(G_j)} \ll \frac{n}{\log^6(n)}  &,\ q>c_0m\\
          \frac{\|G_j\|_2}{\sigma^2_{\min}(G_j)} \ll \frac{mn}{\log^5(n)}  &,\ m>c_0q
        \end{cases}
    \end{align*}
        \item \label{cond3} Condition 3: When Assumption \ref{as.A.add}.\ref{as.A.3} holds and $j \not\in S_\psi$:
        \begin{align*}
        \begin{cases}
         \frac{\|G_j\|_2}{\sigma_{\min}(G_j)} \ll \frac{n}{s_\psi\log^7(n)} \wedge \frac{n^2}{s_\psi|H_j|^2\log(p)\log^8(n)} \wedge \frac{n}{\log^6(n)}   &,\ q>c_0m\\
         \frac{\|G_j\|_2}{\sigma_{\min}(G_j)} \ll \frac{mn^2}{s_\psi|H_j|^2\log(p)\log^7(n)} \wedge \frac{n}{\log^5(n)}   &,\ m>c_0q,\ p=q\\
         \frac{\|G_j\|_2}{\sigma_{\min}(G_j)} \ll \frac{n^2}{s_\psi|H_j|^2 \log(p)\log^8(n)} \wedge \frac{n}{\log^5(n)}   &,\ m>c_0q,\ p>q
        \end{cases}
    \end{align*}

\end{enumerate}
\end{assumption}

\begin{lemma}
\label{lemma:sigma-theta}
For $\Sigma_{\theta}^i = Z^i \Psi (Z^i)^\top + R^i$, $i \in \{1, \dots, n\}$, under Assumption~\ref{as.A}, with probability at least $1-c_1\exp\{-c_2m\}$, we have:
\begin{enumerate}
    \item When $m>c_0q$: Under either Assumption \ref{as.A.add}.\ref{as.A.3} or Assumption \ref{as.A.add}.\ref{as.A.3.2}, 
    \begin{align*}
        c_3 \leq \sigma_{\min}(\Sigma_{\theta}^i) \leq \sigma_{\max}(\Sigma_{\theta}^i) \leq c_4 m.
    \end{align*}
    
    \item When $q>c_0m$: Under Assumption \ref{as.A.add}.\ref{as.A.3.2},  
    \begin{align*}
    \sigma_{\min}(\Sigma_{\theta}^i) \asymp \sigma_{\max}(\Sigma_{\theta}^i) \asymp q.
    \end{align*}
    Under Assumption \ref{as.A.add}.\ref{as.A.3},
    \begin{align*}
    c_5 \leq \sigma_{\min}(\Sigma_{\theta}) \leq \sigma_{\max}(\Sigma_{\theta}) \leq c_6 m.
    \end{align*}
\end{enumerate}

\end{lemma}

\begin{theorem}
\label{thm:S2}
Under Assumption \ref{as.A}, Assumption \ref{as.B} and Assumption~\ref{as.B.4}, with probability at least $1-c_1\exp\{-cn\} -c_2\exp\{-c\log(n)\} - c_3\exp\{-cmnq^{-\qm}\} -c_4\exp\left\{-cn\left(m/q\right)^{\qm} \right\} -c_5\exp\{-c\log(p)\} - c_6\exp\{-cmn\}$, we have that
\begin{align*}
    &\frac{1}{\sqrt{V_j}}\left(\hat\beta_j^{(db)} - \beta_j^*\right) = R_j + o_p(1), \quad \text{where } R_j \xrightarrow[]{d} N(0,1),
\end{align*}
where the variance $V_j$ is given by
\begin{align*}
     V_j = \frac{ \sum_{i=1}^n (\hat w^i_j)^\top (\Sigma_b^i)^{-1/2}\Sigma_{\theta^*}^i (\Sigma_b^i)^{-1/2} \hat w^i_j}{ \left| \sum_{i=1}^n (\hat w^i_j)^\top (\Sigma_b^i)^{-1/2} X^i_j \right|^2}.
\end{align*}
\end{theorem}

\subsection{Related lemmas for Theorem \ref{thm:S2}}
\label{S:B.1}

\begin{lemma}
\label{lemma:b.3}
$\left.\right.$
\begin{enumerate}
    \item \label{lemma:b.3.2}
    Define 
    \begin{align}
    z_j^* :=  \frac{1}{\tr(\Sigma_b^{-1})}\left\| X^\top_{-j} \Sigma_b^{-1}(X_j-X_{-j}\kappa_j^*)\right\|_\infty. \label{def:zj*}
    \end{align}
    Under Assumption \ref{as.A} and Assumption \ref{as.B}.\ref{as.B.1}, with probability at least $1-2\exp\{-cmnq^{-\qm}\}-4\exp\{-c\log(n)\}-4\exp\{-cn\}-2\exp\{-c\log(p)\}-\exp\{-cn(m/q)^{\qm}\}$, we have that:
    \begin{align*}
        z_j^* \leq \begin{cases}
        c_1\sqrt{\frac{q \log(p) \|G_j\|_2}{m^2n}\left(1 \wedge  \frac{m\log(n)}{q}\right)} &, q>c_0m \text{ and } q=p,\\
        c_1  \sqrt{\frac{\log(p)\|G_j\|_2}{m^3n}}&, m>c_0q \text{ and }q=p,\\
        c_1 \sqrt{\frac{q\log(p) \|G_j\|_2}{mn}\left(1 \wedge  \frac{\log(n)}{q}\right)} &, q>c_0m \text{ and } q<p,\\
        c_1\sqrt{\frac{\log(p) \|G_j\|_2}{mn}\left(1 \wedge  \frac{\log(n)}{m}\right)} &, m>c_0q \text{ and }q<p.
        \end{cases}
    \end{align*}

    %% move the kappa results into Lemma b.3
    \item \label{lemma:b.2}
    Under Assumption \ref{as.A} and Assumption \ref{as.B}.\ref{as.B.1}, we have the following results with probability at least $1-c_1\exp\{-cn(m/q)^{\qm}\} - c_2\exp\{-cn\} - c_3\exp\{-c\log(n)\} - c_4 \exp\{-cmnq^{-\qm}\} - c_5 \exp\{-c\log(p)\}$:
    \begin{enumerate}
    \item When $q=p$ and $q>c_0m$: 
    $\lambda_j = c_6\sqrt{\frac{q\log(p) \|G_j\|_2}{m^2n}\left(1 \wedge  \frac{m\log(n)}{q}\right)}$ with suitably large $c_6>0$, and 
    \begin{align*}
        &\|\hat \kappa_j - \kappa_j^*\|_2  \leq c_7 \sqrt{\frac{|H_j|q\log(p)\|G_j\|_2}{m^2n}\left(1 \wedge  \frac{m\log(n)}{q}\right)},\\
        &\|\hat \kappa_j - \kappa_j^*\|_1  \leq c_7 |H_j| \sqrt{\frac{q \log(p) \|G_j\|_2}{m^2n}\left(1 \wedge  \frac{m\log(n)}{q}\right)},\\
        &\|\Sigma_b^{-1/2}X_{-j}(\hat \kappa_j - \kappa_j^*)\|_2^2  \leq c_7 |H_j| {\frac{\log(p)\|G_j\|_2}{m}\left(1 \wedge  \frac{m\log(n)}{q}\right)}.
    \end{align*}
    
    \item When $q=p$ and $m>c_0q$: 
        $\lambda_j = c_6\sqrt{\frac{\log(p)\|G_j\|_2}{m^3n}}$ with suitably large $c_6>0$, and 
        \begin{align*}
        &\|\hat \kappa_j - \kappa_j^*\|_2  \leq c_7 \sqrt{\frac{|H_j| \log(p)\|G_j\|_2}{mn}},\\
        &\|\hat \kappa_j - \kappa_j^*\|_1  \leq c_7 |H_j| \sqrt{\frac{ \log(p)\|G_j\|_2}{mn}},\\
        &\|\Sigma_b^{-1/2}X_{-j}(\hat \kappa_j - \kappa_j^*)\|_2^2  \leq c_7 |H_j| {\frac{\log(p)\|G_j\|_2}{m}}.
    \end{align*}
    
    \item When $q<p$ and $q>c_0m$: 
        $\lambda_j = c_6\sqrt{\frac{q\log(p)\|G_j\|_2}{mn}\left(1 \wedge  \frac{\log(n)}{q}\right)}$ with suitably large $c_6>0$, and 
        \begin{align*}
        &\|\hat \kappa_j - \kappa_j^*\|_2  \leq c_7 \sqrt{\frac{|H_j|q \log(p) \|G_j\|_2}{mn}\left(1 \wedge  \frac{\log(n)}{q}\right)},\\
        &\|\hat \kappa_j - \kappa_j^*\|_1  \leq c_7 |H_j| \sqrt{\frac{q \log(p) \|G_j\|_2}{mn}\left(1 \wedge  \frac{\log(n)}{q}\right)},\\
        &\|\Sigma_b^{-1/2}X_{-j}(\hat \kappa_j - \kappa_j^*)\|_2^2  \leq c_7 |H_j| {\log(p) \|G_j\|_2\left(1 \wedge  \frac{\log(n)}{q}\right)}.
    \end{align*}
    
    \item When $q<p$ and $m>c_0q$: 
        $\lambda_j = c_6\sqrt{\frac{\log(p)\|G_j\|_2}{mn}\left(1 \wedge  \frac{\log(n)}{m}\right)}$ with suitably large $c_6>0$, and 
        \begin{align*}
        &\|\hat \kappa_j - \kappa_j^*\|_2  \leq c_7 \sqrt{\frac{|H_j|m\log(p)\|G_j\|_2}{n}\left(1 \wedge  \frac{\log(n)}{m}\right)},\\
        &\|\hat \kappa_j - \kappa_j^*\|_1  \leq c_7|H_j| \sqrt{\frac{m \log(p) \|G_j\|_2}{n}\left(1 \wedge  \frac{\log(n)}{m}\right)},\\
        &\|\Sigma_b^{-1/2}X_{-j}(\hat \kappa_j - \kappa_j^*)\|_2^2  \leq c_7 {{m\log(p)\|G_j\|_2}\left(1 \wedge  \frac{\log(n)}{m}\right)}.
    \end{align*}
\end{enumerate}

    \item \label{lemma:b.3.1}
        Under Assumption \ref{as.A} and Assumption \ref{as.B}.\ref{as.B.1}, with probability at least $1-c_1\exp\{-cmnq^{-\qm}\}-c_2\exp\{-c\log(n)\}-c_3\exp\{-cn\}-c_4\exp\{-c\log(p)\}-c_5\exp\{-cn(m/q)^{\qm}\} - c_6\exp\{-cmn\}$, we have that:
        \begin{align*}
            \| X_{-j}^\top \Sigma_b^{-1} X_{-j} (\hat\kappa_j - \kappa_j^*) \|_\infty \leq \begin{cases}
        c_7 \sqrt{|H_j| \frac{n\log(p) \|G_j\|_2}{q} \left(1 \wedge \frac{m\log(n)}{q}\right)} &, q>c_0m \text{ and } q=p,\\
        c_7 \sqrt{|H_j| \frac{n\log(p)\|G_j\|_2}{m} } &, m>c_0q \text{ and } q=p,\\  
        c_7 \sqrt{|H_j| \frac{mn \log(p) \|G_j\|_2}{q} \left(1 \wedge \frac{\log(n)}{q}\right)} &, q>c_0m \text{ and } q<p,\\
        c_7 \sqrt{|H_j| n\log(p)\|G_j\|_2 \left(m \wedge \log(n)\right)^2} &, m>c_0q \text{ and } q<p,\\ 
            \end{cases}
        \end{align*}

    \item \label{lemma:b.3.3}
     Define 
     \begin{align*}
         w_j & = \Sigma_b^{-1/2}(X_j - X_{-j}\kappa_j^*)\\
         w^i_j & = (\Sigma_b^i){-\frac{1}{2}}(X_j^i - X_{-j}^i\kappa_j^*).
     \end{align*}
     Under Assumption \ref{as.A}, Assumption \ref{as.B}.\ref{as.B.1} and Assumption \ref{as.B}.\ref{as.B.2}, we have $c_1 \sigma_{\min}(G_j)nmq^{-\qm} \leq \|w_j\|_2^2 \leq c_2 \sigma_{\max}(G_j)nmq^{-\qm}$ with probability at least $1-4\exp\{-cn\}-2\exp\{-c\log(n)\}$, and 
    \begin{align*}
\max_i\|w^i_j\|_2^2 \leq \begin{cases}
c_1(m + \sqrt{m}\log(n)) \left( 1\wedge \frac{\log(n)}{q}\right) \|G_j\|_2 &, q>c_0m ,\\
c_1 \left( m + \log(n)\sqrt{  m \wedge {\log(n)}{} }\right) \|G_j\|_2 &, m>c_0q
\end{cases}
\end{align*}
     with probability at least $1-6\exp\{-c\log(n)\}$.
     
    \item \label{lemma:b.3.4}
      Under Assumption \ref{as.A}, Assumption \ref{as.B}.\ref{as.B.1}, Assumption \ref{as.B}.\ref{as.B.2}, and Assumption \ref{as.B}.\ref{as.B.3}, we have with probability at least $1-c_1\exp\{-cmnq^{-\qm}\}-c_2\exp\{-c\log(n)\}-c_3\exp\{-cn\}-c_4\exp\{-c\log(p)\}-c_5\exp\{-cn(m/q)^{\qm}\} - c_6\exp\{-cmn\}$ that 
      \begin{align*}
          |\hat w_j^\top \Sigma_b^{-1/2} X_j| \geq c_7\sigma_{\min}(G_j) nmq^{-\qm}.
      \end{align*}

    \item \label{lemma:b.3.7}    
    Under Assumption \ref{as.A} and Assumption \ref{as.B}, we have 
    \begin{align*}
        c_1 \sigma_{\min}(G_j) mn q^{-\qm} \leq \|\hat w_j\|^2_2 \leq c_2 \sigma_{\max}(G_j) nmq^{-\qm},
    \end{align*} 
    and 
    \begin{align*}
        \max_i \|\hat w_j^i\|_2^2 \leq \begin{cases}
        c_1 \left(m + \sqrt{m}\log(n)\right) \left( 1 \wedge \frac{\log(n)}{q}\right) \|G_j\|_2&, q>c_0m,\\
        c_1 \left(m+\log(n)\sqrt{m\wedge \log(n)}\right)\|G_j\|_2  &, m > c_0q,
        \end{cases}
    \end{align*}
    with probability at least $1-c_1\exp\{-cmnq^{-\qm}\}-c_2\exp\{-c\log(n)\}-c_3\exp\{-cn\}-c_4\exp\{-c\log(p)\}-c_5\exp\{-cn(m/q)^{\qm}\} - c_6\exp\{-cmn\}$.

    \item \label{lemma:b.3.6}
    Under Assumption \ref{as.A} and Assumption \ref{as.B}, with probability at least $1-c_1\exp\{-cmnq^{-\qm}\}-c_2\exp\{-c\log(n)\}-c_3\exp\{-cn\}-c_4\exp\{-c\log(p)\}-c_5\exp\{-cn(m/q)^{\qm}\} - c_6\exp\{-cmn\}$, we have the following results hold:
    \begin{enumerate}
        \item \label{lemma:b.3.6.c1} Under Condition \ref{cond1} defined in Assumption~\ref{as.B.4}, we have
        \begin{align*}
            & \max_i\left\|(\Sigma_{\theta^*}^i)^{1/2}(\Sigma_{b}^i)^{-1/2} \hat w^i_j\right\|^2_2 \leq \begin{cases}
            c_1 \left(m + \sqrt{m}\log(n)\right)\left(1 \wedge \frac{\log(n)}{q}\right)\log^2(n)\|G_j\|_2 &, q>c_0m,\\
            c_1 \left( m+\log(n)\sqrt{m\wedge \log(n)}\right) \log^2(n) \|G_j\|_2 &, m>c_0q,
            \end{cases}\\
            & \hat w_j^\top \Sigma_b^{-1/2} \Sigma_{\theta^*} \Sigma_b^{-1/2} \hat w_j \geq c_2 nm q^{-\qm} \sigma_{\min}(G_j).
        \end{align*}
        
        \item \label{lemma:b.3.6.c2} Under Condition \ref{cond2} defined in Assumption~\ref{as.B.4}, we have
        \begin{align*}
            & \max_i\left\|(\Sigma_{\theta^*}^i)^{1/2}(\Sigma_{b}^i)^{-1/2} \hat w^i_j\right\|^2_2 \leq \begin{cases}
            c_1 \left(m + \sqrt{m}\log(n)\right)\left(1 \wedge \frac{\log(n)}{q}\right)\log^2(n) \frac{m}{q}\|G_j\|_2 &, q>c_0m,\\
            c_1 \left( m+\log(n)\sqrt{m\wedge \log(n)}\right) \log^2(n) \|G_j\|_2 &, m>c_0q,
            \end{cases}\\
            & \hat w_j^\top \Sigma_b^{-1/2} \Sigma_{\theta^*} \Sigma_b^{-1/2} \hat w_j \geq c_2 nm^2 q^{-2\times \qm} \sigma_{\min}^2(G_j).
        \end{align*}
        
        \item \label{lemma:b.3.6.c3} Under Condition \ref{cond3} defined in Assumption~\ref{as.B.4}, we have
        \begin{align*}
            & \max_i\left\|(\Sigma_{\theta^*}^i)^{1/2}(\Sigma_{b}^i)^{-1/2} \hat w^i_j\right\|^2_2 \leq c_1\begin{cases}
          & s_\psi\frac{m\log^4(n)}{q^2}\|G_j\|_2  + s_\psi|H_j|^2\frac{m\log(p)\log^5(n)}{q^2n}\|G_j\|_2 + \frac{m\log^3(n)}{q^2}\|G_j\|_2  \\
           &\quad \quad \quad \quad \quad \quad \quad \quad \quad \quad \quad \quad \quad  \quad \quad \quad  \quad \quad \quad, q>c_0m,\\
          & s_\psi\frac{\log^2(n)}{m}\|G_j\|_2  + s_\psi|H_j|^2\frac{\log(p)\log^4(n)}{mn}\|G_j\|_2 + \log^2(n) \|G_j\|_2\\
           &\quad \quad \quad \quad \quad \quad \quad \quad \quad \quad \quad \quad \quad  \quad \quad \quad  \quad \quad \quad, m>c_0q,\ p=q,\\
         &  s_\psi\frac{\log^2(n)}{m}\|G_j\|_2  + s_\psi|H_j|^2\frac{\log(p)\log^5(n)}{n}\|G_j\|_2 + \log^2(n) \|G_j\|_2\\
           &\quad \quad \quad \quad \quad \quad \quad \quad \quad \quad \quad \quad \quad  \quad \quad \quad  \quad \quad \quad, m>c_0q,\ p>q
            \end{cases}\\
            & \hat w_j^\top \Sigma_b^{-1/2} \Sigma_{\theta^*} \Sigma_b^{-1/2} \hat w_j \geq \begin{cases}
           c_2\frac{nm\sigma_{\min}(G_j)}{q(q+\log(n))} &, q>c_0m,\\
           c_2\frac{nm\sigma_{\min}(G_j)}{m+\log(n)} &, m>c_0q,
            \end{cases}\\
        \end{align*}
        
    \end{enumerate}
    
\end{enumerate}
\end{lemma}

\begin{remark}
\label{Ssec:B.remark.relax.assumption}
If we only assume $\|\Psi\|_2 \leq c_1$ and do not restrict the structure of $\Psi$, we can still show 
\begin{align*}
& \max_i\left\|(\Sigma_{\theta^*}^i)^{1/2}(\Sigma_{b}^i)^{-1/2} \hat w^i_j\right\|^2_2 \leq c_1 m \log^3(n) \left( \log(n)/q\right) ^{\qm} \|G_j\|_2\\
& \hat w_j^\top \Sigma_b^{-1/2} \Sigma_{\theta^*} \Sigma_b^{-1/2} \hat w_j \geq c_2 nm q^{-\qm}  \sigma_{\min}(G_j) /(\log(n) + m \vee q)
\end{align*}
under Assumption \ref{as.A} and Assumption \ref{as.B}. Then Theorem \ref{thm:S2} still holds under the following additional assumption:
\begin{align*}
  m\log^6(n) \left(q\log(n)/m\right)^{\qm} \|G_j\|_2 \ll n\sigma_{\min}(G_j).
\end{align*}
\end{remark}

\newpage
 
\subsection{Proof of Theorem \ref{thm:S2}}
\begin{proof}

Denote $ \hat u = \hat \beta - \beta^*$ and $\hat v = \hat \kappa_j - \kappa_j^*$. Then we have:
\begin{align}
   \hat\beta^{(db)}_j - \beta_j^* &  = \hat\beta_j - \beta_j^* + \frac{\hat w_j^\top \Sigma_b^{-1/2} (y-X\hat\beta)}{\hat w_j^\top \Sigma_b^{-1/2}  X_{j}} \nonumber \\
    &  =  \left(e_j^\top - \frac{\hat w_j^\top \Sigma_b^{-1/2} X}{\hat w_j^\top \Sigma_b^{-1/2} X_j}\right) \hat u \label{thm2:r1} \\
    & \quad + \frac{\hat w_j^\top \Sigma_b^{-1/2} (y-X\beta^*)}{\hat w_j^\top \Sigma_b^{-1/2} X_j}. \label{thm2:r0}
\end{align}
In the following, we will show \eqref{thm2:r1} is $o_p(1)$, and \eqref{thm2:r0} is asymptotically normal. 

To show \eqref{thm2:r1} is $o_p(1)$: First note that
\begin{align*}
    \left(e_j^\top - \frac{\hat w_j^\top \Sigma_b^{-1/2} X}{\hat w_j^\top \Sigma_b^{-1/2} X_j}\right) \hat u
    & \leq \left\| e_j^\top - \frac{\hat w_j^\top \Sigma_b^{-1/2} X }{\hat w_j^\top \Sigma_b^{-1/2} X_j}\right\|_\infty \|\hat u\|_1 \\
    & = \frac{\left\| e_j^\top \hat w_j^\top \Sigma_b^{-1/2} X_j - \hat w_j^\top \Sigma_b^{-1/2} X \right\|_\infty}{ \left|\hat w_j^\top \Sigma_b^{-1/2} X_j \right|} \|\hat u\|_1 \\
    & = \frac{\left\|\hat w_j^\top \Sigma_b^{-1/2} X_{-j}\right\|_\infty\|\hat u\|_1}{|\hat w_j^\top \Sigma_b^{-1/2} X_j|},
\end{align*}
where 
\begin{align*}
\left\|\hat w_j^\top \Sigma_b^{-1/2} X_{-j}\right\|_\infty & = \| X_{-j}^\top \Sigma_b^{-1} (X_j - X_{-j}\hat\kappa_j) \|_\infty \nonumber\\
    & \leq \| X_{-j}^\top \Sigma_b^{-1} (X_j - X_{-j}\kappa_j^*) \|_\infty + \| X_{-j}^\top \Sigma_b^{-1} X_{-j}(\kappa_j^* - \hat\kappa_j) \|_\infty \nonumber\\
    & = z_j^* \tr(\Sigma_b^{-1}) + \| X_{-j}^\top \Sigma_b^{-1} X_{-j}\hat v \|_\infty 
\end{align*}
by the definition of $z_j^*$ in \eqref{def:zj*}. Then using Lemma \ref{lemma:A.1}.\ref{lemma:A.1(6.5)} to bound $\tr(\Sigma_b^{-1})$, Lemma \ref{lemma:b.3}.\ref{lemma:b.3.2} to bound $z_j^*$ and Lemma \ref{lemma:b.3}.\ref{lemma:b.3.1} to bound $\| X_{-j}^\top \Sigma_b^{-1} X_{-j}\hat v \|_\infty$, we have 
\begin{align*}
    & \left\|\hat w_j^\top \Sigma_b^{-1/2} X_{-j}\right\|_\infty \leq \begin{cases}
    c_1 \sqrt{|H_j|\frac{mn\log(p)\log(n)\|G_j\|_2}{q^2}}&, q>c_0m,\\
    c_1 \sqrt{|H_j|\frac{n\log(p)\|G_j\|_2}{m}}&, m>c_0q \text{ and } q=p,\\
    c_1 \sqrt{|H_j|n\log(p)\log^2(n)\|G_j\|_2}&, m>c_0 q \text{ and } q<p,
    \end{cases}
\end{align*}
with probability at least 
\[1-c_1\exp\{-cn\}-c_2\exp\{-c\log(n)\}-c_3\exp\{-cmnq^{-\qm}\} - c_4\exp\{-cn(m/q)^{-\qm}\} -c_5\exp\{-c\log(p)\}.\] 
Then using Lemma \ref{lemma:b.3}.\ref{lemma:b.3.4} to bound $|\hat w_j^\top \Sigma_b^{-1/2} X_j|$ and Theorem \ref{thm:S1} to bound $\|\hat u \|_1$, we can obtain the following bounds for \eqref{thm2:r1}:
\begin{align*}
     \left|\left(e_j^\top - \frac{\hat w_j^\top \Sigma_b^{-1/2} X}{\hat w_j^\top \Sigma_b^{-1/2} X_j}\right) \hat u \right| \leq \begin{cases}
    c_1 s \sqrt{|H_j|\frac{q\log^2(p)\log(n)\|G_j\|_2}{m^2n^2 \sigma_{\min}^2(G_j)}}&, q>c_0m,\\
    c_1 s \sqrt{|H_j|\frac{\log^2(p)\|G_j\|_2}{m^3n^2\sigma_{\min}^2(G_j)}}&, m>c_0q \text{ and } q=p,\\
    c_1 s \sqrt{|H_j|\frac{\log^2(p)\log^2(n)\|G_j\|_2}{mn^2\sigma_{\min}^2(G_j)}}&, m>c_0 q \text{ and } q<p.
     \end{cases},
\end{align*}
with probability at least $1-c_1\exp\{-cmnq^{-\qm}\}-c_2\exp\{-c\log(n)\}-c_3\exp\{-cn\}-c_4\exp\{-c\log(p)\}-c_5\exp\{-cn(m/q)^{\qm}\} - c_6\exp\{-cmn\}$. Moreover, under Assumption \ref{as.B}.\ref{as.B.3}, we have $\eqref{thm2:r1}=o_p(1)$.

Next we show that with random matrices $X^i$ and $Z^i$, the term \eqref{thm2:r0} is asymptotically normal. Note that conditional on $X$, the terms $\hat w_j$, $\Sigma_b$, $\Sigma_{\theta^*}$ are fixed quantities. Denote 
\begin{align*}
    \xi_i &= \frac{(\Sigma_{\theta^*}^i)^{1/2} (\Sigma_b^i)^{-1/2} \hat w^i_j}{\|\Sigma_{\theta^*}^{1/2} \Sigma_b^{-1/2} \hat w_j\|_2}, \quad 
    \tilde \epsilon_i  = (\Sigma_{\theta^*}^i)^{-1/2} (y^i-X^i\beta^*), \quad i=1, \dots, n
\end{align*}
and let $\xi$ and $\tilde \epsilon$ be the vectors formed by vertically stacking $\xi_i$'s and $\tilde \epsilon_i$'s, respectively. Then, $\|\xi\|_2^2=1$, $\E(\tilde \epsilon_i|X) = 0$, $\mathrm{Var}(\tilde \epsilon_i|X) = I_m$, and $\xi_i^\top \tilde \epsilon_i$ is independent of $\xi_j^\top \tilde \epsilon_j$ for $i\neq j$. Recalling that 
\begin{align*}
    V_j = \frac{\left\|\Sigma_{\theta^*}^{1/2} \Sigma_b^{-1/2} \hat w_j\right\|^2_2}{ \left|\hat w_j^\top \Sigma_b^{-1/2}X_j\right|^2},
\end{align*}
we have for the term \eqref{thm2:r0} that
\begin{align*}
    & \frac{1}{\sqrt{V_j}}\frac{\hat w_j^\top \Sigma_b^{-1/2} (y-X\beta^*)}{\hat w_j^\top \Sigma_b^{-1/2} X_j} = \sum_{i=1}^n \xi_i^\top \tilde \epsilon_i.
\end{align*}
In the following, we first use the Lyapunov Central Limit Theorem to show the (conditional) asymptotic normality of $\sum_{i=1}^n \xi_i^\top \tilde \epsilon_i$ given $X$, and then establish the unconditional asymptotic normality.

We need to verify the following three conditions for the Lyapunov Central Limit Theorem to hold:
\begin{enumerate}
    \item $\forall \  1 \leq i \leq n$, $\E(\xi_i \tilde \epsilon_i) < \infty$.
    \item $\forall \  1 \leq i \leq n$, $\mathrm{Var}(\xi_i \tilde \epsilon_i \mid X) < \infty$.
    \item Defining $s_n^2 = \sum_{i=1}^{n} \mathrm{Var}(\xi_i \tilde\epsilon_i \mid X)$, for some $\delta >0$, 
    \begin{align*}
        \lim_{n \xrightarrow{}\infty} \frac{1}{s_n^{2 + \delta}} \sum_{i=1}^{n} \E\left( \left| \xi_i \tilde \epsilon_i - \E(\xi_i \tilde \epsilon_i)\right|^{2+\delta}\mid X\right) =0.
    \end{align*}
\end{enumerate}
The first two conditions are trivially satisfied since $\E(\xi_i \tilde \epsilon_i) =0$ and $\mathrm{Var}(\xi^\top \tilde \epsilon \mid X)=1$. We show the third condition is satisfied at $\delta=2$. Because $\gamma_i$'s and $\epsilon_i$'s are independent sub-Gaussian vectors, the vectors $\tilde \epsilon_i$'s is also sub-Gaussian with parameter $c\asymp 1$. Then $\E(|\xi_i^\top \tilde\epsilon_i|^4) \leq 16\Gamma(2) \|\xi_i\|_2^4$ based on Proposition 3.2 in \cite{rivasplata2012subgaussian}. Thus, we have
\begin{align}
    \frac{1}{s_n^{4}} \sum_{i=1}^{n} \E\left( \left| \xi^\top_i \tilde \epsilon_i - \E(\xi^\top_i \tilde \epsilon_i)\right|^{4}\mid X\right) & = \sum_{i=1}^{n} \E\left( \left| \xi^\top_i \tilde \epsilon_i\right|^{4}\mid X\right)  \leq c_1 \sum_{i=1}^{n}\|\xi_i\|_2^4 \leq c_1 \max_i\|\xi_i\|_2^2 \times \|\xi\|_2^2 \nonumber\\
    & = c_1 \frac{\max_i\left\|(\Sigma_{\theta^*}^i)^{1/2} (\Sigma_b^i)^{-1/2} \hat w^i_j \right\|_2^2}{\left\|\Sigma_{\theta^*}^{1/2} \Sigma_b^{-1/2} \hat w_j\right\|_2^2}. \label{e.thm2.1}
\end{align}
Based on Lemma \ref{lemma:b.3}.\ref{lemma:b.3.6}, under Assumption \ref{as.B}.\ref{as.B.3} and Assumption~\ref{as.B.4}, with probability at least $1-c_1\exp\{-cmnq^{-\qm}\}-c_2\exp\{-c\log(n)\}-c_3\exp\{-cn\}-c_4\exp\{-c\log(p)\}-c_5\exp\{-cn(m/q)^{\qm}\} - c_6\exp\{-cmn\}$, we have $ \eqref{e.thm2.1} = o_p(\log^{-2}(n))$, and thus the third condition of the Lyapunov Central Limit Theorem is verified.

Notice that here we use a different approach from that in \cite{li2021inference} to show $\eqref{e.thm2.1} \ll 1$, and this difference is critical. \cite{li2021inference} directly assumes $\sigma_{\min}\left( \left(\Sigma_b^{i}\right)^{-1/2} \Sigma^{i}_{\theta} \left(\Sigma_b^{i}\right)^{-1/2}\right) \tr\left((\Sigma_a)^{-1} \right)\gg m\log(n)$ in order to bound $\eqref{e.thm2.1}$. However, under our settings, based on Lemma~\ref{lemma:A.1}, we can show that this assumption implies $n \gg p\log(n)$, which greatly restricts how fast $p$ can grow relative to $n$. Therefore, in our proof, we explicitly discuss the rate of the terms related to this assumption in Lemma~\ref{lemma:b.3}.\ref{lemma:b.3.6}. By imposing the structural assumptions on the matrix $\Psi$ in Assumption~\ref{as.A.add}, we establish the asymptotic normality of $\hat\beta^{(db)}_{j,k}$ with relatively mild sample size assumption. In particular, we allow $p$ to grow faster than $n$ and $m$.

Finally we show the unconditional asymptotic normality of the term \eqref{thm2:r0}:
Based on \cite{zahl1966bounds}, suppose we have a sequence of independent random variables $U_l$, $l=1, \dots, n, \dots$, with $\E(U_l)=\mu_l$, $\E(|U_l-\mu_l|^2)=\sigma^2_l$, $\E(|U_l-\mu_l|^3)=b_l$, $F_n(t)$ being the cumulative density function of the variable 
\begin{equation*}
    \frac{\sum_{l=1}^n(U_l-\mu_l)}{\sqrt{\sum_{l=1}^n \sigma_l^2}},
\end{equation*}
and $\Phi_0(t)$ being the cumulative density function of the standard normal distribution. Then,
\begin{align*}
    & \sup_t|F_n(t)-\Phi_0(t)| \leq c_1  \log(n) \frac{\sum_{l=1}^n b_l}{\sum_{l=1}^n \sigma_l^2\sqrt{\sum_{l=1}^n \sigma_l^2}}.
\end{align*}
In our case, for $l=1, \dots, n$, $U_l = \xi^\top_l\tilde \epsilon_l$, and we have $\mu_l=0$, $\sum_{l=1}^{n}\sigma_l^2=1$. Then we have: 
\begin{align*}
    & \sum_{l=1}^{n} \mathbb{E}(|U_l-\mu_l|^3|X)  \leq \sum_{l=1}^{n} \sqrt{\mathbb{E}(U_l^2|X) \mathbb{E}(U_l^4|X)} \quad \text{(Hoeffding's inequality)} \\
    & \leq \sqrt{\sum_{l=1}^{n}\mathbb{E}(U_l^2|X) \sum_{l=1}^{n}\mathbb{E}(U_l^4|X)} \quad \text{(Cauchy's inequality)} \\
    &  \leq \sqrt{\sum_{l=1}^{n}\|\xi_l\|_2^4}.
\end{align*}
As shown previously in \eqref{e.thm2.1}, under under Assumption \ref{as.B}.\ref{as.B.3} and Assumption~\ref{as.B.4}, we have $\sqrt{\sum_{l=1}^{n}\|\xi_l\|_2^4} = o_p\left(\log^{-1}(n)\right)$ for any $X$. Thus $\sup_t|F_n(t)-\Phi_0(t)| = o_p(1)$, indicating the unconditional asymptotic normality of $\xi^\top \tilde \epsilon$, i.e., the unconditional asymptotic normality of term \eqref{thm2:r0}.
\end{proof}

\subsection{Proof of related lemmas for Theorem \ref{thm:S2}}

\begin{proof}[Proof of Lemma \ref{lemma:sigma-theta}]
$\left.\right.$

First note that $\sigma_{\min}(\Psi)\sigma_{\min}\left( Z^i (Z^i)^\top \right) + \sigma_{\min}(R^i) \leq \sigma\left(\Sigma_{\theta}^i\right) \leq \|\Psi\|_2\sigma_{\max}\left( Z^i (Z^i)^\top \right) + \|R^i\|_2$. Using Lemma~\ref{lemma:A.1}.\ref{lemma:A.1(4)}, with probability at least $1-2\exp\{-cm\vee q\}$, we have
\begin{align*}
    &\sigma_{\min}\left( Z^i (Z^i)^\top \right) \geq \begin{cases}
    c_1 q &, \text{ if }q>c_0m, \\
    0 &, \text{ if } m>c_0q, 
    \end{cases}\\
    &\sigma_{\max}\left( Z^i (Z^i)^\top \right) \leq c_2 m \vee q.
\end{align*}
Then under Assumption~\ref{as.A} and Assumption~\ref{as.A.add}.\ref{as.A.3.2}, we have
\begin{align*}
\begin{cases}
c_3 \leq \sigma\left(\Sigma_{\theta}^i\right) \leq c_4m &, m>c_0q,\\
\sigma\left(\Sigma_{\theta}^i\right) \asymp q &, q>c_0m.
\end{cases}
\end{align*}
Under Assumption~\ref{as.A.add}.\ref{as.A.3}, note that we have $ \min(\psi_{S_\psi}) Z^i_{S_\psi} (Z^i_{S_\psi})^\top \preceq Z^i\Psi (Z^i)^\top \preceq \max(\psi_{S_\psi}) Z^i_{S_\psi} (Z^i_{S_\psi})^\top$ with $s_\psi < c_5m$. Thus, using Lemma~\ref{lemma:A.1}.\ref{lemma:A.1(4)}, with probability at least $1-2\exp\{-cm\}$, we have
\begin{align*}
    \sigma_{\max}\left( Z^i (Z^i)^\top \right) \leq c_6 m.
\end{align*}
Then under Assumption~\ref{as.A} and Assumption~\ref{as.A.add}.\ref{as.A.3}, for both cases of $q>c_0m$ and $m>c_0q$ we get
\begin{align*}
c_7 \leq \sigma\left(\Sigma_{\theta}^i\right) \leq c_8m.
\end{align*}

\end{proof}

\begin{proof}[Proof of Lemma \ref{lemma:b.3}]
$\left.\right.$

\textit{Lemma \ref{lemma:b.3}.\ref{lemma:b.3.2})}
{
$\left.\right.$

Recalling the definition of $z_j^*$ in \eqref{def:zj*}, we can rewrite the expression of $z_j^*$ as
\begin{align*}
z_j^* =  \frac{1}{\tr(\Sigma_b^{-1})} \max_{l \neq j, 1 \leq l \leq p}\left | X^\top_{l} \Sigma_b^{-1}(X_j-X_{-j}\kappa_j^*)\right |.
\end{align*}
Under Assumption \ref{as.B}.\ref{as.B.1} and using the tail bound of sub-Gaussian random variables, we can get
\begin{align}
    \P \left(z_j^* > t \mid X_{-j} \right) \leq 2 \exp \left\{\log(p) - c_1 \frac{t^2 {\tr}^2\left(\Sigma_b^{-1}\right)}{\|G_j\|_2\max_{l\neq j, 1\leq l \leq p} \|X^\top_l \Sigma_b^{-1} \|^2_2 }\right\}. \label{e.b.3.2.1}
\end{align}
For the term $\max_{l\neq j} \|X^\top_l \Sigma_b^{-1} \|^2_2$:
\begin{enumerate}
    \item When $l \leq q$, $l\neq j$: $X^i_l = Z^i_l$. Then by Lemma \ref{lemma:A.1}.\ref{lemma:A.1(9)},
    \begin{align*}
       \max_{l\neq j} \|X^\top_l \Sigma_b^{-1} \|^2_2 &\leq \sigma_{\max}\left(\sum_{i=1}^n \left(Z_{-j}^i \right)^\top \left(\Sigma_b^i\right)^{-2} Z_{-j}^i\right) \max_l\|e_l\|_2^2 \\
       & \leq \begin{cases}
       c_1 \frac{n}{q}\left(1 \wedge \frac{m\log(n)}{q}\right)&, q>c_0m,\\
       c_1\frac{n}{m}&, m>c_0q,
       \end{cases}
    \end{align*}
    with probability at least $1-2\exp\{-cn\} - 2\exp\{-c\log(n)\} - \exp\left\{-cn(m/q)^{\qm}\right\}$.
     
     \item When $l>q$, $l\neq j$: Since there exist a column $X_l$ with $l>q$, it implies that $p>q$. Then based on Lemma \ref{lemma:A.1}.\ref{lemma:A.1(6.3)} and Lemma \ref{lemma:A.3}.\ref{lemma:A.3.1}, we have
     \begin{align*}
         \max_{l\neq j} \|X^\top_l \Sigma_b^{-1} \|^2_2 &\leq \max_l\|e_l\|_2^2 \sigma_{\max}\left(X_{-j}^\top \Sigma_b^{-1} X_{-j}\right) \sigma_{\max}\left(\Sigma_b^{-1}\right) \\
         & \leq \begin{cases}
         c_2 \frac{mn}{q} \left( \frac{\log(n)}{q} \wedge 1\right) &, q>c_0m, \\
         c_2n(\log(n) \wedge m) &, m>c_0q,
         \end{cases}
     \end{align*}
     with probability at least $1-4\exp\{-cn\} - 4\exp\{-c\log(n)\} - \exp\{-cn(m/q)^{\qm}\} - 2\exp\{-cnmq^{-\qm}\}$.
\end{enumerate}
Combining the above two cases for $l \leq q$ and $l>q$, we obtain the following bounds:
\begin{align}
    \max_{l\neq j} \|X^\top_l \Sigma_b^{-1} \|^2_2 & \leq \begin{cases}
    c_1 \frac{n}{q}\left(1 \wedge \frac{m\log(n)}{q}\right)&, q>c_0m \text{ and } p=q,\\
       c_1\frac{n}{m}&, m>c_0q \text{ and } p=q, \\
        c_1 \frac{mn}{q} \left( \frac{\log(n)}{q} \wedge 1\right) &, q>c_0m \text{ and } p>q, \\
         c_1n(\log(n) \wedge m) &, m>c_0q \text{ and } p>q.
    \end{cases} \label{b.3.2.1.1}
\end{align}
Plugging \eqref{b.3.2.1.1} into \eqref{e.b.3.2.1} and taking $t = c_2  \sqrt{\log(p)\max_{l\neq j} \|X^\top_j \Sigma_b^{-1} \|^2_2 \|G_j\|_2}/{\tr(\Sigma_b^{-1})}$, we obtain the stated bounds for $z_j^*$ with probability at least $1-2\exp\{-cmnq^{-\qm}\}-4\exp\{-c\log(n)\}-4\exp\{-cn\}-2\exp\{-c\log(p)\}-\exp\{-cn(m/q)^{\qm}\}$.
} 
\\

\textit{Lemma \ref{lemma:b.3}.\ref{lemma:b.2})}
{
$\left.\right.$

Let $\hat v = \hat\kappa_j - \kappa_j^*$. Then based on the definition of $\hat\kappa_j$, we have 
\begin{align*}
    \frac{1}{2\tr\left(\Sigma_b^{-1}\right)} \left\|\Sigma_b^{-1/2} \left(X_j - X_{-j}\hat\kappa_j \right)\right\|^2_2 + \lambda_j \|\hat\kappa_j\|_1 \leq \frac{1}{2\tr\left(\Sigma_b^{-1}\right)} \left\|\Sigma_b^{-1/2} \left(X_j - X_{-j}\kappa^*_j \right)\right\|^2_2 + \lambda_j \|\kappa^*_j\|_1.
\end{align*}
Rearranging the terms, we get
\begin{align*}
    0 \leq \frac{1}{2\tr\left(\Sigma_b^{-1}\right)} \left\|\Sigma_b^{-1/2} X_{-j}\hat v \right\|^2_2 \leq (z_j^* +\lambda_j) \|\hat v_{H_j}\|_1 + (z_j^* -\lambda_j) \|\hat v_{H_j^c}\|_1 
\end{align*}
where $z_j^*$ is defined in \eqref{def:zj*}.
Based on Lemma \ref{lemma:A.3}.\ref{lemma:A.3.1}, we have $\left\|\Sigma_b^{-1/2} X_{-j}\hat v \right\|^2_2 \geq \|\hat v\|_2^2 \sigma_{\min}(X^\top_{-j} \Sigma_b^{-1} X_{-j}) \geq c_1 \|\hat v\|_2^2 n (m/q)^{\qm}$. Lemma \ref{lemma:b.3}.\ref{lemma:b.3.2} gives the upper bound for $z_j^*$. Then following the same arguments in the proof of Theorem \ref{thm:S1}, we can obtain the stated bounds with probability at least $1-c_1\exp\{-cn(m/q)^{\qm}\} - c_2\exp\{-cn\} - c_3\exp\{-c\log(n)\} - c_4 \exp\{-cmnq^{-\qm}\} - c_5 \exp\{-c\log(p)\}$.
}
\\

\textit{Lemma \ref{lemma:b.3}.\ref{lemma:b.3.1})}
{
$\left.\right.$

Let $\hat v = \hat\kappa_j  - \kappa_j^*$. Then we have:
\begin{align*}
    \max_{l\neq j}\left| X_{l}^\top \Sigma_b^{-1} X_{-j} \hat v\right| & \leq \max_{l\neq j} \|\Sigma_b^{-1/2} X_l\|_2 \|\Sigma_b^{-1/2} X_{-j} \hat v\|_2.
\end{align*}
We can first write
\begin{align*}
    \max_{l\neq j}\|\Sigma_b^{-1/2} X_l\|^2_2 & \leq \min \left( \max_{l\neq j} \|X_l\|_2^2 \sigma_{\max}\left(\Sigma_b^{-1}\right), \max_{l\neq j} \|e_l\|_2^2 \sigma_{\max}\left(X_{-j}^\top \Sigma_b^{-1}X_{-j}\right)\right) \\
    & \leq \begin{cases}
    c_1 \frac{nm}{q}&, q>c_0m,\\
    c_1 n(m \wedge \log(n)) &, m>c_0q \text{ and } q<p ,\\
    c_1 n &, m>c_0q \text{ and } q=p,
    \end{cases}
\end{align*}
where we have used Lemma \ref{lemma:A.1}.\ref{lemma:A.1(6.3)} to bound $\sigma_{\max}\left(\Sigma_b^{-1}\right)$, Lemma \ref{lemma:A.3}.\ref{lemma:A.3.1} to bound $\sigma_{\max}\left(X_{-j}^\top \Sigma_b^{-1}X_{-j}\right)$, and the tail bound for sum of square of independent Gaussian variables to bound $\max_{l\neq j}\|X_l\|_2^2$:
\begin{align*}
    \P\left(\max_l\left|\|X_l\|_2^2 - \sum_{i=1}^n m \left(\Sigma^i_X\right)_{l,l} \right| < c_2nm\right) > 1-2\exp\{ - cmn\} \quad \left(\text{under Assumption~\ref{as.B}.\ref{as.B.1} $\frac{\log(p)}{mn} =o(1)$}\right).
\end{align*} 
Then based on the bounds for $\|\Sigma_b^{-1/2} X_{-j} \hat v\|_2$ in Lemma \ref{lemma:b.3}.\ref{lemma:b.2}, we obtain the states bounds in the lemma, with probability at least $1-c_1\exp\{-cmnq^{-\qm}\}-c_2\exp\{-c\log(n)\}-c_3\exp\{-cn\}-c_4\exp\{-c\log(p)\}-c_5\exp\{-cn(m/q)^{\qm}\} - c_6\exp\{-cmn\}$.
}
\\

\textit{Lemma \ref{lemma:b.3}.\ref{lemma:b.3.3})}
{
$\left.\right.$

Conditioning on $X_{-j}$, we have $X_j - X_{-j}\kappa_j^* \in \SGV(c\|G_j\|_2)$ (Assumption~\ref{as.B}.\ref{as.B.1}). Then based on Corollary 2.8 of \cite{zajkowski2020bounds}, we can get:
\begin{align*}
    & \P\left( \left| \left\|w_j\right\|_2^2 - \E\left(\|w_j\|^2_2 \bigm| X_{-j}\right) \right| > t \mid X_{-j} \right) \leq 2\exp\left\{ -c_1\min\left( \frac{t^2}{\|\Sigma_b^{-1}\|_F^2 \|G_j\|_2^2},\frac{t}{\|\Sigma_b^{-1}\|_F \|G_j\|_2}\right) \right\}. 
\end{align*}
Here based on Lemma \ref{lemma:A.1}.\ref{lemma:A.1(6.3)} and Lemma \ref{lemma:A.1}.\ref{lemma:A.1(6.5)}, we have 
\begin{align*}
    & \E\left(\|w_j\|^2_2 \mid X_{-j}\right) =  \sum_{i=1}^n \tr\left((\Sigma_b^i)^{-1}G_j\right) \in [c_1 \sigma_{\min}(G_j) nm q^{-\qm}, c_2\sigma_{\max}(G_j) nm q^{-\qm}],\\
    & \|\Sigma_b^{-1}\|_F^2 = {\tr}^2(\Sigma_b^{-1}) \leq \|\Sigma_b^{-1}\|_2\tr(\Sigma_b^{-1}) \leq c_3 nm q^{-\qm}\left(1 \wedge \frac{\log(n)}{m \vee q}\right).
\end{align*}
Thus, under Assumption \ref{as.B}.\ref{as.B.2}, we have $\E\left(\|w_j\|^2_2 \mid X_{-j}\right) \geq c_1\log(n)\|\Sigma_b^{-1}\|_F \|G_j\|_2$ for suitably small $c_1>0$. Therefore, we get $ c_4 \sigma_{\min}(G_j) nm q^{-\qm} \leq \|w_j\|_2^2 \leq c_5\sigma_{\max}(G_j) nm q^{-\qm}$ with probability at least $1-4\exp\{-cn\}-2\exp\{-c\log(n)\}$.

For $w_j^i$, we similarly condition on $X_{-j}$ and use Corollary 2.8 of \cite{zajkowski2020bounds} to get
\begin{align}
        & \P\left(\forall \ i, \left| \left\|w^i_j\right\|_2^2 - \E\left(\left\|w^i_j\right\|^2_2 \mid X_{-j}\right) \right| > t \bigm| X_{-j}\right) \nonumber \\
    & \quad \quad  \leq 2\exp\left\{\log(n) -c_1\min\left( \frac{t^2}{\max_i\|(\Sigma_b^i)^{-1}\|_F^2 \|G_j\|_2^2},\frac{t}{\max_i\|(\Sigma_b^i)^{-1}\|_F \|G_j\|_2}\right) \right\}. \label{e.b.3.3.1}
\end{align}
Here, based on Lemma \ref{lemma:A.1}.\ref{lemma:A.1(6.3)} and Lemma \ref{lemma:A.1}.\ref{lemma:A.1(6.5)}, we have 
\begin{align*}
    & \E\left(\left\|w^i_j\right\|^2_2 \mid X_{-j}\right) = \tr\left((\Sigma_b^i)^{-1}G_j\right) \in  \begin{cases}
    c_1 m\left(1 \wedge \frac{\log(n)}{q}\right)\left[\sigma_{\min}(G_j), \sigma_{\max}(G_j)\right] &, q>c_0 m,\\
    c_1\left(m + q\left(1 \wedge \frac{\log(n)}{m}\right)\right)\left[\sigma_{\min}(G_j), \sigma_{\max}(G_j)\right] &, m>c_0q,
    \end{cases} \\
    & \|(\Sigma_b^i)^{-1}\|_F^2 = {\tr}^2((\Sigma_b^i)^{-1}) \leq \|(\Sigma_b^i)^{-1}\|_2\tr((\Sigma_b^i)^{-1})  \leq \begin{cases}
    c_2m\left(1 \wedge \frac{\log(n)}{q}\right)\left(1 \wedge \frac{\log(n)}{q}\right) &, q>c_0 m,\\
    c_2\left(m + q\left(1 \wedge \frac{\log(n)}{m}\right)\right)\left(1 \wedge \frac{\log(n)}{m}\right) &, m>c_0q,
    \end{cases}
\end{align*}

%\textcolor{red}{Here: double check this later; seems we do not need lower bound for $\|w_j^i\|$? Otherwise the assumption on lower bound is restrictive. For now just work on upper bound of $W^i_j$}

Then taking $t=c_3\log(n)\max_i\|(\Sigma_b^i)^{-1}\|_F \|G_j\|_2$ in \eqref{e.b.3.3.1}, we obtain
\begin{align*}
\max_i\|w^i_j\|_2^2 \leq \begin{cases}
c_1(m + \sqrt{m}\log(n)) \left( 1\wedge \frac{\log(n)}{q}\right) \|G_j\|_2 &, q>c_0m ,\\
c_1 \left( m + \sqrt{m \left( 1\wedge \frac{\log(n)}{m}\right)}\log(n)\right) \|G_j\|_2 &, m>c_0q
\end{cases}
\end{align*}
with probability at least $1-6\exp\{-c\log(n)\}$.
}
\\

\textit{Lemma \ref{lemma:b.3}.\ref{lemma:b.3.4})}
{
$\left.\right.$

Define $\hat v = \hat\kappa_j - \kappa_j^*$. Then $\hat w_j -w_j = -\Sigma_b^{-1/2}X_{-j}\hat v$, and by definition of $z_j^*$ we have $\|X_{-j}^\top \Sigma_b^{-1/2} w_j \|_\infty = z_j^* \tr(\Sigma_b^{-1})$. Thus we can write
\begin{align*}
    |\hat w_j^\top \Sigma_b^{-1/2} X_j|& =  |\hat w_j^\top \Sigma_b^{-1/2} (X_j - X_{-j}\kappa_j^* + X_{-j}\kappa_j^*| \\
    & \geq |\hat w_j^\top w_j| - |\hat w_j^\top \Sigma_b^{-1/2}  X_{\-j} \kappa_j^*| \\
    & \geq |w_j^\top w_j| - |(\hat w_j-w_j)^\top w_j| - |w_j^\top \Sigma_b^{-1/2}  X_{-j} \kappa_j^*| - |(\hat w_j-w_j)^\top \Sigma_b^{-1/2}  X_{-j} \kappa_j^*| \\
    &= \|w_j\|_2^2 - \|w_j^\top \Sigma_b^{-1/2} X_{-j} \hat v| -  \|w_j^\top \Sigma_b^{-1/2} X_{-j} \kappa_j^*| - \|\hat v^\top X_{-j}^\top \Sigma_b^{-1} X_{-j} \kappa_j^*| \\
    & \geq \|w_j\|_2^2 - z_j^* \tr\left(\Sigma_b^{-1}\right) \left( \|\hat v\|_1 + \|\kappa_j^*\|_1\right) - \|X_{-j}^\top \Sigma_b^{-1} X_{-j} \hat v \|_\infty \|\kappa_j^*\|_1.
\end{align*}
%% may not need the upper bound for this term

% We can similarly show that 
% \begin{align*}
%     |\hat w_j^\top \Sigma_b^{-1/2} X_j|& \leq \|w_j\|_2^2 + z_j^* \tr(\Sigma_b^{-1}) \left( \|\hat v\|_1 + \|\kappa_j^*\|_1\right) + \|X_{-j}^\top \Sigma_b^{-1} X_{-j} \hat v \|_\infty \|\kappa_j^*\|_1.
% \end{align*}

Then plugging in the bound for $\|\kappa_j^*\|$ from Assumption \ref{as.B}.\ref{as.B.1}, the bound for $z_j^*$ from Lemma \ref{lemma:b.3}.\ref{lemma:b.3.2}, the bound for $\|X_{-j}^\top \Sigma_b^{-1} X_{-j} \hat v \|_\infty$ from Lemma \ref{lemma:b.3}.\ref{lemma:b.3.1}, the bound for $\|w_j\|_2^2$ from Lemma \ref{lemma:b.3}.\ref{lemma:b.3.3}, the bound for $\|\hat v\|_1$ from Lemma \ref{lemma:b.3}.\ref{lemma:b.2}, and the bound for $\tr\left(\Sigma_b^{-1}\right)$ from Lemma \ref{lemma:A.1}.\ref{lemma:A.1(6.5)}, under Assumption \ref{as.B}:\ref{as.B.3}, we obtain 
\begin{align*}
    |\hat w_j^\top \Sigma_b^{-1/2} X_j| \geq c_1\sigma_{\min}(G_j) nmq^{-\qm}
\end{align*}
with probability at least $1-c_1\exp\{-cmnq^{-\qm}\}-c_2\exp\{-c\log(n)\}-c_3\exp\{-cn\}-c_4\exp\{-c\log(p)\}-c_5\exp\{-cn(m/q)^{\qm}\} - c_6\exp\{-cmn\}$.
}
\\

\textit{Lemma \ref{lemma:b.3}.\ref{lemma:b.3.7})}
{
$\left.\right.$

Define $\hat v = \hat\kappa_j - \kappa_j^*$. Then based on Lemma \ref{lemma:b.3}.\ref{lemma:b.2} and Lemma \ref{lemma:b.3}.\ref{lemma:b.3.3}, and under Assumption \ref{as.B}.\ref{as.B.3}, with probability at least $1-c_1\exp\{-cmnq^{-\qm}\}-c_2\exp\{-c\log(n)\}-c_3\exp\{-cn\}-c_4\exp\{-c\log(p)\}-c_5\exp\{-cn(m/q)^{\qm}\} - c_6\exp\{-cmn\}$ we have 
\begin{align}
    \|\hat w_j\|_2^2 & = \|w_j - \Sigma_b^{-1/2} X_{-j} \hat v\|_2^2  \geq \|w_j\|_2^2 - \|\Sigma_b^{-1/2} X_{-j} \hat v\|_2^2 \geq c_1 nmq^{-\qm} \sigma_{\min}(G_j), \label{b.3.7.1}\\
    \|\hat w_j\|_2^2 & \leq \|w_j\|_2^2 + \|\Sigma_b^{-1/2} X_{-j} \hat v\|_2^2\leq c_2 nmq^{-\qm} \sigma_{\max}(G_j) \label{b.3.7.2}.
\end{align}

For $\max_i\|\hat w_j^i\|_2^2$, we follow the similar arguments as \eqref{b.3.7.1} and \eqref{b.3.7.2} and have:
\begin{align*}
    \max_i\|\hat w_j^i\|_2^2 \leq \max_i\|w_j^i\|_2^2 + \|\hat v\|_2^2 \max_i \sigma_{\max}\left( \left(X^i_{-j}\right)^\top (\Sigma_b^i)^{-1} X^i_{-j} \right).
\end{align*}
Then, based on Lemma \ref{lemma:A.3}.\ref{lemma:A.3.2}, Lemma \ref{lemma:b.3}.\ref{lemma:b.2}, Lemma \ref{lemma:b.3}.\ref{lemma:b.3.3}, and under Assumption \ref{as.B}.\ref{as.B.3}, we have 
\begin{align*}
    \|\hat v\|_2^2 \max_i \sigma_{\max}\left( \left(X^i_{-j}\right)^\top (\Sigma_b^i)^{-1} X^i_{-j} \right) \ll \max_i\|w_j^i\|_2^2,
\end{align*}
and thus
\begin{align*}
        \max_i \|\hat w_j^i\|_2^2 \leq \begin{cases}
        c_1 (m+\sqrt{m}\log(n)) \left( 1 \wedge \frac{\log(n)}{q}\right) \|G_j\|_2 &, q>c_0m,\\
        c_1 \left(m + \log(n) \sqrt{m \wedge \log(n)}\right) \|G_j\|_2 &, m > c_0q,
        \end{cases}
    \end{align*}
    with probability at least $1-c_1\exp\{-cmnq^{-\qm}\}-c_2\exp\{-c\log(n)\}-c_3\exp\{-cn\}-c_4\exp\{-c\log(p)\}-c_5\exp\{-cn(m/q)^{\qm}\} - c_6\exp\{-cmn\}$.
}
\\

\textit{Lemma \ref{lemma:b.3}.\ref{lemma:b.3.6})}
{
$\left.\right.$

\begin{enumerate}
    \item For \ref{lemma:b.3}.\ref{lemma:b.3.6.c1}:
    Recall that $\Sigma_b^i = a Z^i_{-j} (Z^i_{-j})^\top + I_m$. We can show that with probability at least $1-c_1\log(n)$, we have 
    \begin{align*}
        \sigma_{\max}\left( \Sigma_{\theta^*}^i \left(\Sigma_b^i\right)^{-1}\right) & \leq \|\Psi\|_2 \sigma_{\max}\left((Z^i)^\top (\Sigma_b^i)^{-1} Z^i\right) + \|R^i\|_2 \sigma_{\max}\left((\Sigma_b^i)^{-1}\right) \\
        & \leq \begin{cases}
        \|\Psi\|_2 \sigma_{\max}\left((Z^i)^\top (\Sigma_a^i)^{-1} Z^i\right) + \|R^i\|_2 \sigma_{\max}\left((\Sigma_a^i)^{-1}\right) &, \text{if }j > q\\
        \|\Psi\|_2 \sigma_{\max}\left((Z_{-j}^i)^\top (\Sigma_b^i)^{-1} Z_{-j}^i\right) + \|R^i\|_2 \sigma_{\max}\left((\Sigma_b^i)^{-1}\right) \\
        \quad \quad \quad \quad \quad \quad \quad \quad + \|\Psi\|_2 (Z_{j}^i)^\top (\Sigma_b^i)^{-1} Z_{j}^i &, \text{if }j \leq q
        \end{cases} \\
         & \leq \begin{cases}
        c_2 &, \text{if }j > q\\
        c_2 +c_3 \|Z_{j}^i\|_2^2 \sigma_{\max}\left((\Sigma_b^i)^{-1}\right) &, \text{if }j \leq q
        \end{cases} \\
        & \leq \begin{cases}
       c_2 &, \text{if }j > q,\\
        c_2 + c_4m\log(n)\left(1 \wedge \frac{\log(n)}{m \vee q}\right) &, \text{if }j \leq q.
        \end{cases} \\
        & \leq c_5 \log^2(n)
        \end{align*}
where we have used Lemma \ref{lemma:A.1}.\ref{lemma:A.1(6.3)} to bound $\sigma_{\max}\left((\Sigma_b^i)^{-1}\right)$, Lemma~\ref{lemma:A.3}.\ref{lemma:A.3.2} to bound $\sigma_{\max}\left((Z^i)^\top (\Sigma_a^i)^{-1} Z^i\right)$ and $\sigma_{\max}\left((Z_{-j}^i)^\top (\Sigma_b^i)^{-1} Z_{-j}^i\right)$, with $\|\Psi\|_2 \asymp \|R^i\|_2 \asymp 1$ under Assumption~\ref{as.A}.\ref{as.A.2}, and the following tail bound for sub-Gaussian random variables: 
        \begin{align}
            \P \left(\max_i\left|\|Z_j^i\|_2^2 - m (\Sigma_Z^i)_{j,j} \right| < c_1 m\log(n) \mid \Sigma_Z^i \right) \geq 1-2\exp\{-c\log(n)\}. \label{eq.sum.x.square}
        \end{align}
        
We can also show that, under Assumption \ref{as.A.add}.\ref{as.A.3.2},
    \begin{align*}
        \sigma_{\min}\left( \Sigma_{\theta^*}^i (\Sigma_b^i)^{-1}\right) & \geq  \sigma_{\min}\left( \left(\sigma_{\min}(\Psi)(Z_{-j}^i)^\top  Z_{-j}^i + \sigma_{\min}(R^i) I_m\right)(\Sigma_b^i)^{-1}\right) \\
        & \geq c_1 \min_l \frac{\sigma_l^2(Z_{-j}^i) + c_2}{a\sigma_l^2(Z_{-j}^i) + 1} \\
        & \geq c_3.
    \end{align*}
Then, by Lemma \ref{lemma:b.3}.\ref{lemma:b.3.7}, we can show that
    \begin{align*}
        \hat w_j^\top \Sigma_b^{-1/2} \Sigma_{\theta^*} \Sigma_b^{-1/2} \hat w_j & \geq \|\hat w_j \|_2^2 \sigma_{\min}\left( \Sigma_{\theta^*}^i \left(\Sigma_b^i\right)^{-1}\right) \\
        & \geq c_1 nm q^{-\qm} \sigma_{\min}(G_j)\\
        \max_i\|(\Sigma_{\theta^*}^i)^{1/2}(\Sigma_{b}^i)^{-1/2} \hat w^i_j\|^2_2 
        & \leq \max_i\sigma_{\max}\left( \Sigma_{\theta^*}^i (\Sigma_b^i)^{-1}\right) \max_i \|\hat w_j^i \|_2^2 \\
        & \leq \begin{cases}
            c_1 (m +\sqrt{m}\log(n)) \left(1 \wedge \frac{\log(n)}{q}\right)\log^2(n) \|G_j\|_2 &, q>c_0m,\\
            c_1 (m + \log(n)\sqrt{m\wedge\log(n)})\log^2(n) \|G_j\|_2 &, m>c_0q,
            \end{cases}
    \end{align*}
     with probability at least $1-c_1\exp\{-cmnq^{-\qm}\}-c_2\exp\{-c\log(n)\}-c_3\exp\{-cn\}-c_4\exp\{-c\log(p)\}-c_5\exp\{-cn(m/q)^{\qm}\} - c_6\exp\{-cmn\}$.
    
    \item For \ref{lemma:b.3}.\ref{lemma:b.3.6.c2}:
    First note that based on the arguments in Lemma \ref{lemma:A.2}.\ref{lemma:A.2.1}: $\sigma_{\max}(Z^i_{S_\psi} (Z^i_{S_\psi})^\top) \leq c_1 m \log(n)$ with probability at least $1-2\exp\{-c\log(n)\}$. So we have
    \begin{align*}
    & \sigma_{\max}( (Z_{S_\psi}^i)^\top (\Sigma_b^i)^{-1} Z^i_{S_\psi}) \leq \sigma_{\max}(Z^i_{S_\psi} (Z^i_{S_\psi})^\top) \sigma_{\max}((\Sigma_b^i)^{-1}) \leq c_1\frac{m\log^2(n)}{m \vee q} \\
    & \sigma_{\max}\left( \Sigma_{\theta^*}^i (\Sigma_b^i)^{-1}\right) \leq \|\Psi\|_2\sigma_{\max}( (Z_{S_\psi}^i)^\top (\Sigma_b^i)^{-1} Z^i_{S_\psi}) + c_2\sigma_{\max}( (Z_{S_\psi}^i)^\top Z^i_{S_\psi}) \leq c_3\frac{m\log^2(n)}{m \vee q}.
    \end{align*}
    Then, based on Lemma \ref{lemma:b.3}.\ref{lemma:b.3.4}, we can show that
    \begin{align*}
        \max_i\|(\Sigma_{\theta^*}^i)^{1/2}(\Sigma_{b}^i)^{-1/2} \hat w^i_j\|^2_2 
        & \leq \max_i \sigma_{\max}\left( \Sigma_{\theta^*}^i (\Sigma_b^i)^{-1}\right) \max_i \|\hat w_j^i \|_2^2 \\
        & \leq \begin{cases}
            c_1 (m +\sqrt{m}\log(n)) \left(1 \wedge \frac{\log(n)}{q}\right)\log^2(n) \frac{m}{q} \|G_j\|_2 &, q>c_0m,\\
            c_1 (m + \log(n)\sqrt{m\wedge\log(n)})\log^2(n) \|G_j\|_2 &, m>c_0q.
            \end{cases}
    \end{align*}
    We can also write
    \begin{align*}
        \hat w_j^\top \Sigma_b^{-1/2} \Sigma_{\theta^*} \Sigma_b^{-1/2} \hat w_j &= \sum_{i=1}^n (\hat w_j^i)^\top (\Sigma_b^i)^{-1/2} \left( \sum_{l \in S_\psi} \psi_l Z^i_l (Z^i_l)^\top + R^i \right) (\Sigma_b^i)^{-1/2} \hat w_j^i\\
        & \geq c_1 \sum_{i=1}^n \left| (Z^i_l)^\top(\Sigma_b^i)^{-1/2} \hat w_j^i \right|^2 \\
        & \geq \frac{c_1}{n} \left|\sum_{i=1}^n (Z^i_l)^\top(\Sigma_b^i)^{-1/2} \hat w_j^i \right|^2 \quad \text{(Cauchy's inequality)}\\
        & \geq c_1 nm^2 q^{-2\times \qm} \sigma_{\min}^2(G_j). \quad \text{(Lemma~\ref{lemma:b.3}.\ref{lemma:b.3.4})}
    \end{align*}

    \item For \ref{lemma:b.3}.\ref{lemma:b.3.6.c3}:
    
    Using Lemma \ref{lemma:b.3}.\ref{lemma:b.3.7} and Lemma \ref{lemma:A.1}.\ref{lemma:A.1(6.4)}, we can show that 
    \begin{align*}
        \hat w_j^\top \Sigma_b^{-1/2} \Sigma_{\theta^*} \Sigma_b^{-1/2} \hat w_j & \geq  \sum_{i=1}^n (\hat w_j^i)^\top (\Sigma_b^i)^{-1/2}  R^i  (\Sigma_b^i)^{-1/2} \hat w_j^i\\
        & \geq c_1 \|\hat w_j\|_2^2 \sigma_{\min}\left(\Sigma_b^{-1}\right) \\
        & \geq c_1 nm q^{-\qm} \sigma_{\min}(G_j) \frac{1}{\log(n) + m \vee q}.
    \end{align*}
    Moreover, denoting $h_l^i = (\Sigma_b^i)^{-1}Z^i_l$, we can also show that 
    \begin{align}
         \max_i \| (\Sigma_{\theta^*}^i)^{1/2} (\Sigma_{b}^i)^{-1/2} \hat w_j^i\|_2^2 
         & \leq c_2 \max_i\|R^i\|_2 (\hat w_j^i)^\top (\Sigma_b^i)^{-1} \hat w_j^i + c_2 s_\psi \max_i \max_{l \in S_\psi} \left| (Z^i_l)^\top (\Sigma_b^i)^{-1/2} \hat w_j^i \right|^2 \nonumber \\
         & \leq c_3 \max_i (\hat w_j^i)^\top (\Sigma_b^i)^{-1} \hat w_j^i \label{e.b.3.6.0}\\
        &  \quad \quad + c_3s_\psi\max_i \max_{l \in S_\psi} \left| (h_l^i)^\top (X^i_j - X^i_{-j}\kappa_j^*) \right|^2  \label{e.b.3.6.1} \\ 
        & \quad \quad + c_3 s_\psi\max_i \max_{l \in S_\psi} \left|(h_l^i)^\top  X^i_{-j} \hat v \right|^2. \label{e.b.3.6.2} 
    \end{align}

To bound the term \eqref{e.b.3.6.0}: Based on Lemma \ref{lemma:A.1}.\ref{lemma:A.1(6.3)} and Lemma \ref{lemma:b.3}.\ref{lemma:b.3.7}, we can get
\begin{align*}
    \max_i (\hat w_j^i)^\top (\Sigma_b^i)^{-1} \hat w_j^i & \leq \max_i \sigma_{\max}((\Sigma_b^i)^{-1}) \|\hat w_j^i \|_2^2  \\
    & \leq \begin{cases}
    c_1 \left( 1\wedge \frac{\log(n)}{q}\right)^2 (m + \sqrt{m}\log(n)) \|G_j\|_2 &, q>c_0m, \\
    c_1 \left(1\wedge \frac{\log(n)}{m}\right) (m + \log(n)\sqrt{m\wedge \log(n)}) \|G_j\|_2 &, m>c_0q,
    \end{cases}
\end{align*}
with probability at least $1-c_1\exp\{-cmnq^{-\qm}\}-c_2\exp\{-c\log(n)\}-c_3\exp\{-cn\}-c_4\exp\{-c\log(p)\}-c_5\exp\{-cn(m/q)^{\qm}\} - c_6\exp\{-cmn\}$.

To bound the second term \eqref{e.b.3.6.1}: Conditioning on $X_{-j}$, under Assumption \ref{as.B}.\ref{as.B.1}, we have
\begin{align*}
   & (h_l^i)^\top (X_j^i -X_{-j}^i\kappa_j^*) \mid X_{-j} \in \SG(c\|h_l^i\|_2^2\|G_j\|_2)\\
    & \left|(h_l^i)^\top (X_j^i - X^i_{-j}\kappa^*_j) \right|^2 - (h_l^i)^\top G_j h^i_l \in \SE \left(c_1 \|h_l^i\|_2^4\|G_j\|^2_2, c_2\|h_l^i\|_2^2\|G_j\|_2\right).
\end{align*}
Then we have the following bound
\begin{align*}
    & \P\left( \max_i\max_{l \in S_\psi} \left|(h_l^i)^\top (X_j^i - X^i_{-j}\kappa^*_j) \right|^2 \leq t+  \max_i\max_{l \in S_\psi}\|G_j\|_2 \|h_l^i\|_2^2 \mid X_{-j}\right) \\
    & \quad \geq 1-2\exp\left\{\log(n) + \log(s_\psi) - c_1 \min \left( \frac{t^2}{\max_i\max_{  l \in S_\psi} \|G_j\|_2^2 \|h_l^i\|_2^4}, \frac{t}{\max_i\max_{ l \in S_\psi} \|G_j\|_2\|h_l^i\|_2^2}\right) \right\},
\end{align*}
where by Lemma \ref{lemma:A.1}.\ref{lemma:A.1(6.4)}
\begin{align}
    \max_i\max_{l \in S_\psi}\|h_l^i\|_2^2 & = \max_i\max_{ l \in S_\psi}(Z^i_l)^\top (\Sigma_b^i)^{-2} Z_l^i \nonumber \\
    & \leq \max_i \sigma_{\max}((\Sigma_b^i)^{-1})\sigma_{\max}\left((Z^i_{S_\psi})^\top (\Sigma_b^i)^{-1} Z_{S_\psi}^i\right) \nonumber \\
    & \leq c_1 \left(1\wedge \frac{\log(n)}{m \vee q} \left(\frac{m\log^2(n)}{q}\right)^{\qm} \right). \label{b.3.6.t1}
\end{align}
The last inequality \eqref{b.3.6.t1} holds because $\sigma_{\max}\left((Z^i_{S_\psi})^\top (\Sigma_b^i)^{-1} Z_{S_\psi}^i\right) \leq c_1 m\log^2(n)/(m\vee q)$ (shown in Lemma \ref{lemma:b.3}.\ref{lemma:b.3.6.c2}), and we also have $\sigma_{\max}\left((Z^i_{S_\psi})^\top (\Sigma_b^i)^{-1} Z_{S_\psi}^i\right) \leq \sigma_{\max}\left((Z^i_{-j})^\top (\Sigma_b^i)^{-1} Z_{-j}^i\right) \leq c$ by Lemma \ref{lemma:A.3}.\ref{lemma:A.3.2}.
Thus, we can bound the term \eqref{e.b.3.6.1} by $c_1 s_\psi \log(n) \left(1\wedge \frac{\log(n)}{m \vee q} \right) \left(\frac{m\log^2(n)}{q}\right)^{\qm}\|G_j\|_2$ with probability at least $1-4\exp\{-c\log(n)\}$.

We finally bound the term \eqref{e.b.3.6.2}. To this end, we use Lemma \ref{lemma:A.1}.\ref{lemma:A.1(6.4)}, Lemma \ref{lemma:b.3}.\ref{lemma:b.2}, and the tail bounds for $\|Z^i_{l_1}\|^2_2$, $\|X^i_{l_2}\|_2^2$ based on \eqref{eq.sum.x.square} to show that
\begin{align*}
    \max_i\max_{l \in S_\psi} \left|(h_l^i)^\top  X^i_{-j} \hat v \right|^2 & \leq \max_i\max_{l \in S_\psi} \left\| (Z^i_{l})^\top (\Sigma_b^i )^{-1} X^i_{-j} \right\|_\infty^2  \|\hat v\|_1^2 \\
    & = \max_i\max_{l_1 \in S_\psi, l_2 \in S_\psi} \left| (Z^i_{l_1})^\top (\Sigma_b^i )^{-1} X^i_{l_2} \right|^2  \|\hat v\|_1^2 \\
    & \leq \max_i\max_{l_1 \in S_\psi, l_2 \in S_\psi}  \|Z^i_{l_1}\|^2_2 \sigma_{\max}^2((\Sigma_b^i )^{-1}) \|X^i_{l_2}\|_2^2  \|\hat v\|_1^2\\
    & \leq \begin{cases}
    c_1 |H_j|^2 \frac{m\log(p)\log^5(n)}{nq^2} \|G_j\|_2&, q>c_0m,\\
    c_1 |H_j|^2 \frac{\log(p)\log^4(n)}{mn} \|G_j\|_2  &, m>c_0q \text{ and } q=p,\\
    c_1 |H_j|^2 \frac{\log(p)\log^5(n)}{n}\|G_j\|_2 &, m>c_0q \text{ and } q<p,
    \end{cases}
\end{align*}
with probability at least $1-c_1\exp\{-cmnq^{-\qm}\}-c_2\exp\{-c\log(n)\}-c_3\exp\{-cn\}-c_4\exp\{-c\log(p)\}-c_5\exp\{-cn(m/q)^{\qm}\} - c_6\exp\{-cmn\}$. 

Therefore, under Assumption \ref{as.B}, we get the stated bounds for $\max_i \| (\Sigma_{\theta^*}^i)^{1/2} (\Sigma_{b}^i)^{-1/2} \hat w_j^i\|_2^2$.
\end{enumerate}
}
\end{proof}

\section{Sandwich Estimator for $V_j$}
\label{S:C}
 
\begin{assumption}
 \label{as.C}
 For the three conditions defined in Assumption~\ref{as.B.4}:
 \begin{enumerate}
     \item Under Condition \ref{cond1}:
     \begin{align*}
         \begin{cases}
         \frac{\|G_j\|_2}{\sigma_{\min}(G_j)} \ll \frac{n}{s\log^4(n)\log(p)} \wedge \frac{n}{s^2\log^2(p)}&, q>c_0m \\
         \frac{\|G_j\|_2}{\sigma_{\min}(G_j)} \ll \frac{n}{s^2\log(p)\log^3(n)}&, m>c_0q,\ p=q\\
         \frac{\|G_j\|_2}{\sigma_{\min}(G_j)} \ll \frac{n}{s m \log(p)\log^3(n)} \wedge \frac{n\log(n)}{s^2m^2\log(p)} &, m>c_0q,\ p>q
         \end{cases}
     \end{align*}
     \item Under Condition \ref{cond2}:
          \begin{align*}
         \begin{cases}
         \frac{\|G_j\|_2}{\sigma^2_{\min}(G_j)} \ll \frac{n}{s\log^5(n)\log(p)} \wedge \frac{n}{s^2\log^2(n)\log^2(p)} &, q>c_0m \\
         \frac{\|G_j\|_2}{\sigma^2_{\min}(G_j)} \ll \frac{mn}{s^2\log(p)\log^3(n)}&, m>c_0q,\ p=q\\
         \frac{\|G_j\|_2}{\sigma^2_{\min}(G_j)} \ll \frac{n}{s \log(p)\log^3(n)} \wedge \frac{n\log(n)}{s^2m\log(p)}&, m>c_0q,\ p>q
         \end{cases}
     \end{align*}
     \item Under Condition \ref{cond3}:
          \begin{align*}
         \begin{cases}
         \frac{\|G_j\|_2}{\sigma_{\min}(G_j)} \ll \frac{n}{sm\log^5(n)\log(p)} \wedge \frac{n}{s^2m\log^3(n)\log^2(p)} &, q>c_0m \\
         \frac{\|G_j\|_2}{\sigma_{\min}(G_j)} \ll \frac{n}{s^2m\log(p)\log^4(n)}&, m>c_0q,\ p=q\\
         \frac{\|G_j\|_2}{\sigma_{\min}(G_j)} \ll \frac{n}{s m^2 \log(p)\log^4(n)} \wedge \frac{n}{s^2m^3\log(p)}&, m>c_0q,\ p>q
         \end{cases}
     \end{align*}
 \end{enumerate}
 \end{assumption}

\begin{theorem}
\label{lemma:Vj}
Under Assumption \ref{as.A}, Assumption \ref{as.B}, Assumption \ref{as.B.4} and Assumption \ref{as.C}, with probability at least $1-c_1\exp\{-cn\} -c_2\exp\{-c\log(n)\} - c_3\exp\{-cmnq^{-\qm}\} -c_4\exp\left\{-cn\left(m/q\right)^{\qm} \right\} -c_5\exp\{-c\log(p)\} - c_6\exp\{-cmn\}$ we have
\begin{align*}
    \frac{\hat V_j}{V_j}  = 1 + o_p(1).
\end{align*}
\end{theorem}

\subsection{Proof of Theorem \ref{lemma:Vj}}
\begin{proof}
According to the definitions of $\hat V_j$ and $V_j$, we can write:
\begin{align}
    \frac{\hat V_j}{V_j} & = \frac{\sum_{i=1}^n\left| (\hat w_j^i)^\top (\Sigma_b^i)^{-1/2} \left(y^i - X^i\hat\beta\right) \right|^2}{\hat w_j^\top \Sigma_b^{-1/2} \Sigma_{\theta^*}\Sigma_b^{-1/2} \hat w_j}  \nonumber \\
    & = \frac{\sum_{i=1}^n\left| (\hat w_j^i)^\top (\Sigma_b^i)^{-1/2} \left(y^i - X^i\beta^*\right) \right|^2}{\hat w_j^\top \Sigma_b^{-1/2} \Sigma_{\theta^*}\Sigma_b^{-1/2} \hat w_j} \label{e.vj.e1}\\
    & \quad + \frac{\sum_{i=1}^n\left| (\hat w_j^i)^\top (\Sigma_b^i)^{-1/2} X^i \left(\hat \beta - \beta^*\right) \right|^2}{\hat w_j^\top \Sigma_b^{-1/2} \Sigma_{\theta^*}\Sigma_b^{-1/2} \hat w_j} \label{e.vj.e2}\\
    & \quad + 2\frac{\sum_{i=1}^n (\hat w_j^i)^\top (\Sigma_b^i)^{-1/2} \left(y^i - X^i\beta^*\right) \times (\hat w_j^i)^\top (\Sigma_b^i)^{-1/2} X^i \left(\beta^* - \hat\beta\right)}{\hat w_j^\top \Sigma_b^{-1/2} \Sigma_{\theta^*}\Sigma_b^{-1/2} \hat w_j} \label{e.vj.e3}.
\end{align}

Denote $\xi_i = (\Sigma_{\theta^*}^i)^{1/2}(\Sigma_{b}^i)^{-1/2} \hat w_j^i$, $\delta_i = (\Sigma_{a}^i)^{1/2}(\Sigma_{b}^i)^{-1/2} \hat w_j^i$, $\hat u = \hat \beta - \beta^*$, and  $\tilde \epsilon_i = (\Sigma_{\theta^*}^i)^{-1/2} (y^i - X^i\beta^*)$. 

\begin{enumerate}
    \item For term \eqref{e.vj.e1}: 
    \begin{align*}
        \frac{\sum_{i=1}^n\left| (\hat w_j^i)^\top (\Sigma_b^i)^{-1/2} (y^i - X^i\beta^*) \right|^2}{\hat w_j^\top \Sigma_b^{-1/2} \Sigma_{\theta^*}\Sigma_b^{-1/2} \hat w_j} = \frac{\sum_{i=1}^n (\xi_i^\top \tilde\epsilon_i )^2}{\sum_{i=1}^n \|\xi_i \|_2^2}.
    \end{align*}
    Denote $E_1 := \frac{\sum_{i=1}^n (\xi_i^\top \tilde\epsilon_i )^2}{\sum_{i=1}^n \|\xi_i \|_2^2}$. Then conditioning on $X^i$'s, we have 
    \[
    \sum_{i=1}^n (\xi_i^\top \tilde\epsilon_i )^2 - \sum_{i=1}^n \|\xi_i \|_2^2 \in \SE\left(c_1\sum_{i=1}^n \|\xi_i \|_2^4, c_2\max_i \|\xi_i \|_2^2\right).
    \]
    By the tail bound of sub-exponential random variables, we have
    \begin{align*}
        \P(| E_1 - 1| >t \mid X) \leq 2\exp\left\{ -c_1\min \left(\frac{t^2 \left(\sum_{i=1}^n \|\xi_i \|_2^2\right)^2}{\sum_{i=1}^n \|\xi_i \|_2^4}, \frac{t \sum_{i=1}^n \|\xi_i \|_2^2}{\max_i \|\xi_i \|_2^2} \right)\right\},
    \end{align*}
    where by Lemma \ref{lemma:b.3}.\ref{lemma:b.3.6} and under the conditions of Theorem \ref{thm:S2},
    \begin{align*}
        \frac{\sum_{i=1}^n \|\xi_i \|_2^4}{\left(\sum_{i=1}^n \|\xi_i \|_2^2\right)^2} & \leq \frac{\max_i \|\xi_i \|_2^2}{\sum_{i=1}^n \|\xi_i \|_2^2} = o_p\left(\log^{-2}(n)\right).
    \end{align*}
    Thus, $|E_1-1| < \log^{-1/2}(n)$ with probability at least $1-c_1\exp\{-cmnq^{-\qm}\}-c_2\exp\{-c\log(n)\}-c_3\exp\{-cn\}-c_4\exp\{-c\log(p)\}-c_5\exp\{-cn(m/q)^{\qm}\} - c_6\exp\{-cmn\}$.
    
    \item For term \eqref{e.vj.e2}: Recall that $\Sigma_a = \diag\left(\{\Sigma_a^i\}_{i=1}^n \right)$ and $X$ is obtained by vertically stacking the $X^i$'s. We can write
    \begin{align*}
        & \frac{\sum_{i=1}^n\left| (\hat w_j^i)^\top (\Sigma_b^i)^{-1/2} X^i (\hat \beta - \beta^*) \right|^2}{\hat w_j^\top \Sigma_b^{-1/2} \Sigma_{\theta^*}\Sigma_b^{-1/2} \hat w_j} \\
        & = \frac{\sum_{i=1}^n\left| (\hat w_j^i)^\top (\Sigma_b^i)^{-1/2} (\Sigma_a^i)^{1/2}(\Sigma_a^i)^{-1/2} X^i (\hat \beta - \beta^*) \right|^2}{\hat w_j^\top \Sigma_b^{-1/2} \Sigma_{\theta^*}\Sigma_b^{-1/2} \hat w_j} \\
        & \leq \frac{\max_i \left| (\hat w_j^i)^\top (\Sigma_b^i)^{-1/2} (\Sigma_a^i)^{1/2}(\Sigma_b^i)^{-1/2} \hat w_j^i \right|  \times \left\|\Sigma_a^{-1/2} X (\hat \beta - \beta^*) \right\|_2^2}{\hat w_j^\top \Sigma_b^{-1/2} \Sigma_{\theta^*}\Sigma_b^{-1/2} \hat w_j} \\
        & \leq \frac{\max_i \left\| \hat w_j^i \right\|_2^2  \sigma_{\max}\left( (\Sigma_b^i)^{-1} \Sigma_a^i  \right)  \left\|\Sigma_a^{-1/2} X (\hat \beta - \beta^*) \right\|_2^2}{\hat w_j^\top \Sigma_b^{-1/2} \Sigma_{\theta^*}\Sigma_b^{-1/2} \hat w_j}.
    \end{align*}
    Using \eqref{eq.sum.x.square} and Lemma \ref{lemma:A.1}.\ref{lemma:A.1(6.3)}, we can bound $\sigma_{\max}\left( (\Sigma_b^i)^{-1} \Sigma_a^i \right)$ by 
    \begin{align*}
        \sigma_{\max}\left( (\Sigma_b^i)^{-1} \Sigma_a^i  \right) & = \begin{cases}
        \sigma_{\max}\left( (\Sigma_a^i)^{-1} \Sigma_a^i  \right)  &, \text{ if } j >  q,\\
        \sigma_{\max}\left(I + a Z^i_j(Z^i_j)^\top (\Sigma_b^i)^{-1}\right) &, \text{ if } j \leq q
        \end{cases}\\
        & \leq \begin{cases}
        1 &, \text{ if } j >  q,\\
        1 +  (Z^i_j)^\top (\Sigma_b^i)^{-1}Z^i_j \leq 1 + c_1 m\log(n) \left(1\wedge \frac{\log(n)}{m\vee q}\right) &, \text{ if } j \leq q
        \end{cases}\\
        & \leq c_1\log^2(n).
    \end{align*}
    Then using Lemma \ref{lemma:b.3}.\ref{lemma:b.3.7} to bound $\max_i\|\hat w_j^i\|_2^2$, Lemma \ref{lemma:b.3}.\ref{lemma:b.3.6} to bound $\hat w_j^\top \Sigma_b^{-1/2} \Sigma_{\theta^*}\Sigma_b^{-1/2} \hat w_j$ and Theorem \ref{thm:S1} to bound $\|\Sigma_a^{-1/2} X (\hat \beta - \beta^*)\|_2^2$, under Assumption \ref{as.C}, we obtain
    \begin{align*}
        \frac{\sum_{i=1}^n\left| (\hat w_j^i)^\top (\Sigma_b^i)^{-1/2} X^i (\hat \beta - \beta^*) \right|^2}{\hat w_j^\top \Sigma_b^{-1/2} \Sigma_{\theta^*}\Sigma_b^{-1/2} \hat w_j} = o_p(1).
    \end{align*}

    \item For term \eqref{e.vj.e3}:
    \begin{align}
        &\frac{\sum_{i=1}^n (\hat w_j^i)^\top (\Sigma_b^i)^{-1/2} (y^i - X^i\beta^*) \times (\hat w_j^i)^\top (\Sigma_b^i)^{-1/2} X^i(\beta^* - \hat\beta)}{\hat w_j^\top \Sigma_b^{-1/2} \Sigma_{\theta^*}\Sigma_b^{-1/2} \hat w_j} \nonumber \\ 
        & \leq  \frac{\|\hat u \|_2^2}{\sum_{i=1}^n \|\xi_i\|_2^2} \left\| \sum_{i=1}^n \xi_i^\top \tilde \epsilon_i (X^i)^\top (\Sigma_b^i)^{-1/2} \hat w_j^i \right \|_\infty \nonumber \\
        & \leq  \frac{\|\hat u \|_2^2}{\sum_{i=1}^n \|\xi_i\|_2^2} \max_{1\leq l \leq p} \left |\sum_{i=1}^n (X^i_l)^\top (\Sigma_b^i)^{-1/2} \hat w_j^i \xi_i^\top \tilde \epsilon_i  \right |. \label{vj.e3.1}
    \end{align}
Conditioning on $X^i$'s, $\tilde \epsilon_i \in \SGV(c_1)$, and we use the tail bound of sub-Gaussian random variables to get
\begin{align*}
    \P\left( \max_{1\leq l \leq p} \left| \sum_{i=1}^n (X_l^i)^\top (\Sigma_b^i)^{-1/2} \hat w_j^i \xi_i^\top \tilde \epsilon_i  \right| > t \mid X \right) \leq 2\exp\left\{ \log(p) - c_1 \frac{t^2}{\max_l \sum_{i=1}^n \| (X_l^i)^\top (\Sigma_b^i)^{-1/2} \hat w_j^i  \xi_i \|_2^2} \right\}.
\end{align*}
Then, taking $t = c_2\sqrt{\log(p)} \sqrt{\max_l \sum_{i=1}^n \| (X_l^i)^\top (\Sigma_b^i)^{-1/2} \hat w_j^i  \xi_i \|_2^2}$ and plugging the bound into \eqref{vj.e3.1}, with probability at least $1-2\exp\{-c\log(p)\}$, we have 
\begin{align*}
    &\frac{\sum_{i=1}^n (\hat w_j^i)^\top (\Sigma_b^i)^{-1/2} (y^i - X^i\beta^*) \times (\hat w_j^i)^\top (\Sigma_b^i)^{-1/2} X^i(\beta^* - \hat\beta)}{\hat w_j^\top \Sigma_b^{-1/2} \Sigma_{\theta^*}\Sigma_b^{-1/2} \hat w_j} \\ 
    & \leq c_3 \frac{\|\hat u \|_2^2}{\sum_{i=1}^n \|\xi_i\|_2^2} \sqrt{\log(p)} \sqrt{\max_l \sum_{i=1}^n \| (X_l^i)^\top (\Sigma_b^i)^{-1/2} \hat w_j^i  \xi_i \|_2^2}\\
     & \leq c_3 \frac{\|\hat u \|_2^2}{\sum_{i=1}^n \|\xi_i\|_2^2} \sqrt{\log(p)} \sqrt{\max_l \sum_{i=1}^n \|\hat w_j^i\|_2^2 \|\xi_i\|_2^2 \|  (\Sigma_b^i)^{-1/2}X_l^i \|_2^2}\\
     & \leq c_3 \frac{\|\hat u \|_2^2}{\sum_{i=1}^n \|\xi_i\|_2^2} \sqrt{\log(p)} \max_i  \|\hat w_j^i\|_2 \max_l  \|\xi_i\|_2 \sqrt{\sigma_{\max}(X^\top \Sigma_b^{-1} X)}.
\end{align*}
Then, under the conditions of Theorem \ref{thm:S2} and Assumption \ref{as.C}, we use Theorem \ref{thm:S1} to bound $\|\hat u\|_2^2$, use Lemma \ref{lemma:A.3}.\ref{lemma:A.3.1} to bound $\sigma_{\max}(X^\top \Sigma_b^{-1} X)$, use Lemma \ref{lemma:b.3}.\ref{lemma:b.3.6} to bound $\sum_{i=1}^n \|\xi_i\|_2^2$, $\max_l  \|\xi_i\|_2$ and Lemma \ref{lemma:b.3}.\ref{lemma:b.3.7} to bound $\max_i  \|\hat w_j^i\|_2$. Then it follows that \eqref{e.vj.e3} is $o_p(1)$ with probability at least $1-c_1\exp\{-cmnq^{-\qm}\}-c_2\exp\{-c\log(n)\}-c_3\exp\{-cn\}-c_4\exp\{-c\log(p)\}-c_5\exp\{-cn(m/q)^{\qm}\} - c_6\exp\{-cmn\}$.
\end{enumerate}

\end{proof}

\section{Variance Component Estimator $\hat\theta$}
\label{Ssec:VC}

\begin{assumption}
 \label{as.D}
 \begin{enumerate}
     \item \label{as.D.1} The vectors $\gamma_i$ and $\epsilon_i$ are normally distributed with mean zero and variance matrices $\Psi$, $\sigma_e^2 I_m$, respectively. The covariance matrix $\Psi$ satisfies Assumption~\ref{as.A.add}.\ref{as.A.3}. 
     \item \label{as.D.2}\label{as.D.3} The following conditions hold: 
     \begin{align*}
     & \sqrt{m} \gg \log(nq) \\
     & nm \gg \max \left\{ q^{3/2}\log(q) \log^2(n), \log(q) \log(n) \left(s_Z\sqrt{m}\log(nq^2) + q\log^2(nq^2)\right) \right\} \\
     & nm^3 \gg q^2\log(q)\log^2(n)
     \end{align*}
     \item \label{as.D.4} $\sqrt{n}m \gg s s_\psi (q/m)^{\qm} m^{\bm{1}\{p>q, m>c_0q\}}\log(q)\log(p)\log(n)\log(nmq)$.
 \end{enumerate}
 
\end{assumption}

\begin{theorem}
\label{thm:Svc}
Under Assumption~\ref{as.A} and Assumption~\ref{as.D}.\ref{as.D.1}--\ref{as.D}.\ref{as.D.3}, with probability at least $1 - c_1\exp\{-c\log(nq)\} -c_2\exp\{-cn\} -c_3\exp\{-c\log(n)\} - c_4\exp\{-cmnq^{-\qm}\} - c_5\exp\{-cn(m/q)^{\qm}\}  - c_6\exp\{-c\log(q)\}$, we have 
\begin{align*}
    \|\hat\psi- \psi^*\|_\delta & \leq s_{\psi}^{1/\delta}  \frac{\log(n)\log(p)\log(nmq)}{\sqrt{n}} m^{\bm{1}\{m>c_0q, p>q\}} (q/m)^{\qm}, \quad \delta=1, 2.
\end{align*}
\end{theorem}

\begin{theorem}
\label{thm:Svc.e}
Under Assumption~\ref{as.A} and Assumption~\ref{as.D}, we have $|\hat\sigma_e^2 - \sigma_e^{2, *}| = o_p(1)$ with probability at least
\begin{align*}
1- & c_1\frac{s_\psi (m\vee q)\log^3(n)}{nm}  - c_2\exp\{-cnm\} - c_3\exp\{-cn\} -c_4\exp\{-c\log(n)\} - c_5\exp\{-cmnq^{-\qm}\}  \\
& - c_6 \exp\{-cn(m/q)^{\qm}\}
 - c_7\exp\left\{- c \frac{n^2}{s\log^4(n)\log(p)} \left(\frac{m^2}{q^2}\right)^{\qm} m^{-\bm{1}\{ m>c_0q, p>q\}} \right\}
 \end{align*}
\end{theorem}

\subsection{Related lemmas for Theorem~\ref{thm:Svc} and Theorem~\ref{thm:Svc.e}}
\begin{lemma}
\label{lemma.D.1}
\begin{enumerate}
    \item \label{lemma.D.1.E1} For $1 \leq j \leq q$, define 
    \begin{align*}
        E_{1, j} & =\sum_{i\in S_2} \Tr\left( A_j^i  \left(r_i r_i^\top -  \sum_{k=1}^{q} A_k^i  \psi_k^* \right) \right) . 
    \end{align*}
    Under Assumption~\ref{as.A} and Assumption~\ref{as.D}.\ref{as.D.1}, with probability at least $1-2\exp\{-c(m\vee q)\log(n)\} - 2\exp\{-cm\log(nq)\} - 2\exp\{-c\log(nmq)\} -2\exp\{-c\log(q)\}$, we have 
    \begin{align*}
    \max_j|E_{1, j}| \leq c_1(m \vee q) \log(n)\log(nmq)\log(q) m\sqrt{n}.
\end{align*}

    \item \label{lemma.D.1.E2} Define 
    \begin{align*}
        E_{2, j} & =\sum_{i \in S_2} \Tr\left(A_j^i X^i (\beta^*-\hat\beta) (\beta^*-\hat\beta)^\top (X^i)^\top \right). 
    \end{align*}
    Under Assumption~\ref{as.A} and Assumption~\ref{as.D}.\ref{as.D.1}, with probability at least  $1-4\exp\{-cn\} -12\exp\{-c\log(n)\} - 2\exp\{-cmnq^{-\qm}\} - \exp\{-cn(m/q)^{\qm}\} - 2\exp\{-cm\log(nq)\} -2\exp\{-c\log(nmq)\} -2\exp\{-c(m\vee q)\log(n)\}$, we have
    \begin{align*}
   \max_j|E_{2, j}| \leq \begin{cases}
   c_2s\log(p)\log^3(n)\log(nq)m^2 &, q>c_0m \\
   c_2s\log(p)\log(n)\log(nq)m^2 &, m>c_0q,\ p=q \\
   c_2s\log(p)\log(n)\log(nq)m^3 &, m>c_0q,\ p>q,
   \end{cases}
\end{align*}

    \item \label{lemma.D.1.E3} Define 
    \begin{align*}
        E_{3, j} & = \sum_{i\in S_2} \Tr\left( A_j^i  r_i (\beta^*-\hat\beta)^\top (X^i)^\top \right).
    \end{align*}
    Under Assumption~\ref{as.A} and Assumption~\ref{as.D}.\ref{as.D.1}, with probability at least $1-4\exp\{-cn\} -12\exp\{-c\log(n)\} - 2\exp\{-cmnq^{-\qm}\} - \exp\{-cn(m/q)^{\qm}\} - 2\exp\{-cm\log(nq)\} -2\exp\{-c\log(nmq)\} -2\exp\{-c\log(q)\}- 2\exp\{-c(m\vee q)\log(n)\}$, we have \begin{align*}
    \max_{j}|E_{3,j}| \leq 
    \begin{cases}
    c_3\sqrt{s\log(p)\log(q)\log^4(n)\log^2(nq)m^3{q}} &, q>c_0m \\
    c_3\sqrt{s\log(p)\log(q)\log^2(n)\log^2(nq)m^4} &, m>c_0q,\ p=q \\
    c_3\sqrt{s\log(p)\log(q)\log^2(n)\log^2(nq)m^5} &, m>c_0q,\ p>q.
   \end{cases}
\end{align*}
    
\end{enumerate}
\end{lemma}

\begin{lemma}
\label{lemma.D.2}
Define $G_1^i =\left( (Z^{i})^\top Z^i\right) \circ \left( (Z^{i})^\top Z^i\right)$ and $G_2^i = \left(Z^{i} \circ Z^i \right)^\top \left(Z^{i} \circ Z^i \right)$. 
\begin{enumerate}
    \item \label{lemma.D.2.G1} Under Assumption~\ref{as.A}, Assumption~\ref{as.D}.\ref{as.D.1} and Assumption~\ref{as.D}.\ref{as.D.2}, with probability at least $1- 2\exp\{-c\log(nq)\} - 2\exp\{-c\log(nq^2)\}$, we have $\max_i\left\|G^i_1 - \E\left(G^i_1\right)\right\|_2 \leq c_1m^{3/2} \log(nq^2) + c_1s_Z m^{3/2} \log(nq^2)  + c_1 m q\log^2(nq^2)$.
    
    \item \label{lemma.D.2.G2} Under Assumption~\ref{as.A} and Assumption~\ref{as.D}.\ref{as.D.1}, we have $ \max_i \|G_2^i - \mathbb{E}(G_2^i) \|_2^2 \leq c_2 mq\log(n)$ with probability at least $1-\exp\{- c q\log(n)\}$. 

\end{enumerate}
\end{lemma}

\begin{lemma}
\label{lemma:RE_for_B}
Under Assumption~\ref{as.A} and Assumption~\ref{as.D}, with probability at least $1-\exp\{-c\log(q)\} -2\exp\{-c\log(nq)\} - \exp\{-cq\log(n)\}$, for any $v\in\R^{q}$ we have $v^\top B v \geq c_1nm^2\|v\|_2^2$, where $B$ is defined in Appendix equation (19). %\eqref{def.B}.
\end{lemma}

\subsection{Proof of Theorem~\ref{thm:Svc}}

\begin{proof}[Proof of Theorem~\ref{thm:Svc}]
$\left.\right.$

We first show the consistency of $\hat\psi$.

Based on the definition of $\hat\psi$ in equation (7) %\eqref{main.hat.psi.def} 
in the main paper and the definition of $A_l^i$ in Appendix equation (18) %\eqref{def.A.G}
, we can write
\begin{align*}
 \hat\psi & = \arg\min_{\psi}\sum_{i \in S_2} \left\| \hat r_i \hat r_i^\top - \left(\diag(\hat r_i)\right)^2 - \sum_{l=1}^q \psi_l A_l^i \right\|_F^2 +\lambda_\theta\|\psi\|_1 \\
& = \arg\min_{\psi} \sum_{i \in S_2} \Tr \left( \left( \hat r_i \hat r_i^\top - \left(\diag(\hat r_i)\right)^2 - \sum_{l=1}^q \psi_l A_l^i \right)^2 \right) +\lambda_\theta\|\psi\|_1 . 
\end{align*}

Rearranging the terms, we can write
\begin{align}
    & \sum_{i \in S_2} \Tr \left( \left( \hat r_i \hat r_i^\top - \left(\diag(\hat r_i)\right)^2 - \sum_{l=1}^q \hat\psi_l A_l^i \right)^2 \right) +\lambda_\theta\|\hat\psi\|_1   \leq \sum_{i \in S_2} \Tr \left( \left( \hat r_i \hat r_i^\top - \left(\diag(\hat r_i)\right)^2 - \sum_{l=1}^q \psi_l^* A_l^i \right)^2 \right) +\lambda_\theta\|\psi^*\|_1 \nonumber \\
    % \Rightarrow &  \sum_{i\in S_2} \Tr\left(\left(\sum_{l=1}^{q}\hat\sigma_l^2 A_l^i\right)\left(\sum_{l=1}^{q}\hat\sigma_l^2 A_l^i\right)  - 2 \left(\sum_{l=1}^{q}\hat\sigma_l^2 A_l^i\right)\hat R^i \right)  + \lambda_\sigma\|\hat{\bm{\sigma}}^2\|_1 \\
    % & \quad \quad \leq \sum_{i=1}^{n_2} \Tr\left( \left(\sum_{l=1}^{q} \sigma^{2,*}_l A_l^i\right) \left(\sum_{l=1}^{q} \sigma^{2,*}_l A_l^i\right)  - 2 \left(\sum_{l=1}^{q} \sigma^{2,*}_l A_l^i\right) \hat R^i \right)  + \lambda_\sigma\| \bm{\sigma}^{2,*}\|_1 \\
    \Rightarrow & \sum_{i\in S_2} \Tr\left(\sum_{l_1=1}^{q}\sum_{l_2=1}^{q}\hat\psi_{l_1}\hat\psi_{l_2}  A_{l_1}^i A_{l_2}^i - 2\sum_{l=1}^{q} \hat\psi_l  A_{l}^i  \left(\hat r_i\hat r_i^\top - \left(\diag(\hat r_i)\right)^2 \right) \right) + \lambda_\theta\|\hat\psi\|_1 \nonumber \\
    &\quad \quad \leq \sum_{i\in S_2} \Tr\left(\sum_{l_1=1}^{q}\sum_{l_2=1}^{q}\psi^*_{l_1}\psi^*_{l_2}  A_{l_1}^i A_{l_2}^i - 2\sum_{l=1}^{q} \psi^*_l  A_{l}^i  \left(\hat r_i\hat r_i^\top - \left(\diag(\hat r_i)\right)^2 \right) \right) + \lambda_\theta\|\psi^*\|_1. \label{eq.vc.1}
\end{align}

Recall the definition of $B$ in Appendix equation (19). %\eqref{def.B}. 
Define the length $q$ vector $\delta$ with $\delta_k = \sum_{i\in S_2} \Tr\left(A_{k}^i \left(\hat r_i\hat r_i^\top - \left(\diag(\hat r_i)\right)^2 \right) \right)$ for $k=1, \dots, q$. Then the above inequality \eqref{eq.vc.1} implies:
\begin{align*}
 (\hat\psi - \psi^*)^\top B (\hat\psi - \psi^*) &\leq 2 (\hat\psi - \psi^*) (\delta - B\psi^*)+\lambda_\theta\|\psi^*\|_1 - \lambda_\theta \|\hat\psi\|_1 \\
    & \leq 2 \|\hat\psi - \psi^*\|_1 \|\delta - B\psi^*\|_\infty +\lambda_\theta\|\psi^*\|_1 - \lambda_\theta \|\hat\psi\|_1.
\end{align*}

We next show that $\|\delta - B\psi^*\|_\infty$ is upper bounded by $(\hat\psi - \psi^*)^\top B (\hat\psi - \psi^*)$, such that we can follow similar arguments as those in the proof of Theorem~\ref{thm:S1} to show the consistency of $\hat\psi$. 

For the term $\|\delta - B\psi^*\|_\infty$, we can write
\begin{align}
    |\left(\delta - B\psi^* \right)_j| 
    & = \left|\sum_{i\in S_2} \Tr\left( A_j^i \left( \hat r_i \hat r_i^\top - \left(\diag(\hat r_i)\right)^2 - \sum_{l=1}^q A_l^i \psi_l^* \right) \right) \right| \nonumber \\
    & = \left|\sum_{i\in S_2} \Tr\left( A_j^i  \left(r_i r_i^\top- \left(\diag(r_i)\right)^2 -  \sum_{l=1}^{q} A_l^i  \psi_l^*\right) \right) \right. \nonumber \\
    & \quad \quad + \sum_{i\in S_2} \Tr\left(A_j^i \left [X^i (\beta^*-\hat\beta) (\beta^*-\hat\beta)^\top (X^{i})^\top- \left(\diag\left(X^i (\beta^*-\hat\beta)\right)\right)^2\right ]\right) \nonumber \\
    & \left.\quad \quad + \ 2 \sum_{i\in S_2} \Tr\left( A_j^i \left[ r_i (\beta^*-\hat\beta)^\top (X^i)^\top - \diag\left(r_i (\beta^*-\hat\beta)^\top (X^i)^\top \right) \right] \right) \right| \nonumber \\
    & = \left|\sum_{i \in S_2} \Tr\left( A_j^i  \left(r_i r_i^\top -  \sum_{l=1}^{q} A_l^i  \psi_l^* \right) \right) \right. \label{vc.E1}\\
    & \quad \quad + \sum_{i \in S_2} \Tr\left(A_j^i X^i (\beta^*-\hat\beta) (\beta^*-\hat\beta)^\top (X^i)^\top\right)  \label{vc.E2} \\
    & \left.\quad \quad + \ 2 \sum_{i\in S_2} \Tr\left( A_j^i  r_i (\beta^*-\hat\beta)^\top (X^i)^\top \right) \right|, \label{vc.E3} 
\end{align}
where the last equality holds because $\tr\left(A_j^i \diag(u)\right) = 0$ for any vector $u\in \R^m$. Then using Lemma~\ref{lemma.D.1}, we can bound the terms \eqref{vc.E1}, \eqref{vc.E2} and \eqref{vc.E3} to get
\begin{align*}
    |\left(\delta - B\psi^*\right)_j| \leq  c_1\log(n)\log(p)\log(nmq)   m^{1+\bm{1}\{m>c_0q, p>q\}}(m\vee q)\sqrt{n} \leq \lambda_\theta/4
\end{align*}
with probability at least $1-4\exp\{-cn\} -12\exp\{-c\log(n)\} - 2\exp\{-cmnq^{-\qm}\} - \exp\{-cn(m/q)^{\qm}\} - 2\exp\{-cm\log(nq)\} -2\exp\{-c\log(nmq)\} - 2\exp\{-c\log(q)\} -2\exp\{-c(m\vee q)\log(n)\}$.

On the other hand, using Lemma \ref{lemma:RE_for_B} we can show that with probability at least $1-\exp\{-c\log(q)\} - 2\exp\{-c\log(nq)\} -\exp\{-cq\log(n)\}$, we have
\begin{align*}
    (\hat\psi - \psi^*)^\top B (\hat\psi - \psi^*) \geq c_2 n m^2 \|\hat\psi-\psi^*\|_2^2.
\end{align*}

Next, letting $v = \hat{\psi} - \psi^*$, we follow the similar arguments as those in the proof of Theorem~\ref{thm:S1} to show that
\begin{align*}
    c_2nm^2 \|v\|_2^2 \leq \frac{3}{2} \lambda_\theta \|v_{S_\psi}\|_1 \leq \frac{3}{2}\lambda_\theta \sqrt{s_\psi} \|v\|_2.
\end{align*}
Thus, with probability at least $1 - c_3\exp\{-c\log(nq)\} -c_4\exp\{-cn\} -c_5\exp\{-c\log(n)\} - c_6\exp\{-cmnq^{-\qm}\} - c_7\exp\{-cn(m/q)^{\qm}\}  - c_8\exp\{-c\log(q)\}$ we have 
\begin{align*}
    \|\hat\psi- \psi^*\|_1 & \leq s_{\psi}  \frac{\log(n)\log(p)\log(nmq)}{\sqrt{n}} m^{\bm{1}\{m>c_0q, p>q\}} (q/m)^{\qm}\\
    \|\hat\psi- \psi^*\|_2 & \leq \sqrt{s_{\psi}}  \frac{\log(n)\log(p)\log(nmq)}{\sqrt{n}} m^{\bm{1}\{m>c_0q, p>q\}} (q/m)^{\qm}.
\end{align*}
\end{proof}

\begin{proof}[Proof of Theorem~\ref{thm:Svc.e}]
$\left.\right.$
We can write the proposed estimator $\hat\sigma_e^2$ as:
\begin{align*}
    \hat\sigma_e^2 & =  \sigma_e^{2,*} + \frac{1}{n_3m} \sum_{i \in S_3}\left(\Tr(\hat r_i \hat r_i^\top  - \Sigma^i_{\theta^*}) - \Tr(Z^i \diag(\hat\psi) (Z^i)^\top - Z^i \diag(\psi) (Z^i)^\top )\right). 
\end{align*}
We can then show that
\begin{align}
    n_3m \left|\hat\sigma_e^2 - \sigma_e^{2,  *}\right| & = \sum_{i \in S_3}\|r_i\|_2^2 + \|X^i (\beta^*-\hat\beta)\|_2^2 + 2 (\beta^*-\hat\beta)^\top (X^i)^\top r_i - \Tr(\Sigma^i_{\theta^*}) - \Tr\left(Z^i \diag(\hat\psi - \psi^*) (Z^i)^\top\right) \nonumber \\
    & \leq \sum_{i \in S_3} \|r_i\|_2^2 - \Tr(\Sigma^i_{\theta^*})  \label{vc.e.1}\\
    & \quad + \|X (\beta^*-\hat\beta)\|_2^2 \label{vc.e.2} \\
    & \quad + 2 \sum_{i \in S_3} (\beta^*-\hat\beta)^\top (X^{i})^\top r_i \label{vc.e.3} \\
    & \quad + \sum_{i \in S_3} \Tr\left(Z^i \diag(\hat\psi - \psi^*) (Z^i)^\top\right) \label{vc.e.4}.
\end{align}

     For the term \eqref{vc.e.1}: 
    {
    Conditioning on the design matrices $Z^i$, we have $r_i \mid Z^i \sim N(0, \Sigma_\theta^i)$ independently for $i=1, \ldots, n$, and $\E\left(\|r_i\|_2 \mid Z^i\right) = \tr(\Sigma_{\theta^*}^i)$. Denote the $(j,k)$ entry of $\Sigma_{\theta^*}^i$ by $w_{i,j,k}$. By Markov's inequality we can show that
    \begin{align}
        & \mathbb{P}\left( \left|\sum_{i \in _3} \|r_i\|_2^2 - \Tr(\Sigma^i_{\theta^*})  \right|  \geq t \mid Z^i \right) 
        \leq \frac{\sum_{i \in S_3}\mathrm{Var}\left(\|r_i\|_2^2\right)}{t^2} \nonumber \\
        &  = \frac{ \sum_{i \in S_3} \left( \sum_{j=1}^{m} 3w_{i, j, j}^2 + \sum_{k=1}^m \sum_{j=1, j\neq k}^{m} (w_{i, j, j}w_{i, k, k} + 2 w^2_{i, j, k})  - (\sum_{j=1}^{m}w_{i, j, j})^2   \right)}{t^2} \nonumber \\
        & = \frac{\sum_{i \in S_3}\sum_{k=1}^m \sum_{j=1}^{m}2 w^2_{i, j, k}}{t^2} = \frac{\sum_{i \in S_3} \|\Sigma_{\theta^*}^i \|_F^2}{t^2}.\label{vc.e.1.p1}
    \end{align}
    
    Note that we have $\Psi = \diag(\psi)$ with $\|\psi\|_0 = s_\psi < c_1 m\wedge n$ (Assumption \ref{as.A.add}.\ref{as.A.3}), and we can thus show that
    \begin{align}
        \sum_{i\in S_3}\|\Sigma_{\theta^*}^i\|_F^2 & \leq \sum_{i\in S_3} \Tr\left(Z^i \diag(\psi) (Z^i)^\top + \sigma_e^{2}I_m\right) \sigma_{\max}\left(\Sigma_{\theta^*}^i\right) \nonumber \\
        & \leq c_1 \sum_{i\in S_3} \left(\sum_{l \in S_\psi} \psi_l \|Z^i_l\|_2^2 + m\sigma_e^2 \right) \left(\sigma^2_{\max}\left(Z^i\right) + 1\right) \nonumber \\
        & \leq c_2 \left(nm + s_{\psi} \max_{l\in S_\psi}\sum_{i\in S_3} \|Z^i_l\|_2^2 \right) \sigma^2_{\max}(Z^i). \label{vc.e.sigma.F}
    \end{align}
    Using Lemma~\ref{lemma:A.1}.\ref{lemma:A.1(4)}, we have $\sigma^2_{\max}(Z^i) \leq c_3(m \vee q)\log(n)$ with probability at least $1-2\exp\{-c\log(n)\}$. We can also use $Z^i_l \mid \Sigma_Z^i \sim N\left(0, \left(\Sigma_Z^i\right)_{l,l} I_m \right)$ to show that 
    \begin{align}
        & \P\left( \max_{l \in S_\psi} \left|\sum_{i\in S_3} \|Z^i_l\|_2^2 - m\left(\Sigma_Z^i\right)_{l,l} \right| \geq t \mid \Sigma_Z^i \right) \leq 2\exp\left\{\log(s_\psi) - c_4 \min\left\{ \frac{t^2}{4nm}, \frac{t}{4} \right\}\right\} \nonumber \\
        & \Rightarrow \P\left( \max_{l \in S_\psi} \sum_{i\in S_3} \|Z^i_l\|_2^2 \leq c_5nm  \right) \geq 1-2\exp\left\{-cnm\right\}. \label{vc.e.z2}
    \end{align}
    Plugging in the bounds into \eqref{vc.e.sigma.F}, we obtain $ \sum_{i\in S_3}\|\Sigma_{\theta^*}^i\|_F^2 \leq c_6 s_\psi nm (m \vee q)\log(n)$. Then plugging into \eqref{vc.e.1.p1} and taking $t = c_7 nm/\log(n)$, we obtain $\eqref{vc.e.1} \leq nm /\log(n)$ with probability at least $1- c\frac{s_\psi (m\vee q)\log^3(n)}{nm} - 2\exp\{-c\log(n)\} - 2\exp\{-cnm\}$.
 }
    
     For the term \eqref{vc.e.2}: 
    {
    Using Theorem \ref{thm:S1} and Lemma \ref{lemma:A.1}.\ref{lemma:A.1(4)}, we have with probability at least $1- c_1\exp\{-cn\} -c_2\exp\{-c\log(n)\} - c_3\exp\{-cmnq^{-\qm}\} - c_4 \exp\{-cn(m/q)^{\qm}\}$ that 
    \begin{align*}
        \|X (\beta^*-\hat\beta)\|_2^2 & \leq \|\Sigma_a^{-1/2} X (\beta^*-\hat\beta)\|_2^2 \sigma_{\max}(\Sigma_a) \\
        & \leq c_5 \begin{cases}
           sq\log(p)\log(n) &, q>c_0m\\
           sm\log^3(n)\log(p) &, q>c_0m \text{ and assuming Assumption \ref{as.A.add}.\ref{as.A.3}} \\
           sm\log(p)\log(n) &, m>c_0q, \ p=q \\
           sm^2\log(p)\log(n) &, m>c_0q, \ p>q.
        \end{cases}
    \end{align*}
    }
    
    For the term \eqref{vc.e.3}:
    {
    Conditioning on $\hat\beta$ and $X$ and using the tail bound of normally distributed random variables, we can write
    \begin{align}
        \mathbb{P}\left( \left| \sum_{i \in S_3} (\beta^*-\hat\beta)^\top (X^{i})^\top r_i \right| \geq t | X, \hat\beta \right) & \leq 2\exp\left\{ - \frac{t^2}{8\sum_{i \in S_3} (\beta^*-\hat\beta)^\top (X^{i})^\top \Sigma_{\theta^*}^i X^i (\beta^*-\hat\beta) } \right\} \nonumber \\
        & \leq 2\exp\left\{ - \frac{t^2}{8 \max_i\sigma_{\max}(\Sigma_{\theta^*}^i)\sigma_{\max}(\Sigma_a^i) \| \Sigma_a^{-1/2} X (\beta^*-\hat\beta) \|_2^2 }\right\}. \label{vc.e.3.p1}
    \end{align}
    Using Theorem~\ref{thm:S1} to bound $\| \Sigma_a^{-1/2} X (\beta^*-\hat\beta) \|_2^2$ and Lemma~\ref{lemma:A.1}.\ref{lemma:A.1(4)} to bound $\sigma_{\max}(\Sigma_{\theta^*}^i)\sigma_{\max}(\Sigma_a^i)$, we have with probability at least $1- c_1\exp\{-cn\} -c_2\exp\{-c\log(n)\} - c_3\exp\{-cmnq^{-\qm}\} - c_4 \exp\{-cn(m/q)^{\qm}\}$,
    \begin{align*}
       & \max_i\sigma_{\max}(\Sigma_{\theta^*}^i)\sigma_{\max}(\Sigma_a^i) \| \Sigma_a^{-1/2} X (\beta^*-\hat\beta) \|_2^2  \\
        & \leq c_5 \begin{cases}
           sq^2\log(p)\log^2(n) &, q>c_0m\\
           sm^2\log(p)\log^2(n) &, m>c_0q, \ p=q \\
           sm^3\log(p)\log^2(n) &, m>c_0q, \ p>q.
        \end{cases}
    \end{align*}
    Plugging in the bound into \eqref{vc.e.3.p1} and taking $t= c_6nm/\log(n)$, we have $\eqref{vc.e.3} \leq c_6nm/\log(n)$ with probability at least $1- c_1\exp\{-cn\} -c_2\exp\{-c\log(n)\} - c_3\exp\{-cmnq^{-\qm}\} - c_4 \exp\{-cn(m/q)^{\qm}\} - 2\exp\{- c \frac{n^2}{s\log^4(n)\log(p)} \left(\frac{m^2}{q^2}\right)^{\qm} m^{-\bm{1}\{ m>c_0q, p>q\}} \}$
    }
    
     For the term \eqref{vc.e.4}:
    {
    We can write
    \begin{align*}
        \sum_{i \in S_3} \Tr \left(Z^i \diag(\hat\psi - \psi^*) (Z^{i})^\top \right) & = \sum_{i \in S_3}\sum_{l=1}^q (\hat\psi_l - \psi_l^* ) \|Z_{l}^i \|_2^2 \\
        & \leq \|\psi -\psi^*\|_1 \max_{l=1, \ldots, q} \sum_{i \in S_3} \|Z_{ l}^i\|_2^2.
    \end{align*}
    Using similar arguments as those in \eqref{vc.e.z2}, we can show $\max_{l=1, \ldots, q} \sum_{i \in S_3} \|Z_{ l}^i\|_2^2 \leq c_1 \log(q) nm$ with probability at least $1- 2\exp\{-cnm\log(q)\}$. Then using Theorem~\ref{thm:Svc}, we have 
    \begin{align*}
        \eqref{vc.e.4} \leq s_{\psi} \sqrt{n} m\log(q) {\log(n)\log(p)\log(nmq)} m^{\bm{1}\{m>c_0q, p>q\}} (q/m)^{\qm}
    \end{align*}
    with probability at least
    $1 - c_1\exp\{-c\log(nq)\} -c_2\exp\{-cn\} -c_3\exp\{-c\log(n)\} - c_4\exp\{-cmnq^{-\qm}\} - c_5\exp\{-cn(m/q)^{\qm}\}  - c_6\exp\{-c\log(q)\} -c_7\exp\{-cnm\log(q)\}$.
    }

Therefore, plugging in the above bounds for \eqref{vc.e.1}--\eqref{vc.e.4}, under Assumption \ref{as.D}.\ref{as.D.4}, we obtain $|\hat\sigma_e^2 - \sigma_e^{2, *}| = o_p(1)$ with probability at least
\begin{align*}
1- & c_1\frac{s_\psi (m\vee q)\log^3(n)}{nm}  - c_2\exp\{-cnm\} - c_3\exp\{-cn\} -c_4\exp\{-c\log(n)\} - c_5\exp\{-cmnq^{-\qm}\}  \\
& - c_6 \exp\{-cn(m/q)^{\qm}\}
 - c_7\exp\left\{- c \frac{n^2}{s\log^4(n)\log(p)} \left(\frac{m^2}{q^2}\right)^{\qm} m^{-\bm{1}\{ m>c_0q, p>q\}} \right\}.
 \end{align*}

\end{proof}

\subsection{Proof of related lemmas for Theorem~\ref{thm:Svc} and Theorem~\ref{thm:Svc.e}}

\begin{proof}[Proof of Lemma \ref{lemma.D.1}]
$\left.\right.$

\textit{Lemma~\ref{lemma.D.1}.\ref{lemma.D.1.E1})}
{
$\left.\right.$

We can write
\begin{align*}
     E_{1,j} &= \sum_{i\in S_2} \Tr\left( A_j^i  \left(r_i r_i^\top -  \sum_{k=1}^{q} A_k^i  \psi_k^* \right) \right) \\
    & = \sum_{i\in S_2} r_i^\top  A^i_j  r_i - \sum_{i\in S_2}\Tr\left( A_j^i \sum_{k=1}^{q} A_k^i  \psi_k^*
    \right)
\end{align*}
Conditioning on the design matrices $Z^i$, we have that $r_i \mid Z^i \sim N(0, \Sigma^i_{\theta^*})$, and 
\begin{align*}
    \mathbb{E}\left(r_i^\top A_j^i r_i \mid Z^i \right) &  = \Tr(A_j^i \Sigma^i_{\theta^*}) \\
    & = \Tr\left( A_j^i \left(\sigma_e^{2, *} I_{m} + \sum_{k=1}^q \left( A_k^i + \left(\diag\left(Z_k^i\right)\right)^2\right) \psi_k^*\right)\right) \\
    & = \sum_{i \in S_2} \Tr\left( A_j^i \sum_{k=1}^{q} A_k^i \psi_k^*\right),
\end{align*}
where for the last equality we again use $\tr\left(A_j^i\diag(u)\right) =0$ for any vector $u\in R^m$. Then using the Hanson-Wright inequality \cite{rudelson2013hanson} and denoting $W_j  = \diag\left(\left\{\left(\Sigma_{\theta^*}^i \right)^{1/2} A_j^i \left(\Sigma_{\theta^*}^i \right)^{1/2}\right\}_{i\in S_2}\right)$, we have that
\begin{align}
    & \mathbb{P}\left(\max_{1\leq j\leq q}\left| E_{1,j} \right|  \geq t \mid Z \right) 
    \leq 2\exp\left\{\log(q) - c_1 \min \left\{\frac{t^2}{ \max_j\left\| W_j \right\|_F^2}, \frac{t}{\max_j\left\| W_j \right \|_2}\right\} \right\}. \label{pf.v.e1}
\end{align}

First, for the term $\|W_j \|_F^2$, we can show that
\begin{align}
    \| W_j \|_F^2 & = \tr\left(W_j^2\right) \nonumber \\
    & = \sum_{i \in S_2} \tr\left( \Sigma^{i}_{\theta^*} A^i_j  \Sigma^{i}_{\theta^*} A^i_j   \right) \nonumber\\
    & =  \sum_{i \in S_2} \tr\left( \sigma_e^{4,*} A_j^i A_j^i + 2\sigma_e^{2,*} Z^i \Psi (Z^i)^\top A_j^i A_j^i + Z^i\Psi (Z^i)^\top A_j^i  Z^i\Psi (Z^i)^\top A_j^i \right) \nonumber\\
    & = \sum_{i \in S_2}  \Tr\left( 
    \sigma_\epsilon^{4, *} Z_{j}^i (Z_{j}^{i})^\top  Z_{j}^i (Z_{ j}^{i})^\top - 
    \sigma_e^{4, *} \diag(Z_{j}^i)^2   Z_{j}^i (Z_{ j}^{i})^\top \right.\nonumber\\
    & \quad \quad \quad \left.  + 2 \sigma_e^{2, *} Z^i \Psi (Z^{i})^\top Z_{j}^i(Z_j^i)^\top  Z_{ j}^i (Z_j^i)^\top \right. \nonumber\\
    & \left. \quad \quad \quad + 2 \sigma_e^{2, *} Z^i \Psi (Z^{i})^\top \diag(Z^i_j)^4 \right. \nonumber\\
    & \left. \quad \quad \quad - 4 \sigma_e^{2, *} Z^i \Psi (Z^{i})^\top \diag(Z^i_j)^2 Z_{j}^i(Z_j^i)^\top   \right.\nonumber \\
    & \left. \quad \quad \quad +
    Z^i \Psi (Z^{i})^\top Z^i_j (Z^i_j)^\top Z^i \Psi (Z^{i})^\top Z^i_j (Z^i_j)^\top \right. \nonumber \\
    & \quad \quad \quad + \left. Z^i \Psi (Z^{i})^\top \diag(Z^i_j)^2 Z^i \Psi (Z^{i})^\top \diag(Z^i_j)^2 \right. \nonumber\\
    & \quad \quad \quad - 2 \left. Z^i \Psi (Z^{i})^\top Z^i_j (Z^i_j)^\top Z^i \Psi (Z^{i})^\top \diag(Z^i_j)^2 \right)\nonumber \\
    & \leq \left(\max_i \sigma^2_{\max}\left(Z^i \Psi (Z^i)^\top\right) + 2 \sigma_e^{2,*} \max_i \sigma_{\max}\left(Z^i \Psi (Z^i)^\top\right) + \sigma_e^{4,*}\right) \sum_{i \in S_2}  \|Z_{j}^i\|_2^4 \nonumber\\
    & \quad \quad + \left(3\max_i \sigma^2_{\max}\left(Z^i \Psi (Z^i)^\top\right) + 6 \sigma_e^{2,*} \max_i \sigma_{\max}\left(Z^i \Psi (Z^i)^\top\right) + \sigma_e^{4,*}\right) \sum_{i \in S_2}  \sum_{l=1}^m \left(\left(Z_{j}^i\right)_l\right)^4. \label{E1.e1}
\end{align}
Using Lemma~\ref{lemma:A.1}.\ref{lemma:A.1(4)} we can show that $\max_i \sigma_{\max}\left(Z^i \Psi (Z^i)^\top\right) \leq c_1(m\vee q)\log(n)$ with probability at least $1-2\exp\{-c_2(m\vee q)\log(n)\}$. Note that $\sum_{l=1}^m \left(\left(Z_{j}^i\right)_l\right)^4\leq \|Z_{j}^i\|_2^4$. Based on the distribution $Z^i_j \mid \Sigma_Z^i \sim N\left(0, \left(\Sigma_Z^i\right)_{j,j} I_m\right)$ and Assumption~\ref{as.A}.\ref{as.A.2} that $\left(\Sigma_Z^i\right)_{j,j} \asymp 1$, we can show that
\begin{align}
    \P\left( \max_j \max_i \left| \|Z^i_j\|_2^2 - c_3 m \right| \geq  t \mid \Sigma_Z^i \right) \leq 2\exp\left\{ \log(q) +\log(n_2) - c_4\min\left\{ \frac{t^2}{ 8m}, \frac{t}{8}\right\}\right\}. \label{vc.E1.z2}
\end{align}
Taking $t=c_5m \log(nq)$, we have $\max_{i,j} \|Z^i_j\|_2^2 \leq c_6 m\log(nq)$ with probability at least $1-2\exp\{-c_7m\log(nq)\}$. Thus, plugging in the bounds for $\max_{i,j} \|Z^i_j\|_2^2$ and $\max_i \sigma_{\max}\left(Z^i \Psi (Z^i)^\top\right)$ into \eqref{E1.e1}, we can show that with probability at least $1-2\exp\{-c(m\vee q)\log(n)\} - 2\exp\{-cm\log(nq)\}$, we have
\begin{align}
    \max_j\|W_j\|_F^2 \leq c(m^2 \vee q^2) \log^2(n) n m^2 \log^2(nq). \label{E1.wj.f.2}
\end{align}

Next, for the term $\| W_j \|_2$, we can write
\begin{align*}
   \max_j \| W_j \|_2 
    &  = \max_i \max_j\left\|\Sigma_{\theta^*}^i Z^i_j (Z^i_j)^\top - \Sigma_{\theta^*}^i \diag(Z^i_j)^2 \right\|_2 \\
    & \leq \max_i \max_j\|\Sigma_{\theta^*}^i\|_2  \|Z^i_j\|^2_2 + \max_i \max_j\| \Sigma_{\theta^*}^i\|_2 \left\|Z^i_j\right\|_\infty^2.
\end{align*}
Then by the normality of $Z^i_j$, we can write 
\begin{align}
\P\left(\max_i\max_j \left|\left\|Z^i_j\right\|_\infty^2 -\left(\Sigma_Z^i\right)_{j,j}\right| \geq t \mid \Sigma_Z^i \right) \leq 2\exp\{\log(m) +\log(n) +\log(q) - \min\{t^2/8, t/8\}\}, \label{vc.E1.z.inf}
\end{align}
which implies $\max_i\max_j \left\|Z^i_j\right\|_\infty^2 \leq c_1\log(nmq)$ with probability at least $1-2\exp\{-c_2 \log(nmq)\}$. Then using Lemma~\ref{lemma:A.1}.\ref{lemma:A.1(4)} to bound $\max_i \|\Sigma_{\theta^*}^i\|_2$ and inequality \eqref{vc.E1.z2} to bound $\max_i\max_j \|Z^i_j\|^2_2$, we have
\begin{align}
    \max_j\|W_j\|_2 & \leq c_3(m \vee q)\log(n) m \log(nq) + c_4 (m \vee q) \log(n) \log(nmq) \nonumber \\
    &\leq c_5 (m \vee q)\log(n) m \log(nmq) \label{E1.wj.2}
\end{align}
which holds with probability at least $1-2\exp\{-c(m\vee q)\log(n)\} - 2\exp\{-cm\log(nq)\} - 2\exp\{-c\log(nmq)\}$.

Plugging in the bounds in \eqref{E1.wj.f.2} and \eqref{E1.wj.2} into \eqref{pf.v.e1}, and taking $t= c_6 (m \vee q) m\sqrt{n} \log(n)\log(nmq)\log(q)$, we have 
\begin{align*}
    \max_j|E_{1, j}| \leq c_6(m \vee q) \log(n)\log(nmq)\log(q) m\sqrt{n}
\end{align*}
with probability at least $1-2\exp\{-c(m\vee q)\log(n)\} - 2\exp\{-cm\log(nq)\} - 2\exp\{-c\log(nmq)\} -2\exp\{-c\log(q)\}$.
}
\\

\textit{Lemma~\ref{lemma.D.1}.\ref{lemma.D.1.E2})}
{
$\left.\right.$

We can write 
\begin{align*}
     \max_j|E_{2,j}| & = \max_j \left|\sum_{i \in S_2} \Tr\left( A_j^i X^i(\beta^*-\hat\beta)(\beta^*-\hat\beta)^\top (X^i)^\top\right) \right|\\
     & \leq \max_j \left| \max_{i}\left(\sigma_{\max}\left(A_j^i \Sigma_a^i\right)\right) \|\Sigma_a^{-1/2}X(\beta^*-\hat\beta)\|_2^2  \right| \\
     & = \|\Sigma_a^{-1/2}X(\beta^*-\hat\beta)\|_2^2 \max_j\max_{i}\sigma_{\max}\left(\Sigma_a^i\right) \sigma_{\max}\left(Z_{j}^i \left(Z_{j}^{i}\right)^\top-\diag\left(Z_{j}^i\right)^2\right)   \\
    & \leq \|\Sigma_a^{-1/2}X(\beta^*-\hat\beta)\|_2^2 \max_i \sigma_{\max}(\Sigma_a^i)
    \left(\max_{i,j}\|Z^i_j\|_2^2 + \max_{i,j}\left\|Z^i_j\right\|_\infty^2 \right).
\end{align*}
Thus, using Theorem~\ref{thm:S1} to bound $\|\Sigma_a^{-1/2}X(\beta^*-\hat\beta)\|_2^2$, using Lemma~\ref{lemma:A.1}.\ref{lemma:A.1(4)} to bound $\sigma_{\max}(\Sigma_a^i)$, and using \eqref{vc.E1.z2} and \eqref{vc.E1.z.inf}, we have
\begin{align*}
   \max_j|E_{2, j}| \leq \begin{cases}
   c_1s\log(p)\log(n)\log(nq)mq &, q>c_0m \\
   c_1s\log(p)\log^3(n)\log(nq)m^2 &, q>c_0m \ \text{and assuming Assumption~\ref{as.A.add}.\ref{as.A.3}}\\
   c_1s\log(p)\log(n)\log(nq)m^2 &, m>c_0q,\ p=q \\
   c_1s\log(p)\log(n)\log(nq)m^3 &, m>c_0q,\ p>q,
   \end{cases}
\end{align*}
with probability at least  $1-4\exp\{-cn\} -12\exp\{-c\log(n)\} - 2\exp\{-cmnq^{-\qm}\} - \exp\{-cn(m/q)^{\qm}\} - 2\exp\{-cm\log(nq)\} -2\exp\{-c\log(nmq)\} -2\exp\{-c(m\vee q)\log(n)\}$.
}
\\

\textit{Lemma~\ref{lemma.D.1}.\ref{lemma.D.1.E3})}
{
$\left.\right.$

We can write 
\begin{align*}
     E_{3,j} 
    &  = \sum_{i \in S_2} \left( \left(\beta^*-\hat\beta\right)^\top (X^{i})^\top A_j^i \left(\Sigma_{\theta^*}^{i}\right)^{1/2}\right) \left(\Sigma_{\theta^*}^{i}\right)^{-1/2}r_i.  
\end{align*}
Conditioning on $X$ and $\hat\beta$, we have $\left(\Sigma_{\theta^*}^{i}\right)^{-1/2}r_i \mid X, \hat\beta \sim N(0, I_m)$. Thus,
\begin{align}
    & \mathbb{P}\left(\max_{1 \leq j \leq q}|E_{3,j}| \geq t|X,\hat\beta\right)  \leq 2\exp \left\{ \log(q) - \frac{t^2}{ 8 \max_j \sum_{i \in S_2} (\beta^*-\hat\beta)^\top (X^i)^\top  A_j^i  \Sigma_{\theta^*}^i  A_j^i  X^i(\beta^*-\hat\beta)}\right\}. \label{pf.v.lemma.1}
\end{align}
Then, with probability at least $1-4\exp\{-cn\} -12\exp\{-c\log(n)\} - 2\exp\{-cmnq^{-\qm}\} - \exp\{-cn(m/q)^{\qm}\} - 2\exp\{-cm\log(nq)\} -2\exp\{-c\log(nmq)\} - 2\exp\{-c(m\vee q)\log(n)\}$, we have
\begin{align}
   & \max_j \sum_{i \in S_2} (\beta^*-\hat\beta)^\top (X^i)^\top  A_j^i  \Sigma_{\theta^*}^i  A_j^i X^i(\beta^*-\hat\beta) \nonumber \\
   & \leq \|\Sigma_a^{-1/2} X(\beta^*-\hat\beta)\|_2^2 \max_{i,j} \sigma_{\max}\left(A^i_j \Sigma_{\theta^*}^i A^i_j \Sigma_a^i\right)\nonumber \\
   & \leq \|\Sigma_a^{-1/2} X(\beta^*-\hat\beta)\|_2^2 \max_{i,j} \sigma^2_{\max}\left(A^i_j\right) \sigma_{\max}\left(\Sigma_{\theta^*}^i\right)\sigma_{\max}\left(\Sigma_a^i\right) \nonumber \\
   & \leq c_1\|\Sigma_a^{-1/2} X(\beta^*-\hat\beta)\|_2^2  \left(\max_{i,j}\|Z^i_j\|_2^2 + \max_{i,j}\|Z^i_j\|^2_\infty\right)^2 \max_i\sigma_{\max}\left(\Sigma_{\theta^*}^i\right)\sigma_{\max}\left(\Sigma_a^i\right) \nonumber \\
   & \leq  
   c_2 \begin{cases}
   s\log(p)\log^2(n)\log^2(nq) m^2 q^2 &, q>c_0m \\
   s\log(p)\log^4(n)\log^2(nq) m^3 q &, q>c_0m \ \text{and assuming Assumption~\ref{as.A.add}.\ref{as.A.3}}\\
   s\log(p)\log^2(n)\log^2(nq) m^4 &, m>c_0q,\ p=q \\
   s\log(p)\log^2(n)\log^2(nq)m^5 &, m>c_0q,\ p>q,
   \end{cases} \label{vc.E3.1}
\end{align}
where the last inequalities \eqref{vc.E3.1} use Theorem~\ref{thm:S1}, Lemma~\ref{lemma:A.1}.\ref{lemma:A.1(4)}, and the inequalities \eqref{vc.E1.z2} and \eqref{vc.E1.z.inf}. Plugging \eqref{vc.E3.1} into \eqref{pf.v.lemma.1} and we can obtain
\begin{align*}
    \max_{j}|E_{3,j}| \leq 
    c_3 \begin{cases}
   \sqrt{s\log(p)\log(q)\log^2(n)\log^2(nq)m^2q^2} &, q>c_0m \\
   \sqrt{s\log(p)\log(q)\log^4(n)\log^2(nq){m^3}{q}} &, q>c_0m \ \text{and assuming Assumption~\ref{as.A.add}.\ref{as.A.3}}\\
   \sqrt{s\log(p)\log(q)\log^2(n)\log^2(nq)m^4} &, m>c_0q,\ p=q \\
   \sqrt{s\log(p)\log(q)\log^2(n)\log^2(nq)m^5} &, m>c_0q,\ p>q,
   \end{cases}
\end{align*}
with probability at least  $1-4\exp\{-cn\} -12\exp\{-c\log(n)\} - 2\exp\{-cmnq^{-\qm}\} - \exp\{-cn(m/q)^{\qm}\} - 2\exp\{-cm\log(nq)\} -2\exp\{-c\log(nmq)\} -2\exp\{-c\log(q)\} - 2\exp\{-c(m\vee q)\log(n)\}$.
}
\end{proof}

\begin{proof}[Proof of Lemma~\ref{lemma.D.2}]
{
$\left.\right.$

For simpler notation, we denote the $(j,k)$ entry of $\Sigma^i_Z$ by $\sigma_{i, j, k}$ for the rest of the proof. We denote the $l$th entry of the vector $Z^i_j$ by $Z^i_{l,j}$.

\textit{Lemma~\ref{lemma.D.2}.\ref{lemma.D.2.G1})}
{
$\left.\right.$

Defining matrix $H^i = (Z^{i})^\top Z^i$ for $i=1, \ldots, n$, we can write $H^i_{j,k} = (Z_{ j}^{i})^\top  Z^i_{k} =  \sum_{l=1}^{m} Z_{l, j}^i Z_{l, k}^i$. We will focus on the entry-wise concentration of the matrices $H^i$.

First, for the diagonal terms ${1 \leq j=k\leq q}$, we have $H^i_{j,j} =  \sum_{l=1}^{m}  \left(Z_{l, j}^{i}\right)^2$. Since $Z^i \mid \Sigma_Z^i \sim MN_{m\times q}(0, I_m, \Sigma_Z^i)$, we have
    $(Z^i_{l,j})^2 - \sigma_{i,j,j} \mid \Sigma_Z^i \in \SE(4\sigma^2_{i,j,j}, 4\sigma_{i,j,j})$, and thus $H^i_{j,j} - m \sigma_{i,j,j} \mid \Sigma_Z^i \in \SE(4m\sigma^2_{i,j,j}, 4\sigma_{i,j,j})$. Therefore, based on the tail bound of sub-exponential random variables,
  \begin{align*}
    \mathbb{P}&\left(\max_{i,j} \left|H_{j,j}^i - m \sigma_{i,j,j}\right|> t \right)  \leq 2\exp\left\{\log(nq)-\min\left\{\frac{t^2}{8m \sigma^2_{i,j,j}}, \frac{ t}{8{\sigma_{i,j,j}}}\right\}\right\}.
\end{align*}
    %Under Assumption~\ref{as.A}.\ref{as.A.2}, we have $\sigma_{i,j,j}\asymp 1$. 
    Taking $t = 16\sigma_{i,j,j} \sqrt{m} \log(nq)$, we obtain $\max_{i,j} \left|H_{j,j}^i - m \sigma_{i,j,j}\right| \leq 16\sigma_{i,j,j} \sqrt{m} \log(nq)$ with probability at least $1-2\exp\{-c\log(nq)\}$. \textcolor{black}{Under Assumption~\ref{as.D}.\ref{as.D.2}}, this implies that $\forall i,j$, %We can show that $\mathbb{E}\left((H^i_{j,j})^2\right) = (m^2 + 2m)\sigma_{i, j, j}^2$. Thus, with probability at least $1-2\exp\{-cm\log(nq)\}$, we have:
    \begin{align}
    & m^2 + 16^2m \log^2(nq) - 32 m^{3/2}\log(nq)  \leq \frac{1}{\sigma_{i,j,j}^2}(H_{j,j}^i)^2  \leq m^2 + 16^2m \log^2(nq) + 32 m^{3/2}\log(nq). \label{vc.G1.w1}
\end{align}

Next, for the off-diagonal terms ${1 \leq j \neq k\leq q}$, we have the fact that for any two normally distributed random variables $U$, $V$ with mean $0$, variance $1$ and correlation $\rho$,
\begin{align*}
 UV = \frac{(U+V)^2}{4} - \frac{(U-V)^2}{4} = \frac{1+\rho}{2} Q_1 - \frac{1-\rho}{2}Q_2,
\end{align*}
where $Q_1$ and $Q_2$ are independent and follow a $\chi^2_1$ distribution. Thus, the random variable $UV$ is sub-exponential with mean $\rho$, and hence $UV -\rho \in \SE(2\rho^2+2, 2+2|\rho|)$. We thus have
\begin{align*}
    & Z^i_{l,k}Z^i_{l,j} -\sigma_{i,j,k} \in \SE(2\sigma_{i,j,k}^2+2\sigma_{i,j,j}\sigma_{z,k,k}, 2\sqrt{\sigma_{i,j,j}\sigma_{i,k,k}}+2{|\sigma_{i,j,k}|})\\
    \Rightarrow & H^i_{j,k} -m \sigma_{i,j,k} \in \SE( 2m\sigma_{i,j,k}^2+2m\sigma_{i,j,j}\sigma_{i,k,k}, 2\sqrt{\sigma_{i,j,j}\sigma_{i,k,k}}+2{|\sigma_{i,j,k}|}).
\end{align*}
Denoting $\rho_{i,j,k} =\frac{\sigma_{i,j,k}}{\sqrt{\sigma_{i,j,j}\sigma_{i,k,k}}}$, based on the tail bound of sub-exponential random variables, we have that
    \begin{align*}
    &\mathbb{P}\left( \max_{i,j,k} \left|H^i_{j,k} - m \sigma_{i, j, k}\right| > t \right)\\
    & \leq 2\exp\left\{\log(q^2n)-\min\left\{
    \frac{t^2}{m \sigma_{i,j,j}\sigma_{i,k,k}\left(4\rho_{i,j,k}^2 + 4\right)}, \frac{ t}{\sqrt{\sigma_{i,j,j}\sigma_{i,k,k}}\left(4+4\left|\rho_{i,j,k}\right| \right)}\right\}\right\}.
\end{align*}
Thus, taking $t = \sqrt{8 m \sigma_{i,j,j}\sigma_{i,k,k}\left(|\rho_{i,j,k}| + 1\right)} \log(nq^2)$, with probability at least $1-2\exp\{-c\log(nq^2)\}$ we have
\begin{align}
    \max_{i,j,k} \left|H^i_{j,k} - m \sigma_{i, j, k}\right| \leq \sqrt{8 m \sigma_{i,j,j}\sigma_{i,k,k}\left(|\rho_{i,j,k}| + 1\right)} \log(nq^2). \label{vc.G1.1}
\end{align}

To study the lower and upper bounds of $|H^i_{j,k}|^2$ based on \eqref{vc.G1.1}, we consider two cases:

\begin{enumerate}
    \item If for given $i, j, k$, $m|\sigma_{i, j,k}| \gg  \sqrt{ \sigma_{i,k,k}\sigma_{i,j,j}(|\rho_{j,k}| + 1) m} \log(nq^2)$, i.e., $\frac{|\rho_{i,j,k}|+1}{\rho^2_{i,j,k}} \ll \frac{m}{\log^2(nq^2)}$:
The correlation $|\rho_{i,j,k}|$ is not too small, and \eqref{vc.G1.1} implies that $H^i_{j,k}$ is bounded away from zero with high probability. Then with probability at least $1-2\exp\{ - c\log(nq^2)\}$, we have that 
\begin{align}
\frac{(H^i_{j,k})^2}{\sigma_{z, j, j}\sigma_{z, k, k}} 
    & \leq m^2 \rho_{i,j,k}^2 + 8m(|\rho_{i,j,k}|+1)\log^2(nq^2) + 2 m|\rho_{i,j,k}|\sqrt{8 m (|\rho_{i,j,k}|+1)} \log(nq^2) \nonumber \\
    & \leq m^2 \rho_{i,j,k}^2 + 16 m \log^2(nq^2) + 8 m|\rho_{i,j,k}|\sqrt{m} \log(nq^2), \label{vc.G1.w2} \\
\frac{(H^i_{j,k})^2}{\sigma_{z, j, j}\sigma_{z, k, k}} & \geq  m^2 \rho_{i,j,k}^2 + 8m(|\rho_{i,j,k}|+1)\log^2(nq^2) - 2 m|\rho_{i,j,k}|\sqrt{8 m (|\rho_{i,j,k}|+1)} \log(nq^2) \nonumber \\    
    & \geq m^2 \rho_{i,j,k}^2 + 8 m\log^2(nq^2) - 8 m|\rho_{i,j,k}|\sqrt{m} \log(nq^2). \label{vc.G1.w3}
\end{align}
Note that the condition $\frac{|\rho_{i,j,k}|+1}{\rho^2_{i,j,k}} \ll \frac{m}{\log^2(nq^2)}$ implies $\rho_{i,j,k}^2 \gg \frac{\log^2(nq^2)}{m}$, which then implies 
\begin{align}
    m^{3/2} |\rho_{i,j,k}| \log(nq^2) \gg m\log^2(nq^2). \label{vc.G1.tmp1}
\end{align}

\item If for given $i, j, k$, $m|\sigma_{i,j,k}| = O  \left(\sqrt{\sigma_{i,k,k}\sigma_{i,j,j}( |\rho_{i,j,k}|+1)m} \log(nq^2)\right)$, i.e., $\frac{\rho^2_{i,j,k}}{|\rho_{i,j,k}| +1}= O \left(\frac{\log^2(nq^2)}{m}\right)$:
The correlation $\rho_{i,j,k}$ is very small under Assumption~\ref{as.D}.\ref{as.D.2}, and \eqref{vc.G1.1} implies that $H^i_{j,k}$ is not bounded away from zero. Then with probability at least $1-2\exp\{- c\log(nq^2)\}$, we have 
\begin{align}
    0 & \leq \frac{(H^i_{j,k})^2}{\sigma_{i, j, j}\sigma_{i, k, k}}  \leq  m^2 \rho_{j,k}^2 + 16 m \log^2(nq^2) + 8m |\rho_{i,j,k}|\sqrt{m} \log(nq^2). \label{vc.G1.w4}
\end{align}
Note that the condition $\frac{\rho^2_{i,j,k}}{|\rho_{i,j,k}| +1}= O \left(\frac{\log^2(nq^2)}{m}\right)$ implies $\rho^2_{i,j,k} \leq c \log^2(nq^2)/m$ for some constant $c>0$, which then implies 
\begin{align}
    m^{3/2} |\rho_{i,j,k}| \log(nq^2) \leq c_1 m\log^2(nq^2) \label{vc.G1.tmp2}
\end{align}
for some constant $c_1>0$.

\end{enumerate}

Note that for $v \in \R^q$, we can write
\begin{align*}
 v^\top \left(G^i_1 - \E\left(G^i_1\right)\right) v & =   v^\top \left(H^i \circ H^i- \mathbb{E}\left(H^i \circ H^i\right)  \right) v  \leq \sum_{j, k =1}^q |v_j| |v_k| \left| \left(H^i_{j,k}\right)^2 - \mathbb{E}\left(\left(H^i_{j,k}\right)^2\right) \right|  \leq \|v\|_2^2 \|W^i\|_2 \\
     v^\top \left(G^i_1 - \E\left(G^i_1\right)\right) v & \geq  - \sum_{j, k =1}^q |v_j| |v_k| \left| \left(H^i_{j,k}\right)^2 - \mathbb{E}\left(\left(H^i_{j,k}\right)^2\right) \right| \geq - \|v\|_2^2 \|W^i\|_2
\end{align*}
where we define the matrix $W^i$ such that $ W^i_{j,k} = \left| \left(H^i_{j,k}\right)^2 - \mathbb{E}\left(\left(H^i_{j,k}\right)^2\right) \right|$. We compute the values of $\E\left(\left(H^i_{j,k}\right)^2\right)$ based on the distribution $Z^i \mid \Sigma_Z^i \sim MN_{m\times q}(0, I_m, \Sigma_Z^i)$:
\begin{align*}
    \E\left(\left(H^i_{j,k}\right)^2\right) = & \begin{cases}
       (m^2+2m)\sigma^2_{i,j, j} &, j=k\\
       (m^2 +m) \sigma_{i,j,k}^2 + m\sigma_{i,j,j}\sigma_{i,k,k} &, j\neq k.
    \end{cases}
\end{align*}
Thus, based on \eqref{vc.G1.w1}--\eqref{vc.G1.tmp2}, with probability at least $1- 2\exp\{-c\log(nq)\} - 2\exp\{-c\log(nq^2)\}$, for a given $i$ we have
\begin{align*}
    W^i_{j,k} 
    & \leq \begin{cases}
    % 0, \quad j=k=0;\\
    c_2m^{3/2}\log(nq)& , \quad  1\leq j=k\leq q;\\
    % \alpha_0^2\max_i(m_i)\sqrt{n\log(q)}, \quad j=0,\ 1\leq k \leq q,\quad or \quad  k=0,\ 1\leq j \leq q \\
     c_3 m^{3/2} |\rho_{i,j,k}|\log(nq^2)& , \quad  1 \leq j \neq k \leq q, \ \text{and } \frac{\rho_{i,j,k}^2}{|\rho_{i,j,k}|+1} \gg \frac{\log^2(nq^2)}{m} \\
     c_4 m\log^2(nq^2) & , \quad 1 \leq j\neq k \leq q, \ \text{and } \frac{\rho_{i,j,k}^2}{|\rho_{i,j,k}|+1} = O\left( \frac{\log^2(nq^2)}{m} \right)\\
    \end{cases}.
\end{align*}
Using Gershgorin circle theorem \cite{horn2012matrix}, we can obtain the following bounds for the eigenvalues of the matrices $W^i$ with probability at least $1- 2\exp\{-c\log(nq)\} - 2\exp\{-c\log(nq^2)\}$: 
\begin{align*}
    \max_i|\sigma(W^i)| & \leq \max_{i,j}\left(|W^i_{j,j}|+\sum_{k=1,k\neq j}^{q}|W^i_{j,k}|\right) \\
    & \leq
 \max_i \left(c_5m^{3/2} \log(nq^2) + c_5s^i_Z m^{3/2} \log(nq^2)  + c_5 m (q-s^i_Z)\log^2(nq^2)\right) \\
 & \leq c_5m^{3/2} \log(nq^2) + c_5s_Z m^{3/2} \log(nq^2)  + c_5 m q\log^2(nq^2),
\end{align*}
where $s^i_Z$ and $s_Z$ are defined in equation (20). %\ref{sdef:siZ}.
Thus, with probability at least $1- 2\exp\{-c\log(nq)\} - 2\exp\{-c\log(nq^2)\}$, we have $\left\|G^i_1 - \E\left(G^i_1\right)\right\|_2 \leq c_5m^{3/2} \log(nq^2) +c_5 s_Z m^{3/2} \log(nq^2)  + c_5 m q\log^2(nq^2)$.
}
\\

\textit{Lemma~\ref{lemma.D.2}.\ref{lemma.D.2.G2})}
{
$\left.\right.$

The matrix $Z^i \circ Z^i$ has independent rows, and its entries follow scaled $\chi^2_1$ distributions. Thus, by Theorem 5.44 (random matrices with heavy-tailed non-isotropic independent rows) in \cite{vershynin2010introduction}, with probability at least $1-\exp\{\log(nq) - ct^2\}$ we have 
    \begin{align*}
         \|Z^i\circ Z^i \|_2 & \leq \|2\Sigma_Z^i \circ \Sigma_Z^i + u^i_Z (u^i_Z)^\top \|_2^{1/2} \sqrt{m} + t\sqrt{m}\\
         & \leq \left(\|2\Sigma^i_Z\circ\Sigma^i_Z\|_2^{1/2} + \|{u}^i_Z\|_2\right)\sqrt{m} + t\sqrt{m},
     \end{align*}
     where ${u^i_Z} = \left( \left(\Sigma^i_Z\right)_{1, 1}, \dots, \left(\Sigma^i_Z\right)_{q, q} \right)^\top$. Note that under Assumption~\ref{as.A}.\ref{as.A.2}, we have $\|\Sigma^i_Z\circ\Sigma^i_Z\|_2 \leq \|\Sigma_Z^i\|_2^2 \asymp 1$ \cite{schacke2004kronecker, johnson1981eigenvalue}, and $\|u^i_Z\|_2 \asymp \sqrt{q}$. Thus, taking $t=c_1\sqrt{q \log(n)}$, with probability at least $1-\exp\{- c q\log(n) \}$ we have
     \begin{align}
         \|Z^i\circ Z^i \|_2 \leq c_2 \sqrt{mq\log(n)}. \label{vc.G2.tmp1}
     \end{align}
     
     Since $Z^i \mid \Sigma_Z^i \sim MN_{m \times q}(0, I_m, \Sigma_Z^i)$, we have $\mathbb{E}\left(G_2^i\right) = 2m \Sigma_Z^i \circ\Sigma_Z^i + m u^i_Z (u^i_Z)^\top$, which gives 
     \begin{align}
         \left\|\mathbb{E}\left(G_2^i\right) \right\|_2 \leq 2m\|\Sigma_Z^i\|^2_2 + m\| u^i_Z\|_2^2 \leq cmq. \label{vc.G2.tmp2}
     \end{align}
     
     Thus, by \eqref{vc.G2.tmp1} and \eqref{vc.G2.tmp2}, we have $ \|G_2^i - \mathbb{E}(G_2^i) \|_2^2 \leq \|Z^i\circ Z^i \|_2^2 + \|\mathbb{E}(G_2^i)\|_2 \leq c_3 mq\log(n)$ with probability at least $1-\exp\{- c q\log(n) \}$. 
}

}
\end{proof}

\begin{proof}[Proof of Lemma~\ref{lemma:RE_for_B}]
$\left.\right.$
Recalling the definition of $B_{j,k} = \sum_{i \in S_2} \Tr\left(A_j^iA_k^i\right)$ in (19), % \eqref{def.B}, 
for a fixed vector $v\in \R^q$, we can write
\begin{align}
v^\top B v & = \sum_{i \in S_2} \sum_{j,k=1}^q \Tr\left( \left(Z_{j}^i (Z_{j}^i)^\top - \diag(Z_{j}^i)^2 \right) \left(Z_{k}^i (Z_{k}^i)^\top  - \diag(Z_{k}^i)^2 \right) \right) v_jv_k  \nonumber\\
& = \sum_{i \in S_2} \sum_{j,k=1}^q \Tr\left( Z_{j}^i (Z_{j}^{i})^\top   Z_{k}^i (Z_{ k}^{i})^\top  \right) v_jv_k - \Tr\left( Z_{j}^i (Z_{j}^{i})^\top \diag(Z_{ k}^i)^2 \right) v_jv_k  \nonumber\\
& = \sum_{i \in S_2} v^\top \left( (Z^i)^\top Z^i \right) \circ \left( (Z^i)^\top Z^i \right) v - v^\top \left(Z^{i} \circ Z^i \right)^\top \left(Z^{i} \circ Z^i \right) v. \label{pf.B.RE.1}
\end{align}
Then, recalling the definitions of $G_1^i = \left((Z^i)^\top Z^i \right) \circ \left((Z^i)^\top Z^i \right)$, $G_2^i = \left(Z^{i} \circ Z^i \right)^\top \left(Z^{i} \circ Z^i \right)$ in Lemma~\ref{lemma.D.2}, we can write \eqref{pf.B.RE.1} as
\begin{align}
    v^\top B v =  v^\top \left( \sum_{i \in S_2} \left(G_1^i - \mathbb{E}\left(G_1^i\right)\right) - \sum_{i \in S_2} \left(G_2^i - \mathbb{E}\left(G_2^i\right)\right) + \sum_{i \in S_2} \left(\mathbb{E}\left(G_1^i\right) - \mathbb{E}\left(G_2^i\right)\right) \right) v. \label{pf.B.RE.1.1}
\end{align}

We study each of the terms in the parenthesis in \eqref{pf.B.RE.1.1} separately.

First, since $Z^i \mid \Sigma_Z^i \sim MN_{m\times q}(0, I_m, \Sigma_Z^i)$, we have $\mathbb{E}\left(G^i_1\right) - \mathbb{E}\left(G^i_2\right) = m(m-1)\left(\Sigma_Z^i\circ\Sigma_Z^i\right)$. Since we know that for two matrices $A_1$ and $A_2$, $A_1 \circ A_2$ is a principle submatrix of the Kronecker product $A_1 \otimes A_2$, we can show that $\sigma_{\min}(A_1)\sigma_{\min}(A_2) \leq \sigma_{\min}\left(A_1 \otimes A_2\right) \leq \sigma_{\min}\left(A_1 \circ A_2\right)$ \cite{schacke2004kronecker, johnson1981eigenvalue}. Thus, since $\sigma(\Sigma_Z^i)\asymp 1$ by Assumption~\ref{as.A}.\ref{as.A.2}, we have 
 \begin{align}
     \sigma_{\min}\left(\sum_{i \in S_2} \mathbb{E}\left(G^i_1\right) - \mathbb{E}\left(G^i_2\right) \right) \geq c_1 n m^2. \label{GG.bound}
 \end{align}
 
Next, for the term $\sum_{i \in S_2} \left(G_1^i - \mathbb{E}\left(G_1^i \right)\right)$, using Lemma~\ref{lemma.D.2}.\ref{lemma.D.2.G1}, we have $\max_i\|G_1^i - \mathbb{E}\left(G_1^i \right)\|_2 \leq c_1 m^{3/2} \log(nq^2) + c_1s_Z m^{3/2} \log(nq^2)  + c_1 m q\log^2(nq^2)$ with probability at least $1- 2\exp\{-c\log(nq)\} - 2\exp\{-c\log(nq^2)\}$. Then, by matrix Bernstein inequality \cite{tropp2015introduction}, we get 
    \begin{align}
        \mathbb{P}\left( \left\|\sum_{i \in S_2} G_1^i - \mathbb{E}\left(G_1^i \right) \right\|_2 \geq t \right) \leq \exp\left\{\log(2q) - \frac{t^2}{2} \frac{1}{\nu_{1} + c_2\left(s_Z m^{3/2} \log(nq^2)  + m q\log^2(nq^2)\right)  t}\right\}, \label{G1.final}
    \end{align}
    where $\nu_1 = n_2 \left\|\mathbb{E}(G_1^i (G_1^{i})^\top) - \mathbb{E}(G_1^i)\mathbb{E}(G_1^i)^\top\right\|_2$. Denote the $(j,k)$ entry of $\Sigma_Z^i$ by $\sigma_{i,j,k}$. Based on $Z^i \mid \Sigma_Z^i \sim MN_{m\times q}(0, I_m, \Sigma_Z^i)$, with some careful calculations, we can get
     \begin{align*}
          \left(\mathbb{E}(G_1^i G_1^{i,\top}) - \mathbb{E}(G_1^i)\mathbb{E}(G_1^i)^\top\right)_{j,j} & = \sum_{l=1}^q \left( 2m(m+3) \sigma_{i,j,j}^2\sigma_{i,l,l}^2  + 4m(m^2+7m+9)\sigma_{i,j,j}\sigma_{i,l,l}\sigma_{i,j,l}^2 \right. \\
         & \quad \quad + \left. 2(2m^2+5m+3)m\sigma_{i,j,l}^4\right) \\
          \left(\mathbb{E}(G_1^i G_1^{i,\top}) - \mathbb{E}(G_1^i)\mathbb{E}(G_1^i)^\top\right)_{j,k} & = \sum_{l=1}^q \left( m(m+2)(m+3) 4 \sigma_{i,j,k}\sigma_{i,j,l}\sigma_{i,k,l}\sigma_{i,l,l} \right. \\
          & \quad \quad + 2m(2m+3)\left(\sigma_{i,j,l}^2 \sigma_{i,k,k}\sigma_{i,l,l} + \sigma_{i,j,j}\sigma_{i,k,l}^2\sigma_{i,l,l}\right) \\
         & \quad \quad + 2m(m+1)(2m+3)\sigma_{i,j,l}^2\sigma_{i, k,l}^2  + 2m(m+2)\sigma_{i, j,k}^2 \sigma_{i,l,l}^2 \\
         & \quad \quad + \left. 2m \sigma_{i, j, j}\sigma_{i, k, k}\sigma_{i, l,l}^2 \right) 
     \end{align*}
     Then, using Gershgorin circle theorem \cite{horn2012matrix}, and under Assumption~\ref{as.A}.\ref{as.A.2} which implies $\sigma_{i,j,k} = O(1)$, we can bound the maximum eigenvalue of $\mathbb{E}(G_1^i G_1^{i,\top}) - \mathbb{E}(G_1^i)\mathbb{E}(G_1^i)^\top$ by 
     \begin{align}
         & \left\|\mathbb{E}(G_1^i G_1^{i,\top}) - \mathbb{E}(G_1^i)\mathbb{E}(G_1^i)^\top\right\|_2 \nonumber \\
         & \leq \max_j \left(\left| \mathbb{E}(G_1^i G_1^{i,\top}) - \mathbb{E}(G_1^i)\mathbb{E}(G_1^i)^\top\right|_{j,j} + \sum_{k=1, k\neq j}^q \left|\mathbb{E}(G_1^i G_1^{i,\top}) - \mathbb{E}(G_1^i)\mathbb{E}(G_1^i)^\top\right|_{j,k}\right) \nonumber \\
         & \leq c_1 \max_j \left(m^3 \left( \sum_{l=1}^q \sigma^2_{i,j,l} + \sum_{k,l=1}^q|\sigma_{i,k,l}| \right) + qm^2 \left(2 + \sum_{l=1}^q \sigma_{i,j,l}^2\right) + m^2 \sum_{k,l=1}^q \sigma_{i,k,l}^2 \ \right) \nonumber \\
         & \leq c_2 m^3 q^{3/2} \label{G1.circle}
     \end{align}
     where the last inequality follows from $\sum_{k=1}^q \sigma_{i,k,l}^2 \leq c_3 \sum_{k=1}^q |\sigma_{i,k,l}| \leq c_3\|\Sigma_Z^i\|_1 \leq c_3\sqrt{q} \|\Sigma_Z^i\|_2$, with matrix 1-norm defined by $\|A\|_1 = \max_{j} \sum_{k=1}^q |A_{j,k}|$ for matrix $A\in \R^{q\times q}$.

     Therefore, taking $t = c_4 nm^2 /\log(n)$ in \eqref{G1.final} for some suitably large constant $c_4>0$, under Assumption~\ref{as.D}.\ref{as.D.3}, we have
     \begin{align}
         \left\|\sum_{i \in S_2} \left(G_1^i - \mathbb{E}(G_1^i)\right) \right\|_2 \leq c_5 nm^2 /\log(n) \label{G1.bound}
     \end{align}
     with probability at least $1-\exp\{-c\log(q)\} - 2\exp\{-c\log(nq)\}$.
     
Finally, for the term $\sum_{i \in S_2} \left(G_2^i - \mathbb{E}\left(G_2^i\right)\right)$, using Lemma~\ref{lemma.D.2}.\ref{lemma.D.2.G2}, with probability at least $1-\exp\{-cq\log(n)\}$ we have $\left\|G_2^i - \mathbb{E}\left(G_2^i\right)\right\|_2 \leq  c_1mq\log(n)$. Then by matrix Bernstein inequality \cite{tropp2015introduction}, 
     \begin{align}
         \mathbb{P}\left(\left\|\sum_{i \in S_2} G_2^i - \mathbb{E}\left(G_2^i\right) \right\|_2 \geq t \right) \leq \exp \left\{\log(2q) - \frac{t^2}{2}\frac{1}{\nu_2 + c_2mq\log(n)t} \right\}, \label{G2.p}
     \end{align}
     where $\nu_2 = n_2\left\|\mathbb{E}\left(G^i_2 (G^i_2)^\top  \right) - \mathbb{E}\left(G^i_2\right)\mathbb{E}\left(G^i_2 \right)^\top \right\|_2$. Based on $Z^i \mid \Sigma_Z^i \sim MN_{m\times q}(0, I_m, \Sigma_Z^i)$, with some careful calculation, we can get 
     \begin{align*}
         \left( \mathbb{E}\left(G^i_2 (G^{i}_2)^\top \right) - \mathbb{E}\left(G^i_2\right)\mathbb{E}\left(G^i_2\right)^\top \right)_{j,j} & = \sum_{l=1}^q m\left(20\sigma_{i,j,l}^4 + 8 \sigma_{i,j,j}^2\sigma_{i,l,l}^2 + 68\sigma_{i,j,j}\sigma_{i,j,l}^2\sigma_{i,l,l}\right) = O_p(q m)\\
         \left( \mathbb{E}\left(G^i_2 (G^{i}_2)^\top \right) - \mathbb{E}\left(G^i_2\right)\mathbb{E}\left(G^i_2\right)^\top \right)_{j,k} &  = \sum_{l=1}^q m \left(48 \sigma_{i, j, k}\sigma_{i, j,l}\sigma_{i, k,l}\sigma_{i, l,l}  + 20 \sigma_{i, j,l}^2\sigma_{i, k,l}^2 + 10 \sigma_{i, j,l}^2\sigma_{i,k,k}\sigma_{i,l,l} \right.\\
         & \quad \quad \left. + 6 \sigma_{i,j,k}^2\sigma_{i,l,l}^2 + 2 \sigma_{i,j,j}\sigma_{i, k ,k}\sigma_{i,l,l}^2 + 10\sigma_{i, j,j}\sigma_{i, l, l}\sigma_{i,k,l}^2\right)\\
         & = O_p(qm).
     \end{align*}
     Then by Gershgorin circle theorem, we can follow the similar arguments as those in \eqref{G1.circle} to obtain $\nu_2 \leq c_3 nmq^2$. Thus, taking $t=c_4nm^2/\log(n)$ in \eqref{G2.p}, under Assumption~\ref{as.D}.\ref{as.D.3} we have 
     \begin{align}
         \left\|\sum_{i \in S_2} G_2^i - \mathbb{E}\left(G_2^i\right) \right\|_2 \leq c_4 nm^2/\log(n) \label{G2.bound}
     \end{align}
     with probability at least $1-\exp\{-c\log(q)\} - \exp\{-cq\log(n)\}$.

Plugging the bounds \eqref{GG.bound}, \eqref{G1.bound}, and \eqref{G2.bound} into \eqref{pf.B.RE.1.1}, we obtain 
\begin{align*}
    v^\top B v & \geq \|v\|_2^2 \left(\sigma_{\min}\left(\sum_{i \in S_2} \mathbb{E}\left(G^i_1\right) - \mathbb{E}\left(G^i_2\right) \right) - \left\| \sum_{i \in S_2} \left(G_1^i - \mathbb{E}\left(G^i_1\right)\right) \right\|_2- \left\| \sum_{i \in S_2} \left(G_2^i - \mathbb{E}\left(G^i_2\right)\right) \right\|_2 \right)\\
    & \geq c_5 nm^2 \|v\|_2^2
\end{align*} 
with probability at least $1-\exp\{-c\log(q)\} -2\exp\{-c\log(nq)\} - \exp\{-cq\log(n)\}$.
\end{proof}

\setcounter{table}{0}
\setcounter{figure}{0}
\renewcommand{\thetable}{S\arabic{table}}
\renewcommand{\thefigure}{S\arabic{figure}}

\newpage

\section{Extension to High-Dimensional Heterogeneous VAR models}
\label{S:VAR}

\begin{lemma}
\label{Slemma.a0}
Suppose $X\in \R^{T\times p}$ ($T\neq p$) is a Gaussian matrix with $\vec(X) \sim \N(0, \Xi)$. Define $Z\in \R^{T\times p}$ such that $\vec(Z) = \left(\Xi\right)^{-1/2}\vec(X) \sim \N(0, I_{Tp})$. We have that
\begin{align*}
    \sqrt{\sigma_{\min}(\Xi)} \sigma_{\min}(Z) \leq   \sigma(X) \leq  \sqrt{\sigma_{\max}(\Xi)} \sigma_{\max}(Z).
\end{align*}
We also have
\begin{align*}
    & X^\top (aXX^\top + I)^{-1} X \succ \sigma_{\min}(\Xi) Z^\top (a\sigma_{\max}(\Xi) ZZ^\top + I )^{-1}Z \\
    & X^\top (aXX^\top + I)^{-1} X \prec \sigma_{\max}(\Xi) Z^\top (a\sigma_{\min}(\Xi) ZZ^\top + I )^{-1}Z.
\end{align*}
\end{lemma}

\begin{assumption}
\label{as.VAR.a1}
    For the $i$th subject, conditioning on $\Gamma^i$, the observations $\{Y^i(t)\}_{t=1}^T$ are realizations of a stationary Gaussian process.
\end{assumption}

\begin{proof}[Proof for Lemma~\ref{Slemma.a0}]
We first work on the case when $T>p$:

Since the set of singular values $\{\sigma(X)\}$ is identical to the set $\left\{\sqrt{\sigma(X^\top X)}\right\}$, we have $\min_{\nu\in\R^p}\|X\nu\|_2^2 \leq \sigma^2_{\min}(X) \leq \sigma^2_{\max}(X) \leq \max_{\nu\in\R^p}\|X\nu\|_2^2$ for $\|\nu\|_2^2=1$. We can also show that:
\begin{align*}
    \|X\nu\|_2^2 & = \left\| \left(\nu^\top \otimes I_T \right) \vec(X) \right\|_2^2 \\
    & = \left\| \left(\nu^\top \otimes I_T \right) \Xi^{1/2} \vec(Z) \right\|_2^2\\
    & \in \left[ \sigma_{\min}(\Xi) \left\| \left(\nu^\top \otimes I_T \right) \vec(Z) \right\|_2^2, \sigma_{\max}(\Xi)\left\| \left(\nu^\top \otimes I_T \right) \vec(Z) \right\|_2^2 \right]
\end{align*}
Thus with $\left\| \left(\nu^\top \otimes I_T \right) \vec(Z) \right\|_2^2 = \|Z\nu\|_2^2 \in [\sigma^2_{\min}(Z), \sigma^2_{\max}(Z)]$, we obtain 
\begin{align*}
    \sigma_{\min}(\Xi)\sigma^2_{\min}(Z) \leq \sigma^2_{\min}(X) \leq \sigma^2_{\max}(X) \leq \sigma_{\max}(\Xi)\sigma^2_{\max}(Z).
\end{align*}

We next look at the case when $T<p$. Note that we now have $\{\sigma(X)\} = \{\sigma(X^\top)\} = \left\{\sqrt{\sigma(XX^\top)}\right\}$. Since the covariance matrix $\Var(\vec(X^\top))$ can be obtained by imposing the same permutations on the columns and the rows of the matrix $\Xi =\Var(\vec(X))$, the two covariance matrices are similar and have the same set of singular values. Therefore, we can just follow the same arguments used for the case of $T>p$ to establish the bounds for $\sigma(X)$ under the setting of $T<p$.

Based on the above bounds for $\sigma(X)$, we can get $XX^\top \succ \sigma_{\min}(\Xi) ZZ^\top$ since 
\begin{align*}
    \forall \nu\in {\R}^T, \quad  & \nu^\top XX^\top \nu - \nu^\top \sigma_{\min}(\Xi) ZZ^\top \nu \\
    & = \|(\nu^\top \otimes I_p) \vec(X^\top)\|_2^2 - \sigma_{\min}(\Xi) \|(\nu^\top \otimes I_p) \vec(Z^\top)\|_2^2 \\
    & = \|(\nu^\top \otimes I_p) \Xi^{1/2} \vec(Z^\top)\|_2^2 - \sigma_{\min}(\Xi) \|(\nu^\top \otimes I_p) \vec(Z^\top)\|_2^2 \\
    & \geq 0.
\end{align*}
We can similarly show that $XX^\top \prec \sigma_{\max}(\Xi) ZZ^\top$. Given two positive definite matrices $A$ and $B$, if $A \succ B$ then $B^{-1} \succ A^{-1}$. We thus have that
\begin{align}
\label{lemma.a0.1}
 (a\sigma_{\max}(\Xi) ZZ^\top + I_T)^{-1} \prec ( aXX^\top + I_T)^{-1} \prec (a\sigma_{\min}(\Xi) ZZ^\top + I_T)^{-1}.
\end{align}

We then show that for a positive definite matrix $A \in \R^{T\times T}$, $\sigma_{\min}(\Xi) Z^\top A Z \prec X^\top A X \prec \sigma_{\max}(\Xi) Z^\top A Z$: for the upper bound of $X^\top A X$, we have that
\begin{align*}
    \forall \nu \in {\R}^{T}, \quad & \nu^\top \sigma_{\max}(\Xi) Z^\top A Z \nu - \nu^\top X^\top A X \nu \\
    & = \sigma_{\max}(\Xi) \|A^{1/2} (\nu^\top \otimes I_T) \vec(Z) \|_2^2 - \|A^{1/2} (\nu^\top \otimes I_T) \Xi^{1/2} \vec(Z) \|_2^2\\
    & \geq 0.
\end{align*}
We can follow similar arguments to obtain the lower bound for $X^\top A X$.

Therefore, combining the bounds $\sigma_{\min}(\Xi) Z^\top A Z \prec X^\top A X \prec \sigma_{\max}(\Xi) Z^\top A Z$ and the bounds in \eqref{lemma.a0.1}, we obtain
\begin{align*}
 & X^\top (aXX^\top + I)^{-1} X \succ \sigma_{\min}(\Xi) Z^\top (a\sigma_{\max}(\Xi) ZZ^\top + I )^{-1}Z \\
    & X^\top (aXX^\top + I)^{-1} X \prec \sigma_{\max}(\Xi) Z^\top (a\sigma_{\min}(\Xi) ZZ^\top + I )^{-1}Z.
\end{align*}

\end{proof}

\newpage
\bibliographystyle{abbrv}
\bibliography{references.bib}

\end{document}
